# Supplementary material for: Current status and desired accuracy of the isotopic production cross-sections relevant to astrophysics of cosmic rays II. Fluorine to Silicon (and updated LiBeB)
Source: arXiv:2307.06798 source file (2024-06-09)
Supplement: Supplementary file 1 [file Supplementary_Material.pdf]

# Supplemental Material
# for "Current status and desired accuracy of the isotopic production cross-sections relevant to astrophysics of cosmic rays II. Fluorine to Silicon (and updated LiBeB)"

Yoann Génolini, David Maurin, Igor V. Moskalenko, Michael Unger
(Dated: November 23, 2023)

## PLOTS FOR PRODUCTION CROSS SECTIONS OF THE MOST IMPORTANT REACTIONS WITH PROTONS

In this Supplemental Material, we show the plots of the most important reaction channels discussed in the paper. For each shown reaction, all existing data above $\approx 100$ MeV/nucleon are plotted together with the three parametrizations discussed in the paper Sect. II.2, (GP12, GP12up22, GP22); only reactions with hydrogen target are presented. Measurements with He target (or He as a beam) are significantly more complicated to perform and the data are scarce, so we do not show them. We display, sorted by growing projectile atomic number $Z$, the cross-sections for which measurements are available or whose flux impact is $> 0.1\%$ in either Li, Be, B, C, N, O, F, Ne, Na, Mg, Al, or Si (flux impacts $> 1\%$ are highlighted in boldface). Short-lived nuclei (dubbed *ghost* nuclei) with respect to cosmic-ray propagation timescales are tagged with a star ($*$).

This review is based on the GALPROP[1] cross-section database assembled in the file `isotope_cs.dat` supplemented by some other references pointed out in [1, 2]. The references associated to the labels in the plots are provided in the bibliography of this Supplemental Material, except for a few labels that correspond to: [imos] = cross section renormalized by Igor Moskalenko; [TOBV] = target is natural Si (old database, no reference); [We96] = Webber 1996, private comm. (from [3]). Note that for a large number of important reactions no single measurement has been performed yet. We stress that for for some reactions (especially fragments of $^{56}$Fe), none of the above models matches the data. The reason is that data published $\gtrsim 2003$ were not included in the tuning of GP12 and GP22, and only partly for GP12up22 [1,2]. In particular, the reactions for $^{56}$Fe into Si, S, and P isotopes illustrates the fact that OPT22 is overall more accurate than OPT12 for previously uneasured reactions (as already highlighted in [8]). While these discrepancies are not on significant production channels, systematically updating the model on data (from the last two decades) will be part of our next effort to rank reactions up to $Z = 30$.

---

[1] Note that, in case of reactions $^{12}$C, $^{14}$N, $^{16}$O $\rightarrow$ $^{7}$A, $^{9}$A, $^{10}$A, $^{11}$A, the GALPROP code uses cumulative cross sections for $^{7}$Be, $^{9}$Be, $^{10}$Be, $^{10}$B, $^{11}$B instead of using individual cross sections as for many other channels. So, such individual cross sections as, e.g. $^{12}$C,$^{14}$N,$^{16}$O $\rightarrow$ $^{11}$C are set to zero to avoid double counting.

## Z=3 projectiles: $^{x}$Li + H $\rightarrow$ $^{A}_{Z}X$

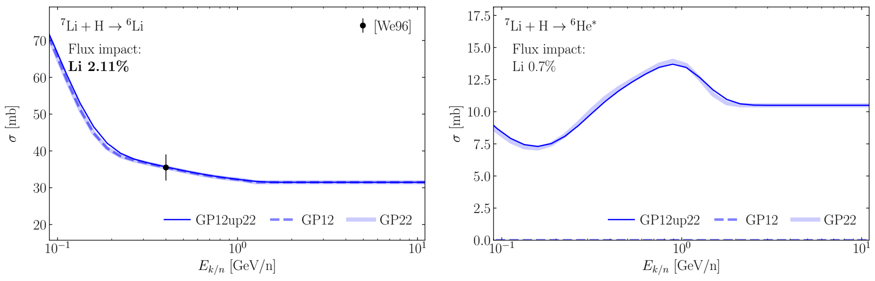


## Z=4 projectiles: $^{x}$Be + H $\rightarrow$ $^{A}_{Z}X$

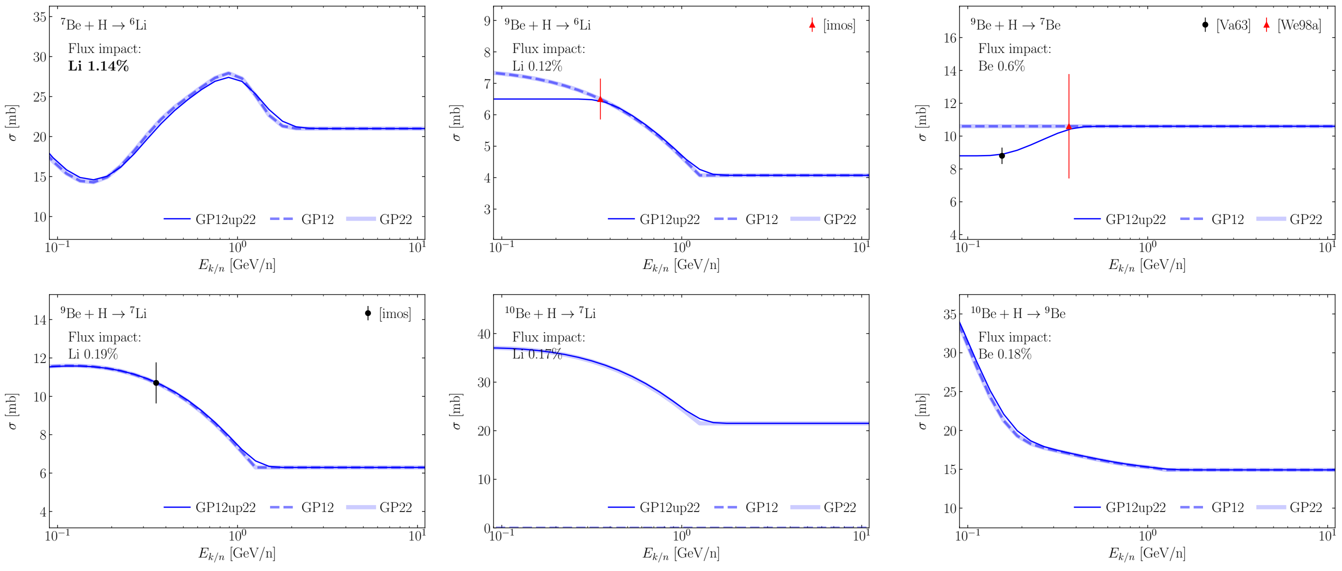


## Z=5 projectiles: $^{x}$B + H $\rightarrow$ $^{A}_{Z}X$

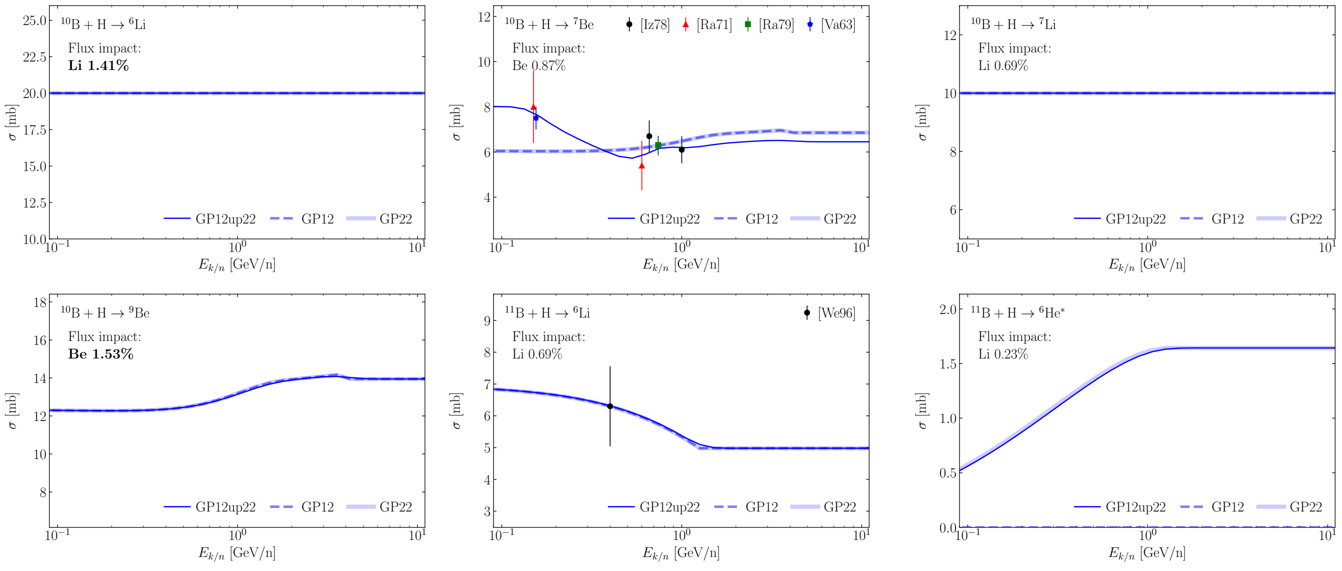

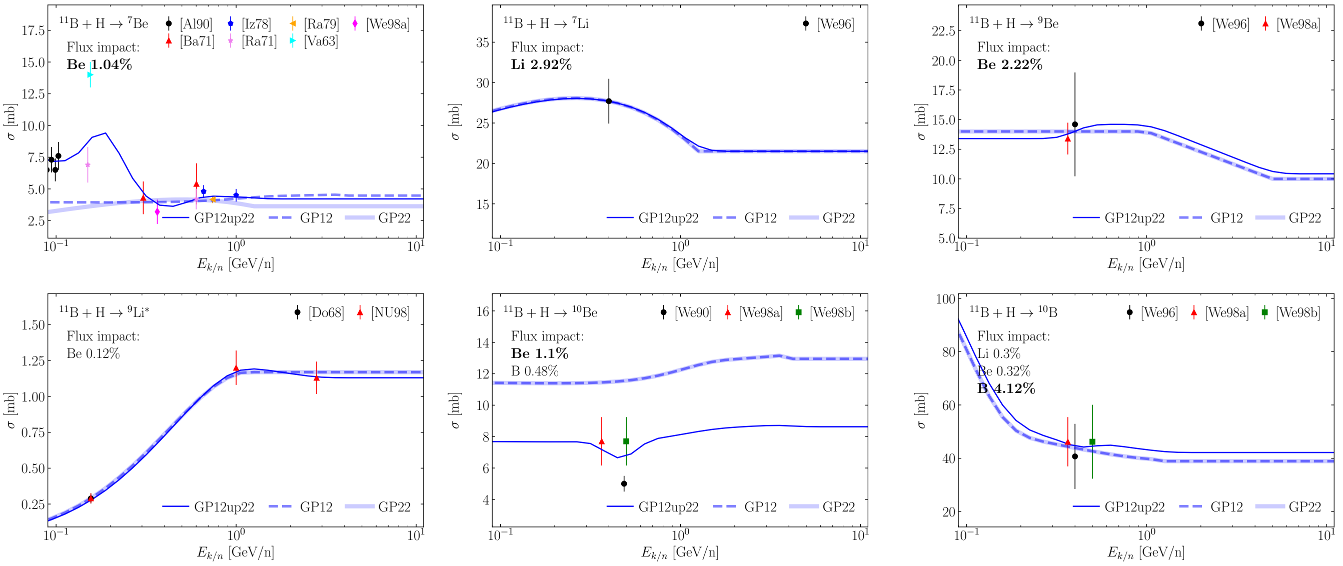


## Z=6 projectiles: $^{x}$C + H → $^{A}_{Z}X$

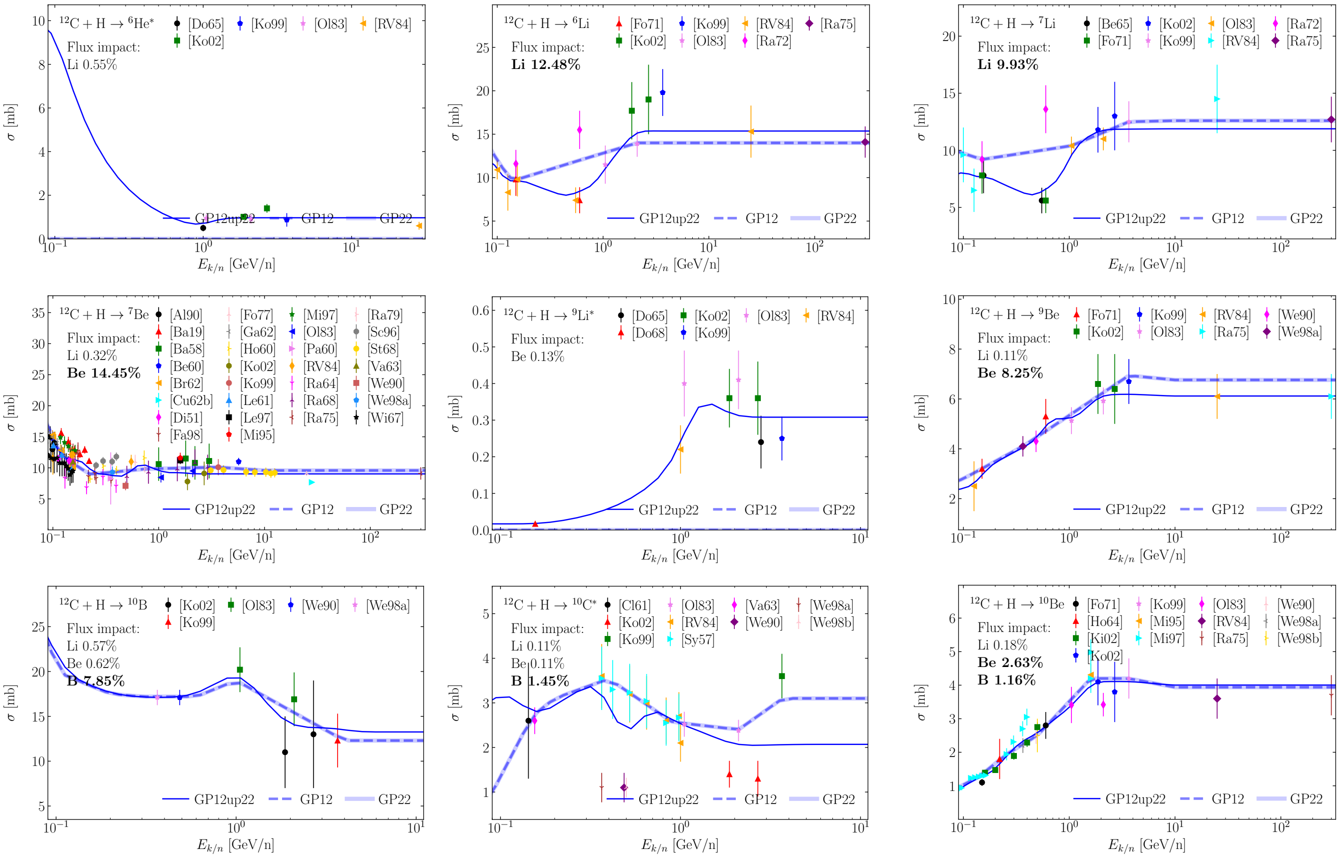

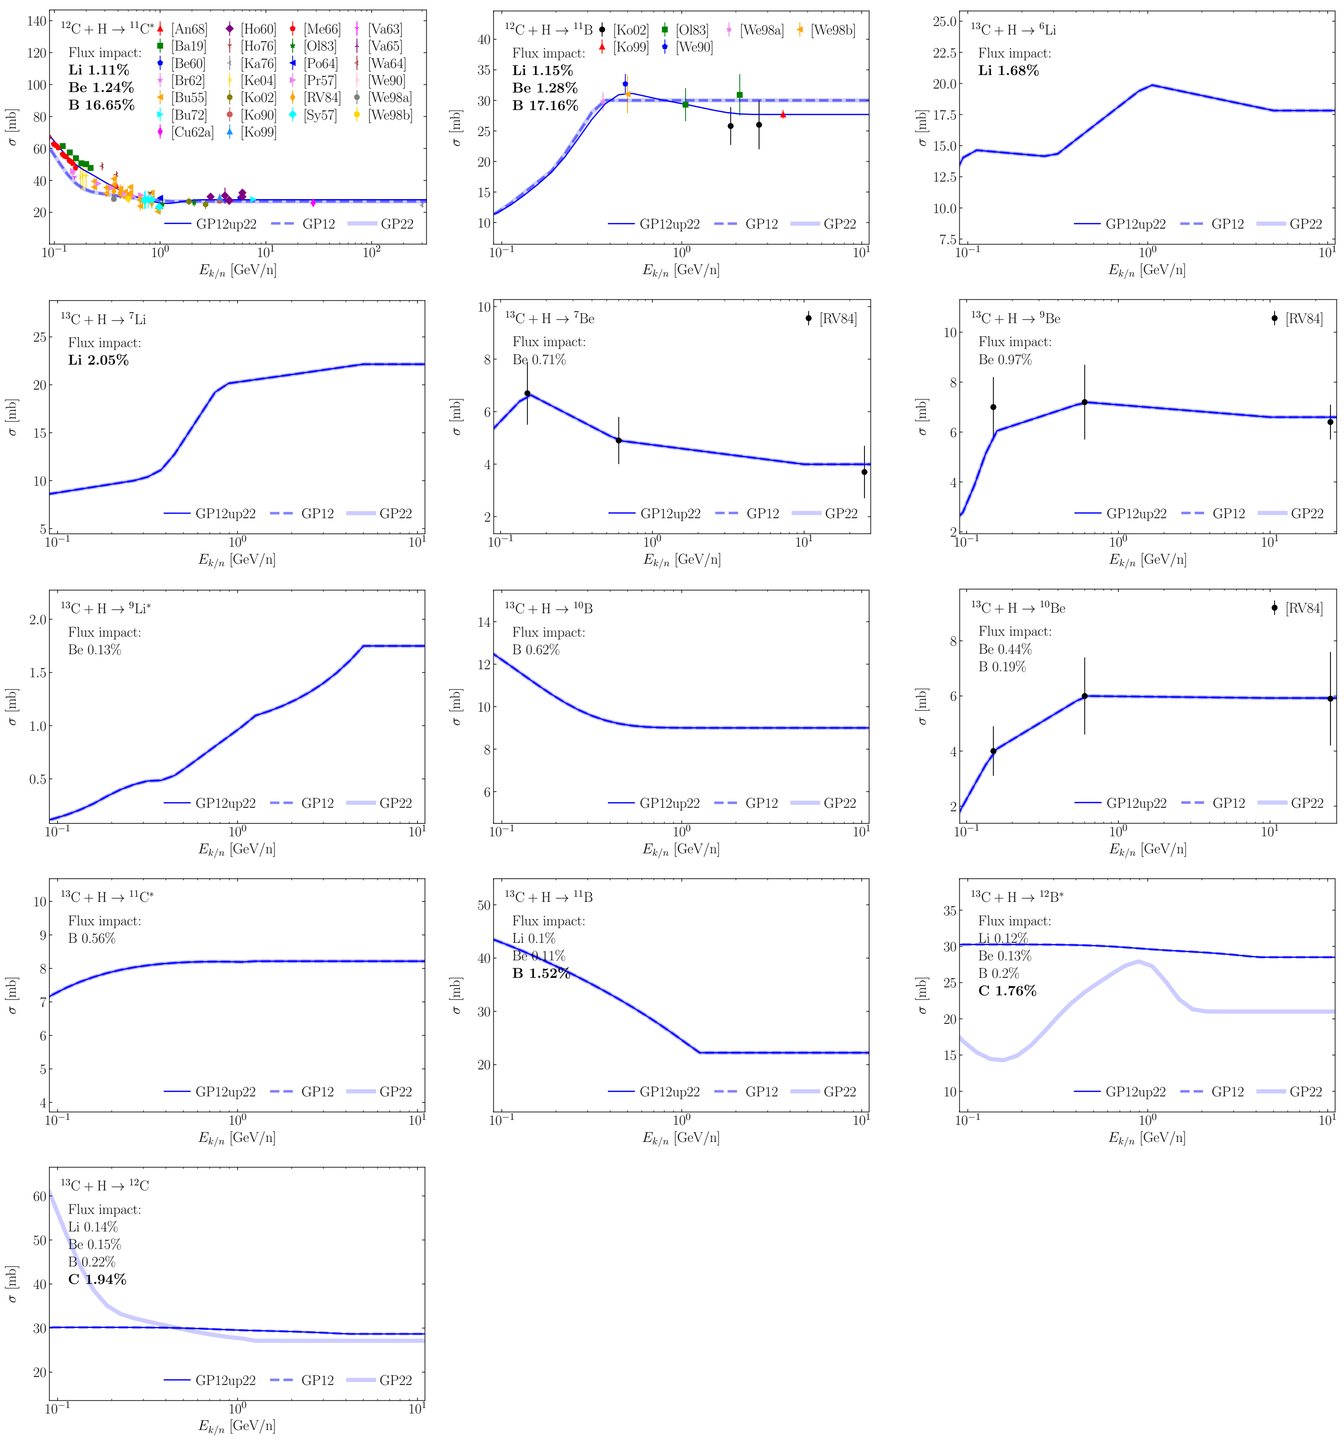


## Z=7 projectiles: $^{x}$N + H → $^{A}_{Z}X$

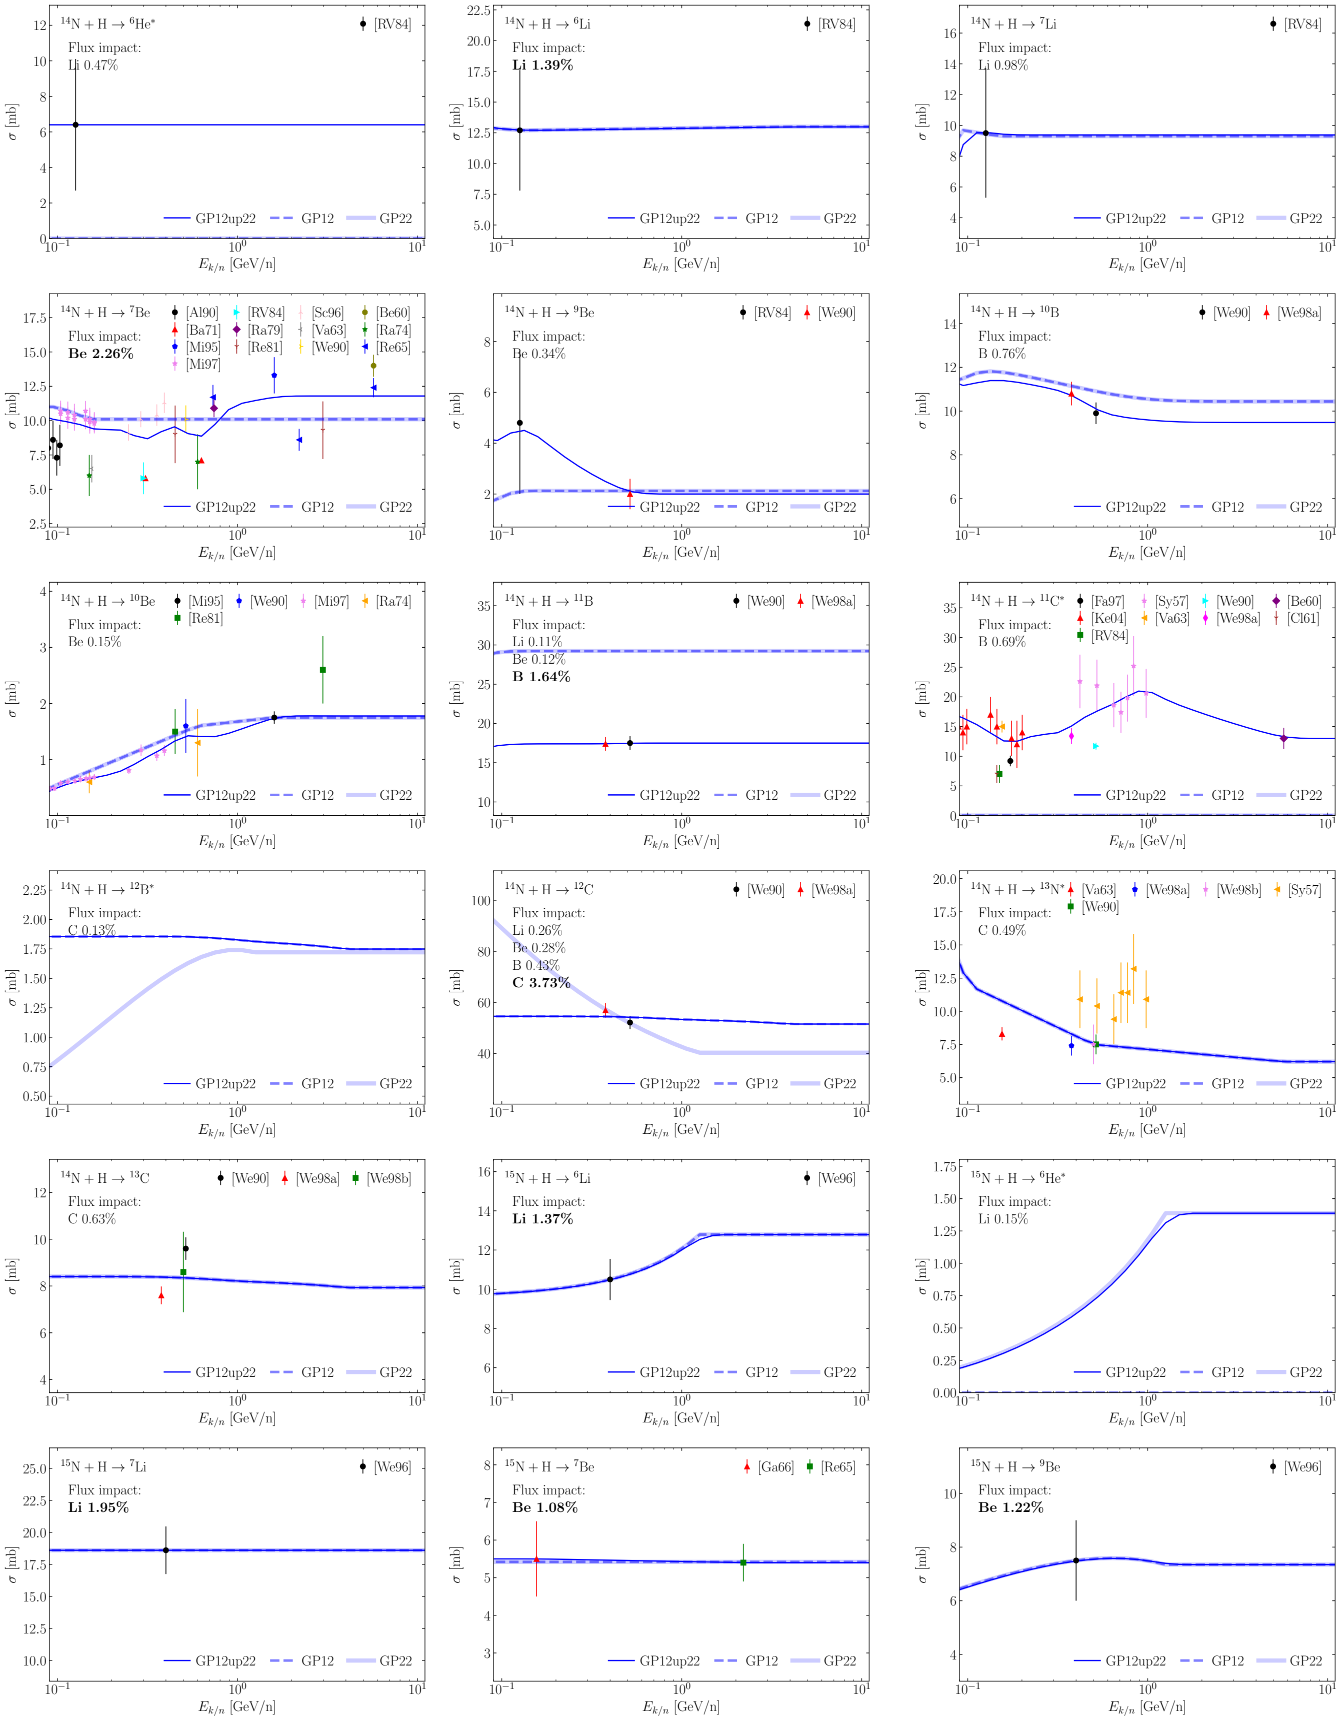

14N + H → 6He*
Flux impact:
Li 0.47%
14N + H → 6Li
Flux impact:
Li 1.39%
14N + H → 7Li
Flux impact:
Li 0.98%
14N + H → 7Be
Flux impact:
Be 2.26%
14N + H → 9Be
Flux impact:
Be 0.34%
14N + H → 10B
Flux impact:
B 0.76%
14N + H → 10Be
Flux impact:
Be 0.15%
14N + H → 11B
Flux impact:
Li 0.11%
Be 0.12%
B 1.64%
14N + H → 11C*
Flux impact:
B 0.69%
14N + H → 12B*
Flux impact:
C 0.13%
14N + H → 12C
Flux impact:
Li 0.26%
Be 0.28%
B 0.43%
C 3.73%
14N + H → 13N*
Flux impact:
C 0.49%
14N + H → 13C
Flux impact:
C 0.63%
15N + H → 6Li
Flux impact:
Li 1.37%
15N + H → 6He*
Flux impact:
Li 0.15%
15N + H → 7Li
Flux impact:
Li 1.95%
15N + H → 7Be
Flux impact:
Be 1.08%
15N + H → 9Be
Flux impact:
Be 1.22%
GP12up22
GP12
GP22
σ [mb]
Ek/n [GeV/n]

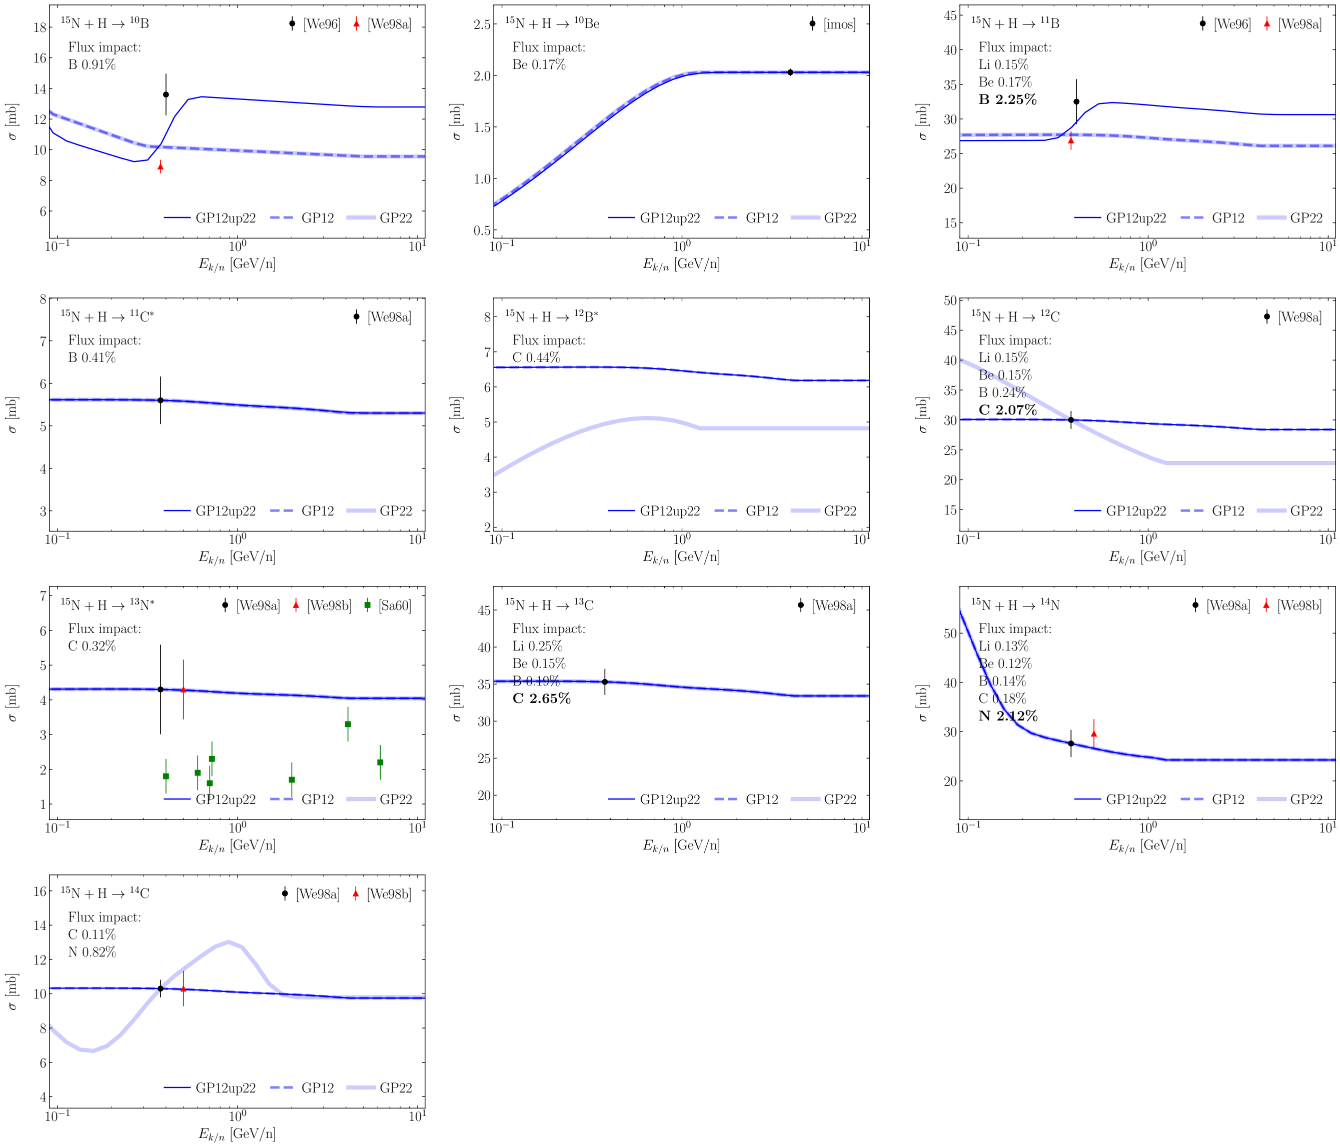


## Z=8 projectiles: $^{x}$O + H → $^{A}_{Z}X$

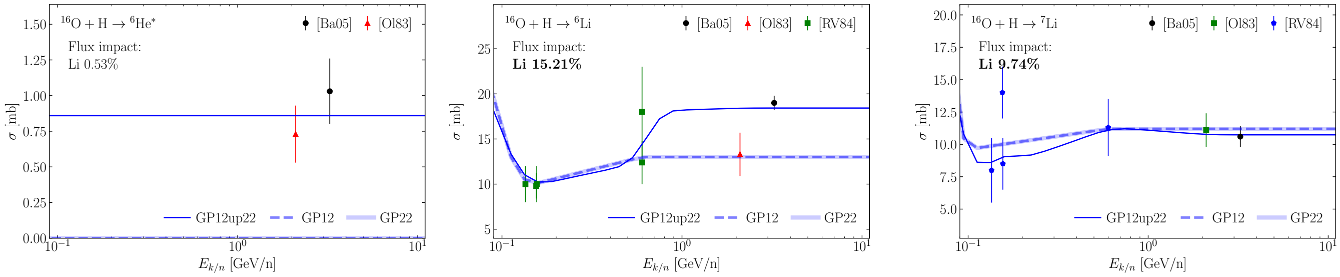

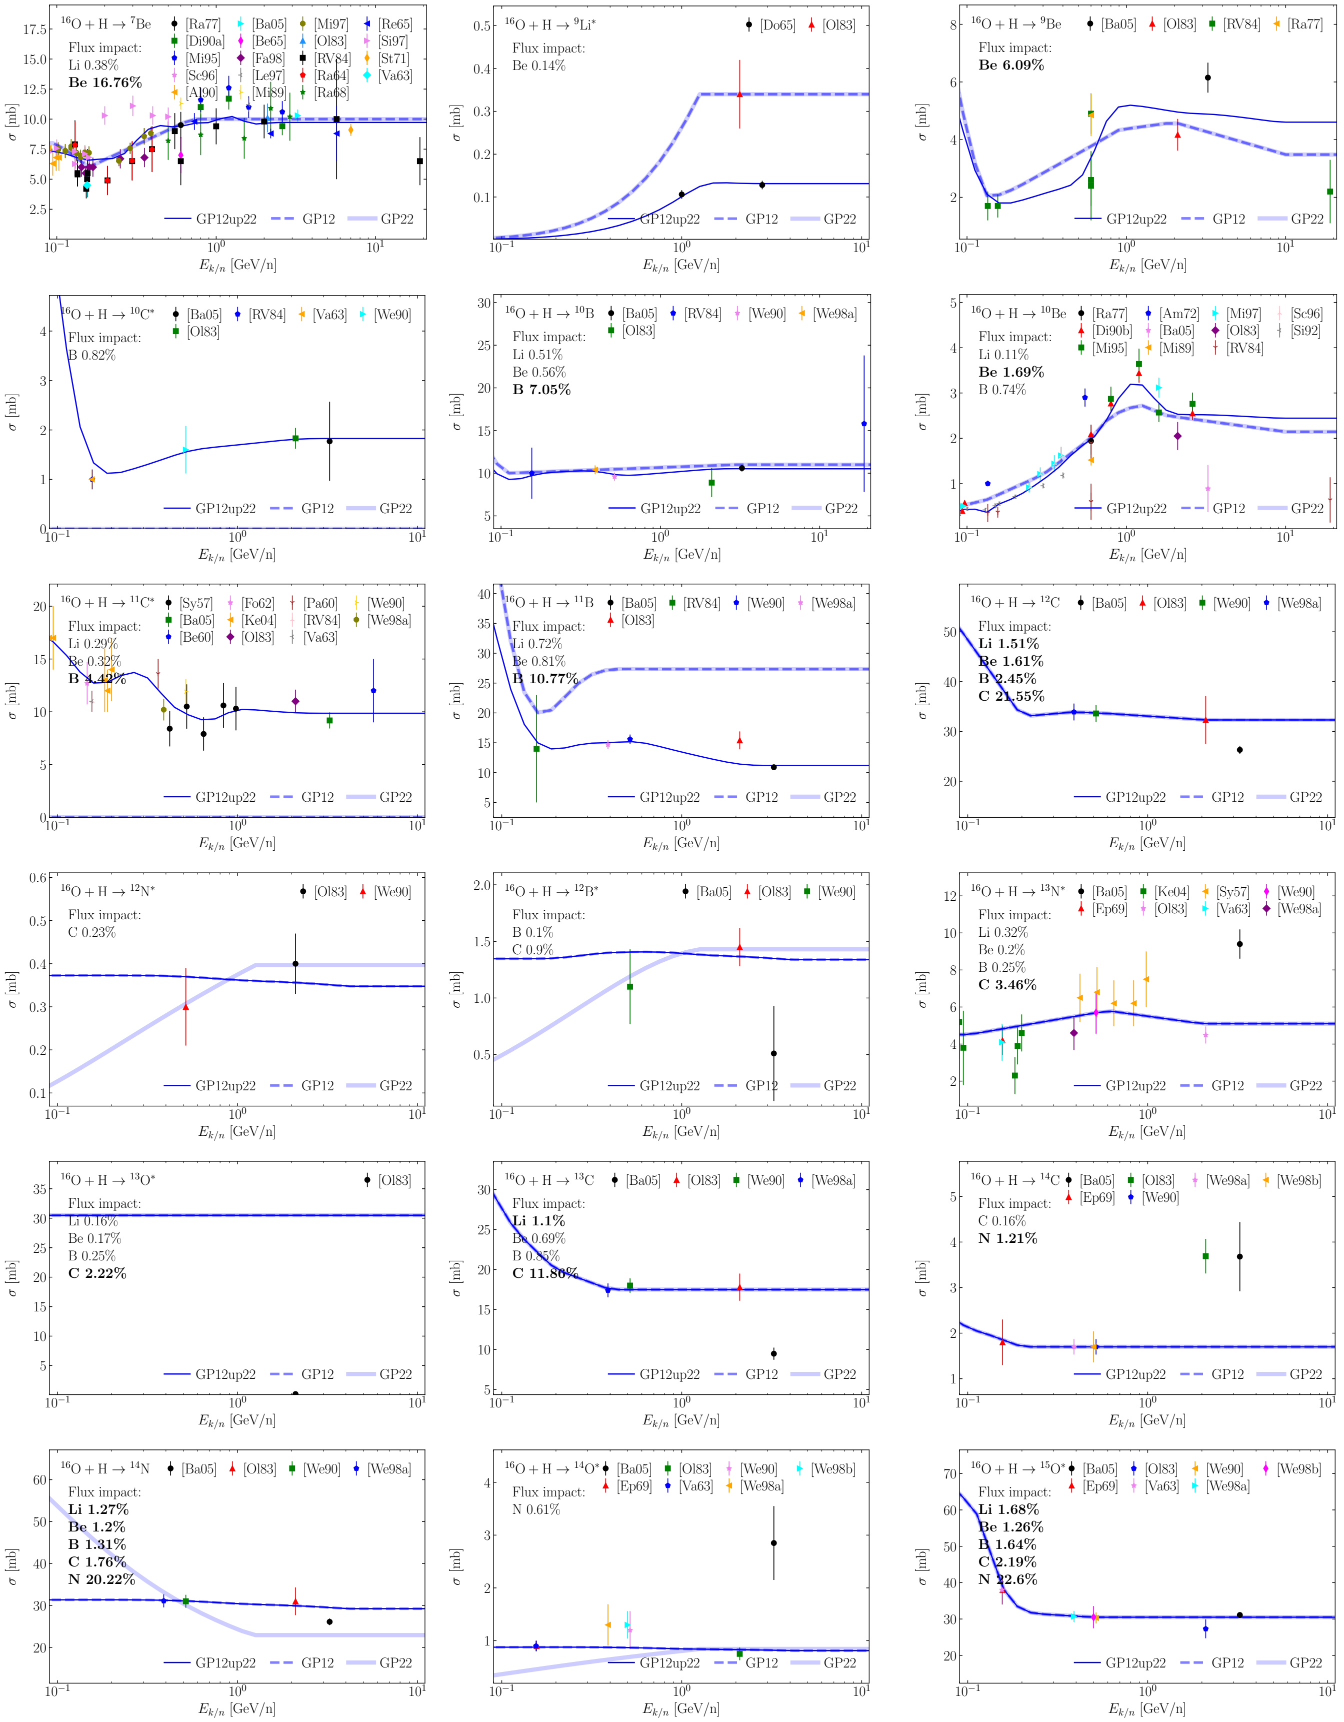

16O + H → 7Be
Flux impact:
Li 0.38%
Be 16.76%
16O + H → 9Li*
Flux impact:
Be 0.14%
16O + H → 9Be
Flux impact:
Be 6.09%
16O + H → 10C*
Flux impact:
B 0.82%
16O + H → 10B
Flux impact:
Li 0.51%
Be 0.56%
B 7.05%
16O + H → 10Be
Flux impact:
Li 0.11%
Be 1.69%
B 0.74%
16O + H → 11C*
Flux impact:
Li 0.29%
Be 0.32%
B 4.42%
16O + H → 11B
Flux impact:
Li 0.72%
Be 0.81%
B 10.77%
16O + H → 12C
Flux impact:
Li 1.51%
Be 1.61%
B 2.45%
C 21.55%
16O + H → 12N*
Flux impact:
C 0.23%
16O + H → 12B*
Flux impact:
B 0.1%
C 0.9%
16O + H → 13N*
Flux impact:
Li 0.32%
Be 0.2%
B 0.25%
C 3.46%
16O + H → 13O*
Flux impact:
Li 0.16%
Be 0.17%
B 0.25%
C 2.22%
16O + H → 13C
Flux impact:
Li 1.1%
Be 0.69%
B 0.85%
C 11.86%
16O + H → 14C
Flux impact:
C 0.16%
N 1.21%
16O + H → 14N
Flux impact:
Li 1.27%
Be 1.2%
B 1.31%
C 1.76%
N 20.22%
16O + H → 14O*
Flux impact:
N 0.61%
16O + H → 15O*
Flux impact:
Li 1.68%
Be 1.26%
B 1.64%
C 2.19%
N 22.6%
GP12up22
GP12
GP22
σ [mb]
E_k/n [GeV/n]

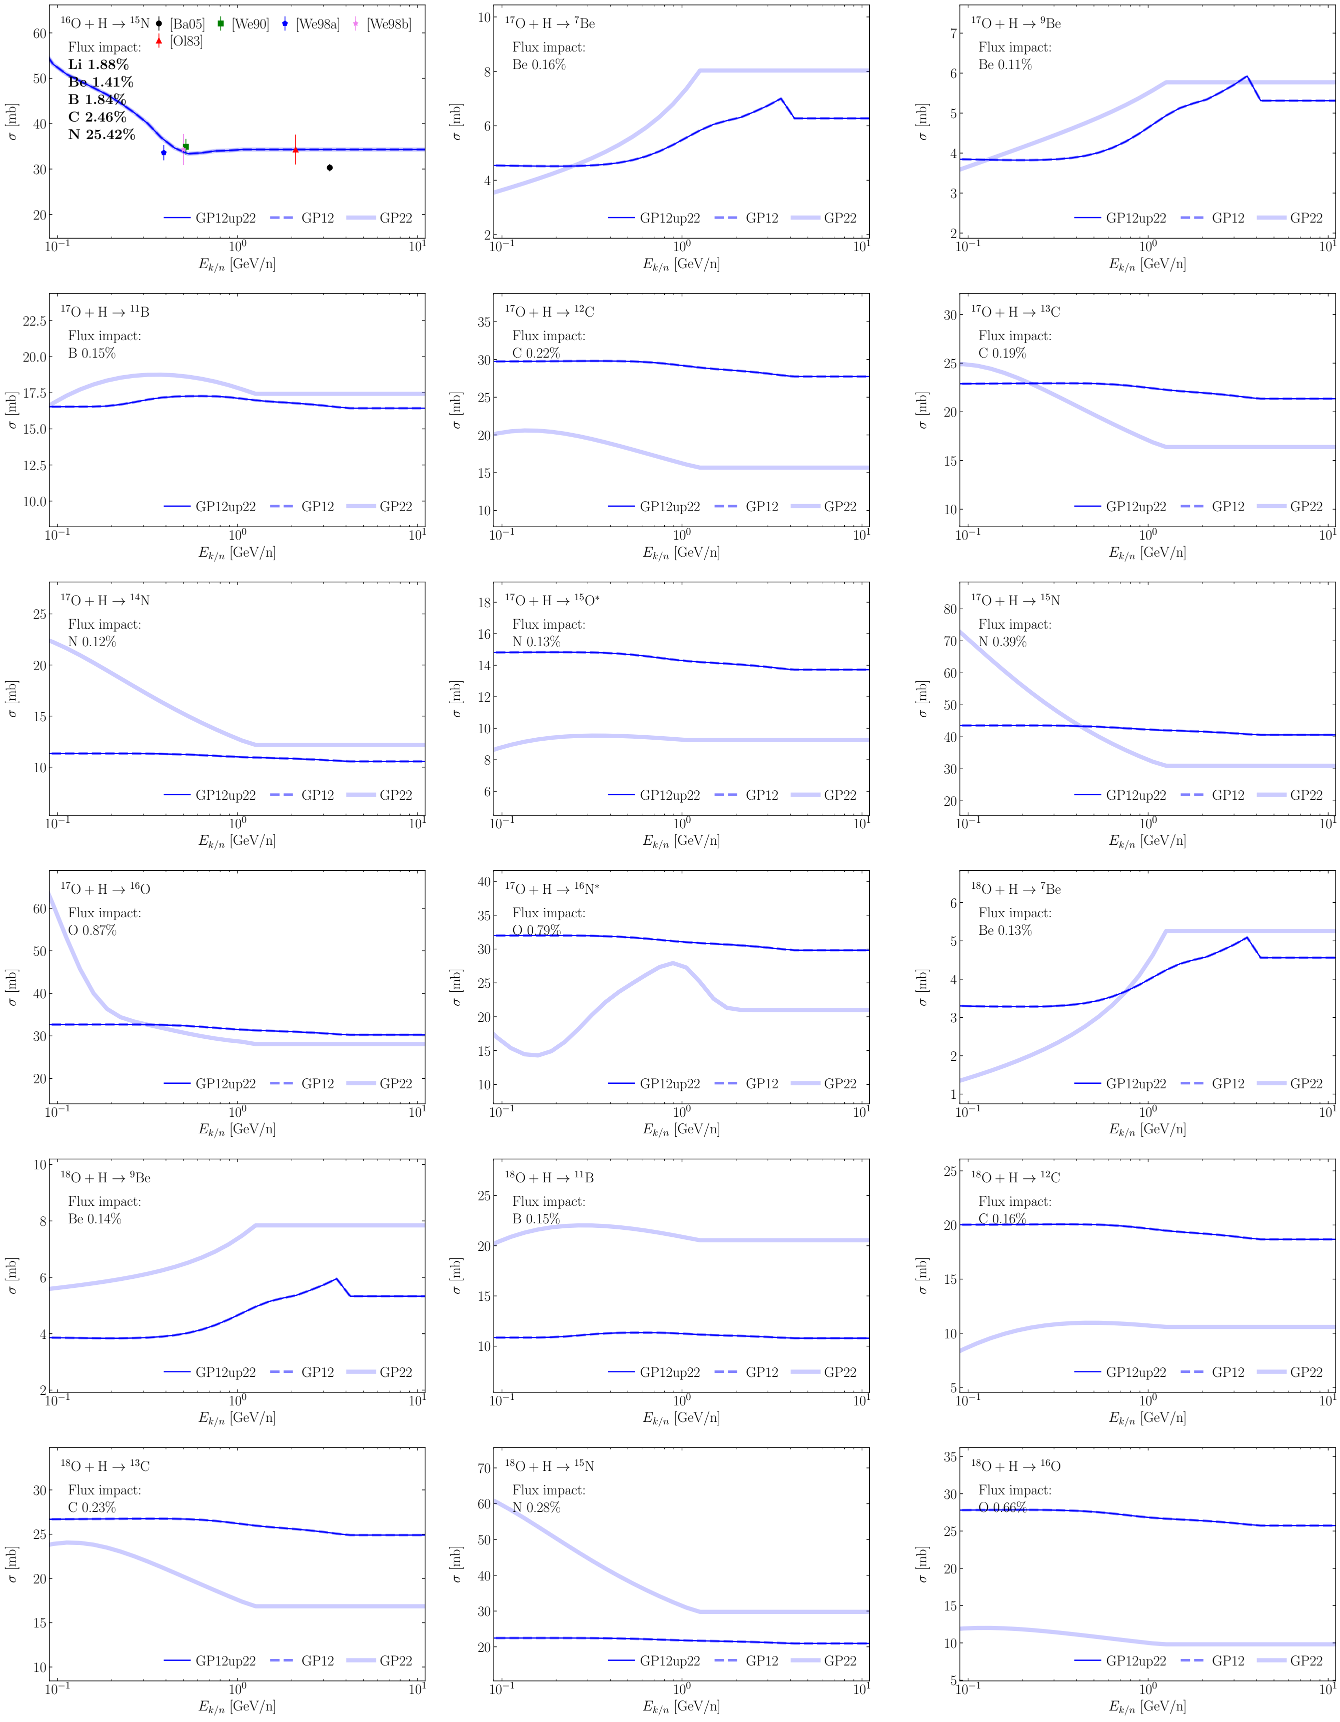
$^{16}$O + H → $^{15}$N
[Ba05] [We90] [We98a] [We98b] [Ol83]
Flux impact:
Li 1.88%
Be 1.41%
B 1.84%
C 2.46%
N 25.42%
$^{17}$O + H → $^{7}$Be
Flux impact:
Be 0.16%
$^{17}$O + H → $^{9}$Be
Flux impact:
Be 0.11%
$^{17}$O + H → $^{11}$B
Flux impact:
B 0.15%
$^{17}$O + H → $^{12}$C
Flux impact:
C 0.22%
$^{17}$O + H → $^{13}$C
Flux impact:
C 0.19%
$^{17}$O + H → $^{14}$N
Flux impact:
N 0.12%
$^{17}$O + H → $^{15}$O*
Flux impact:
N 0.13%
$^{17}$O + H → $^{15}$N
Flux impact:
N 0.39%
$^{17}$O + H → $^{16}$O
Flux impact:
O 0.87%
$^{17}$O + H → $^{16}$N*
Flux impact:
O 0.79%
$^{18}$O + H → $^{7}$Be
Flux impact:
Be 0.13%
$^{18}$O + H → $^{9}$Be
Flux impact:
Be 0.14%
$^{18}$O + H → $^{11}$B
Flux impact:
B 0.15%
$^{18}$O + H → $^{12}$C
Flux impact:
C 0.16%
$^{18}$O + H → $^{13}$C
Flux impact:
C 0.23%
$^{18}$O + H → $^{15}$N
Flux impact:
N 0.28%
$^{18}$O + H → $^{16}$O
Flux impact:
O 0.66%
GP12up22
GP12
GP22
$\sigma$ [mb]
$E_{k/n}$ [GeV/n]

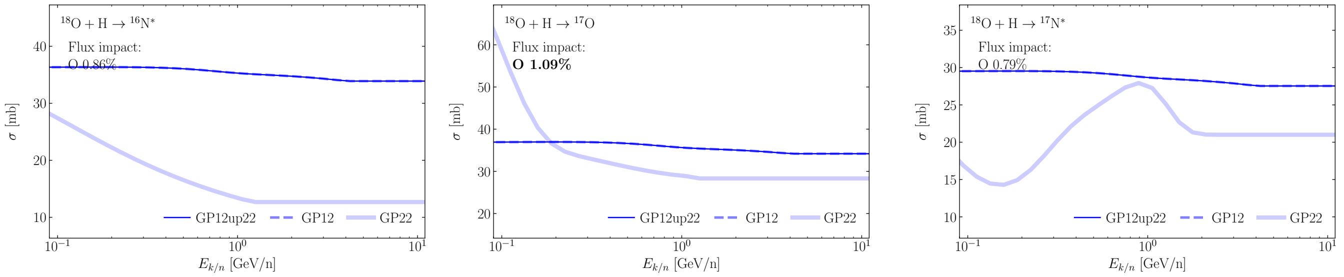


## Z=9 projectiles: $^{x}$F + H → $^{A}_{Z}X$

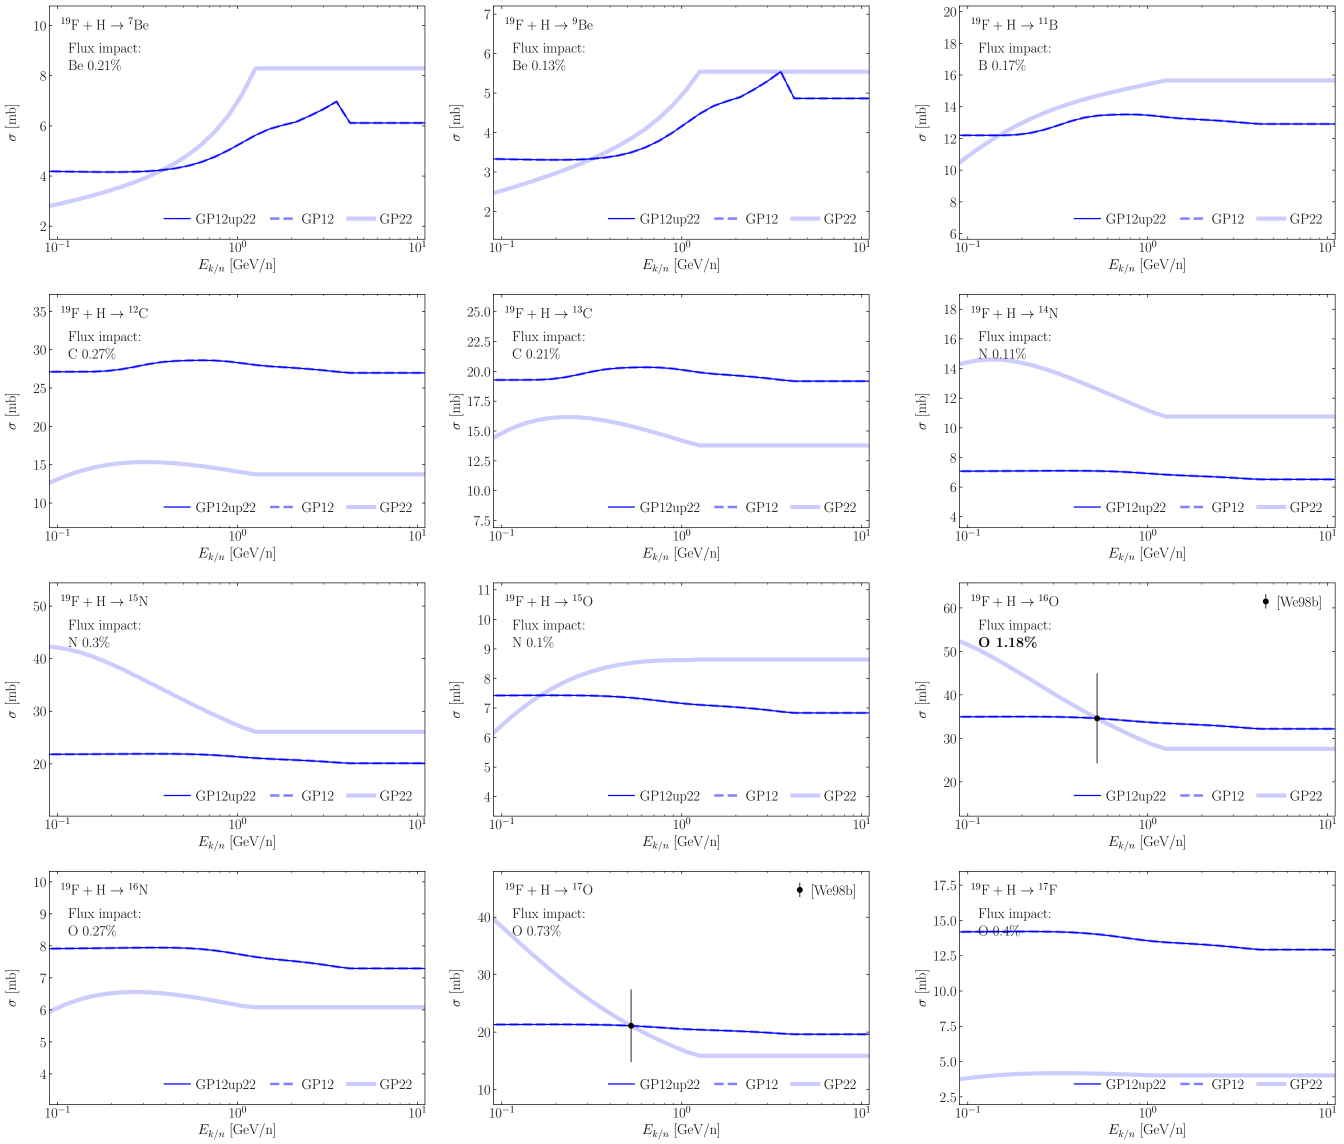

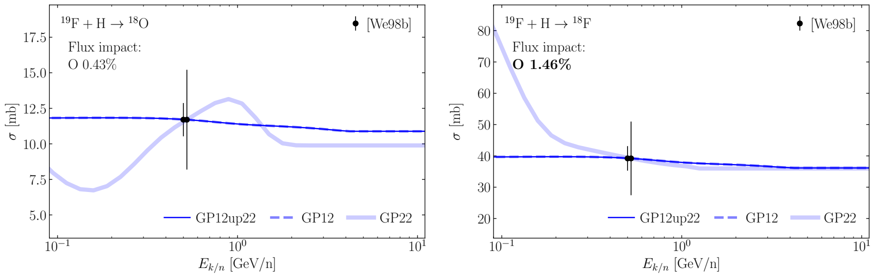


## Z=10 projectiles: $^{x}$Ne + H → $^{A}_{Z}X$

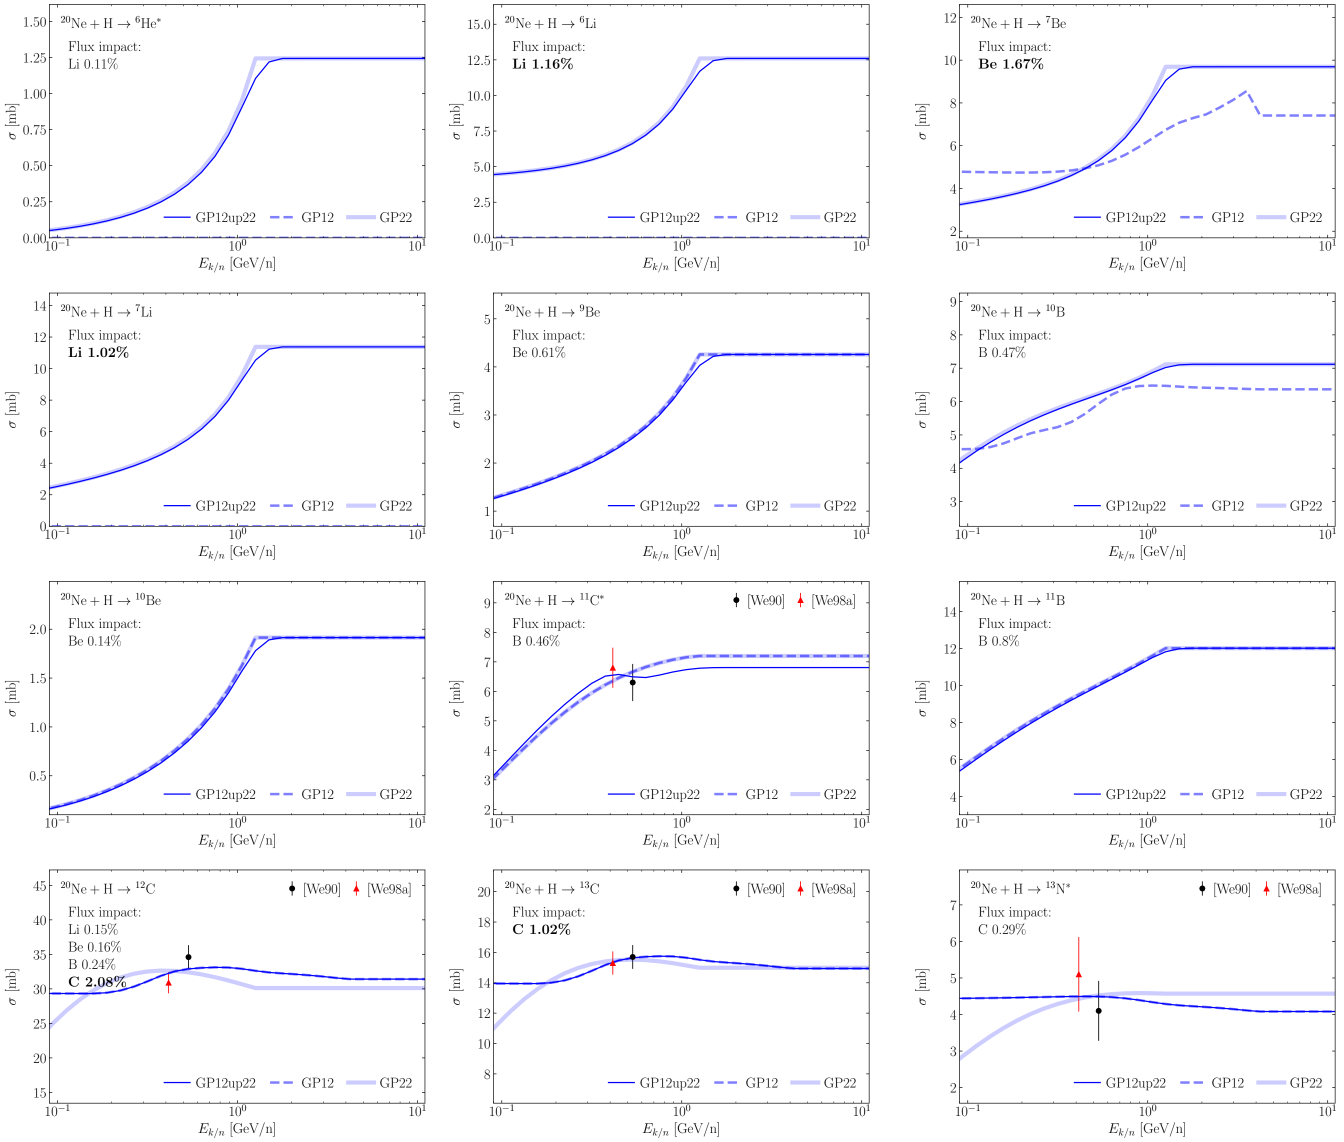

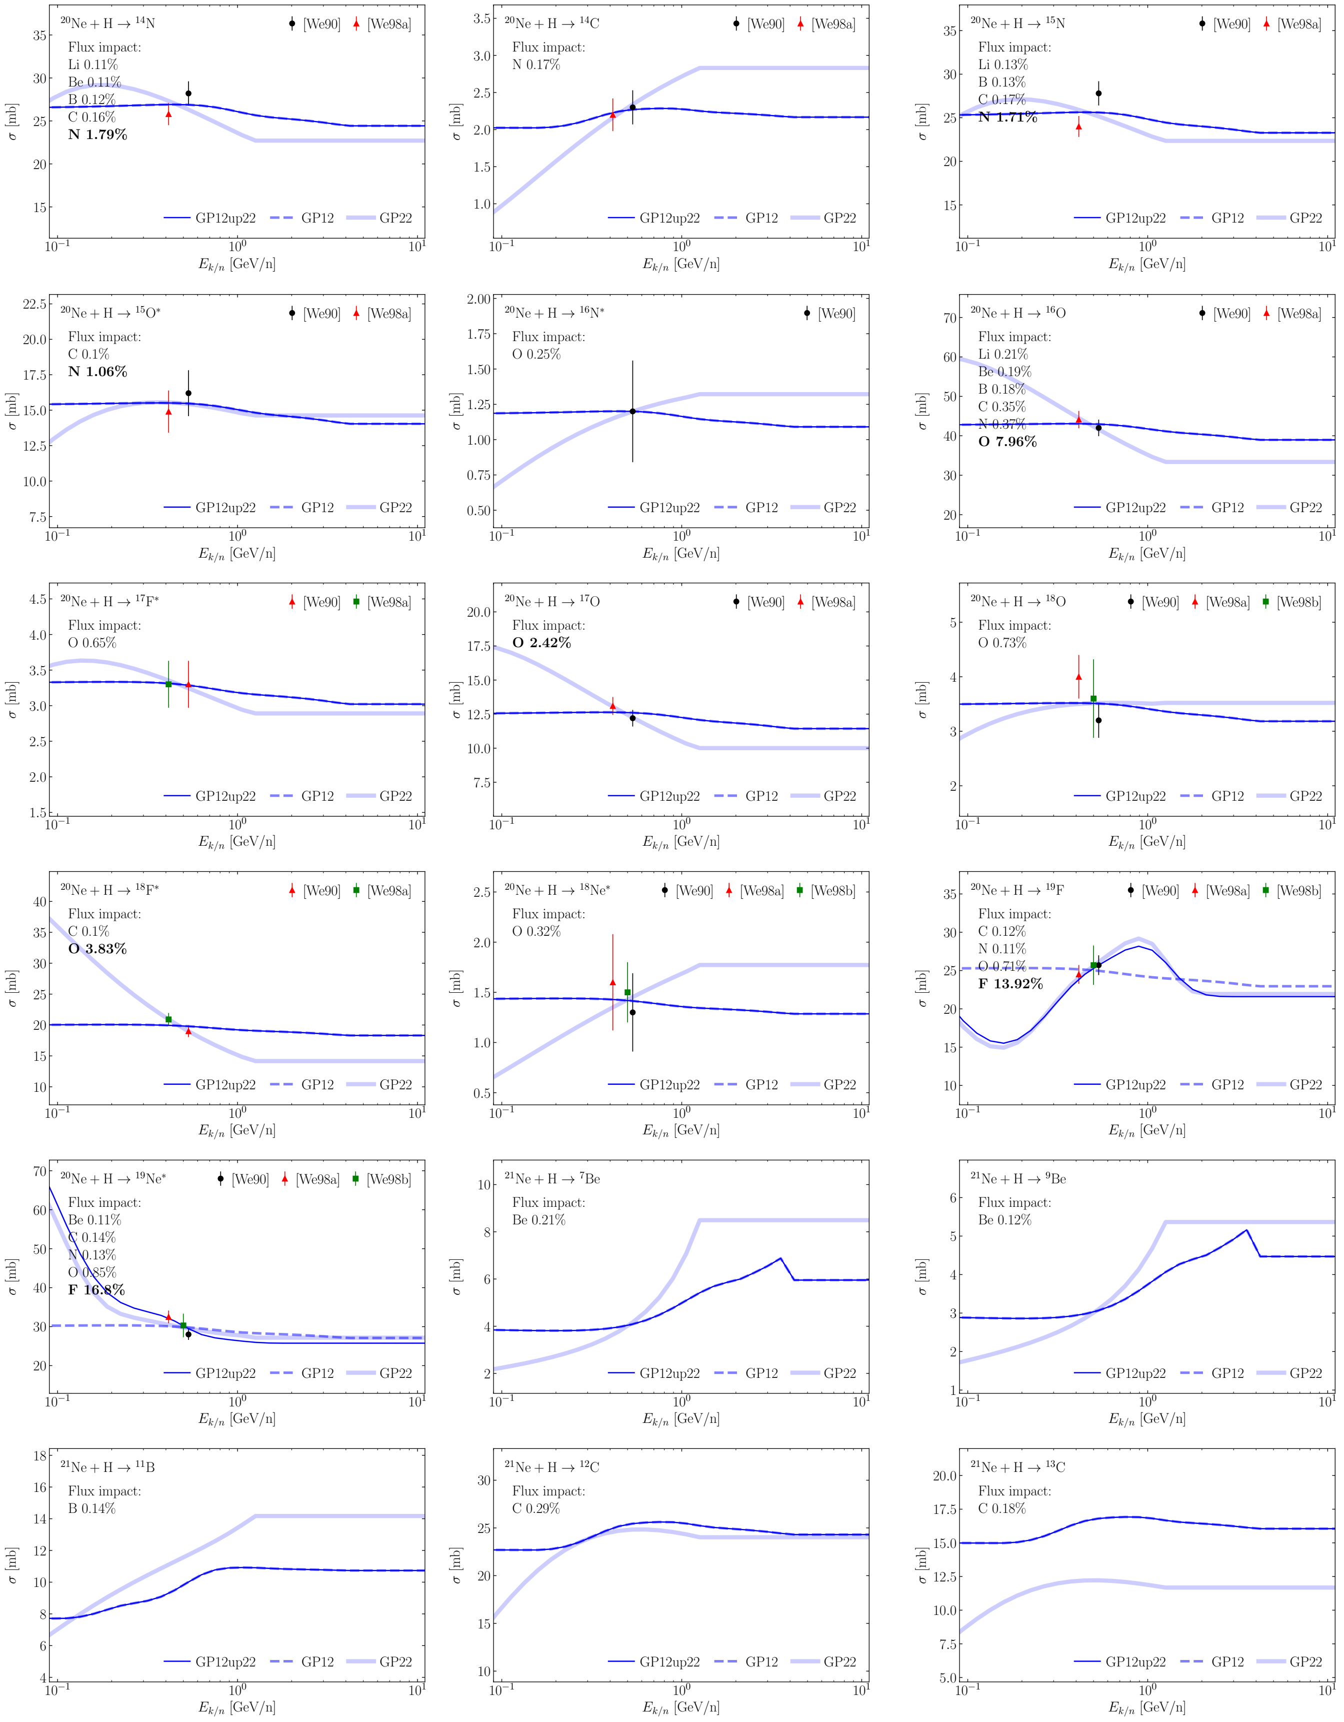

$^{20}$Ne + H → $^{14}$N
[We90] [We98a]
Flux impact:
Li 0.11%
Be 0.11%
B 0.12%
C 0.16%
N 1.79%
$^{20}$Ne + H → $^{14}$C
[We90] [We98a]
Flux impact:
N 0.17%
$^{20}$Ne + H → $^{15}$N
[We90] [We98a]
Flux impact:
Li 0.13%
B 0.13%
C 0.17%
N 1.71%
$^{20}$Ne + H → $^{15}$O*
[We90] [We98a]
Flux impact:
C 0.1%
N 1.06%
$^{20}$Ne + H → $^{16}$N*
[We90]
Flux impact:
O 0.25%
$^{20}$Ne + H → $^{16}$O
[We90] [We98a]
Flux impact:
Li 0.21%
Be 0.19%
B 0.18%
C 0.35%
N 0.37%
O 7.96%
$^{20}$Ne + H → $^{17}$F*
[We90] [We98a]
Flux impact:
O 0.65%
$^{20}$Ne + H → $^{17}$O
[We90] [We98a]
Flux impact:
O 2.42%
$^{20}$Ne + H → $^{18}$O
[We90] [We98a] [We98b]
Flux impact:
O 0.73%
$^{20}$Ne + H → $^{18}$F*
[We90] [We98a]
Flux impact:
C 0.1%
O 3.83%
$^{20}$Ne + H → $^{18}$Ne*
[We90] [We98a] [We98b]
Flux impact:
O 0.32%
$^{20}$Ne + H → $^{19}$F
[We90] [We98a] [We98b]
Flux impact:
C 0.12%
N 0.11%
O 0.71%
F 13.92%
$^{20}$Ne + H → $^{19}$Ne*
[We90] [We98a] [We98b]
Flux impact:
Be 0.11%
C 0.14%
N 0.13%
O 0.85%
F 16.8%
$^{21}$Ne + H → $^{7}$Be
Flux impact:
Be 0.21%
$^{21}$Ne + H → $^{9}$Be
Flux impact:
Be 0.12%
$^{21}$Ne + H → $^{11}$B
Flux impact:
B 0.14%
$^{21}$Ne + H → $^{12}$C
Flux impact:
C 0.29%
$^{21}$Ne + H → $^{13}$C
Flux impact:
C 0.18%
GP12up22 GP12 GP22
$\sigma$ [mb]
$E_{k/n}$ [GeV/n]

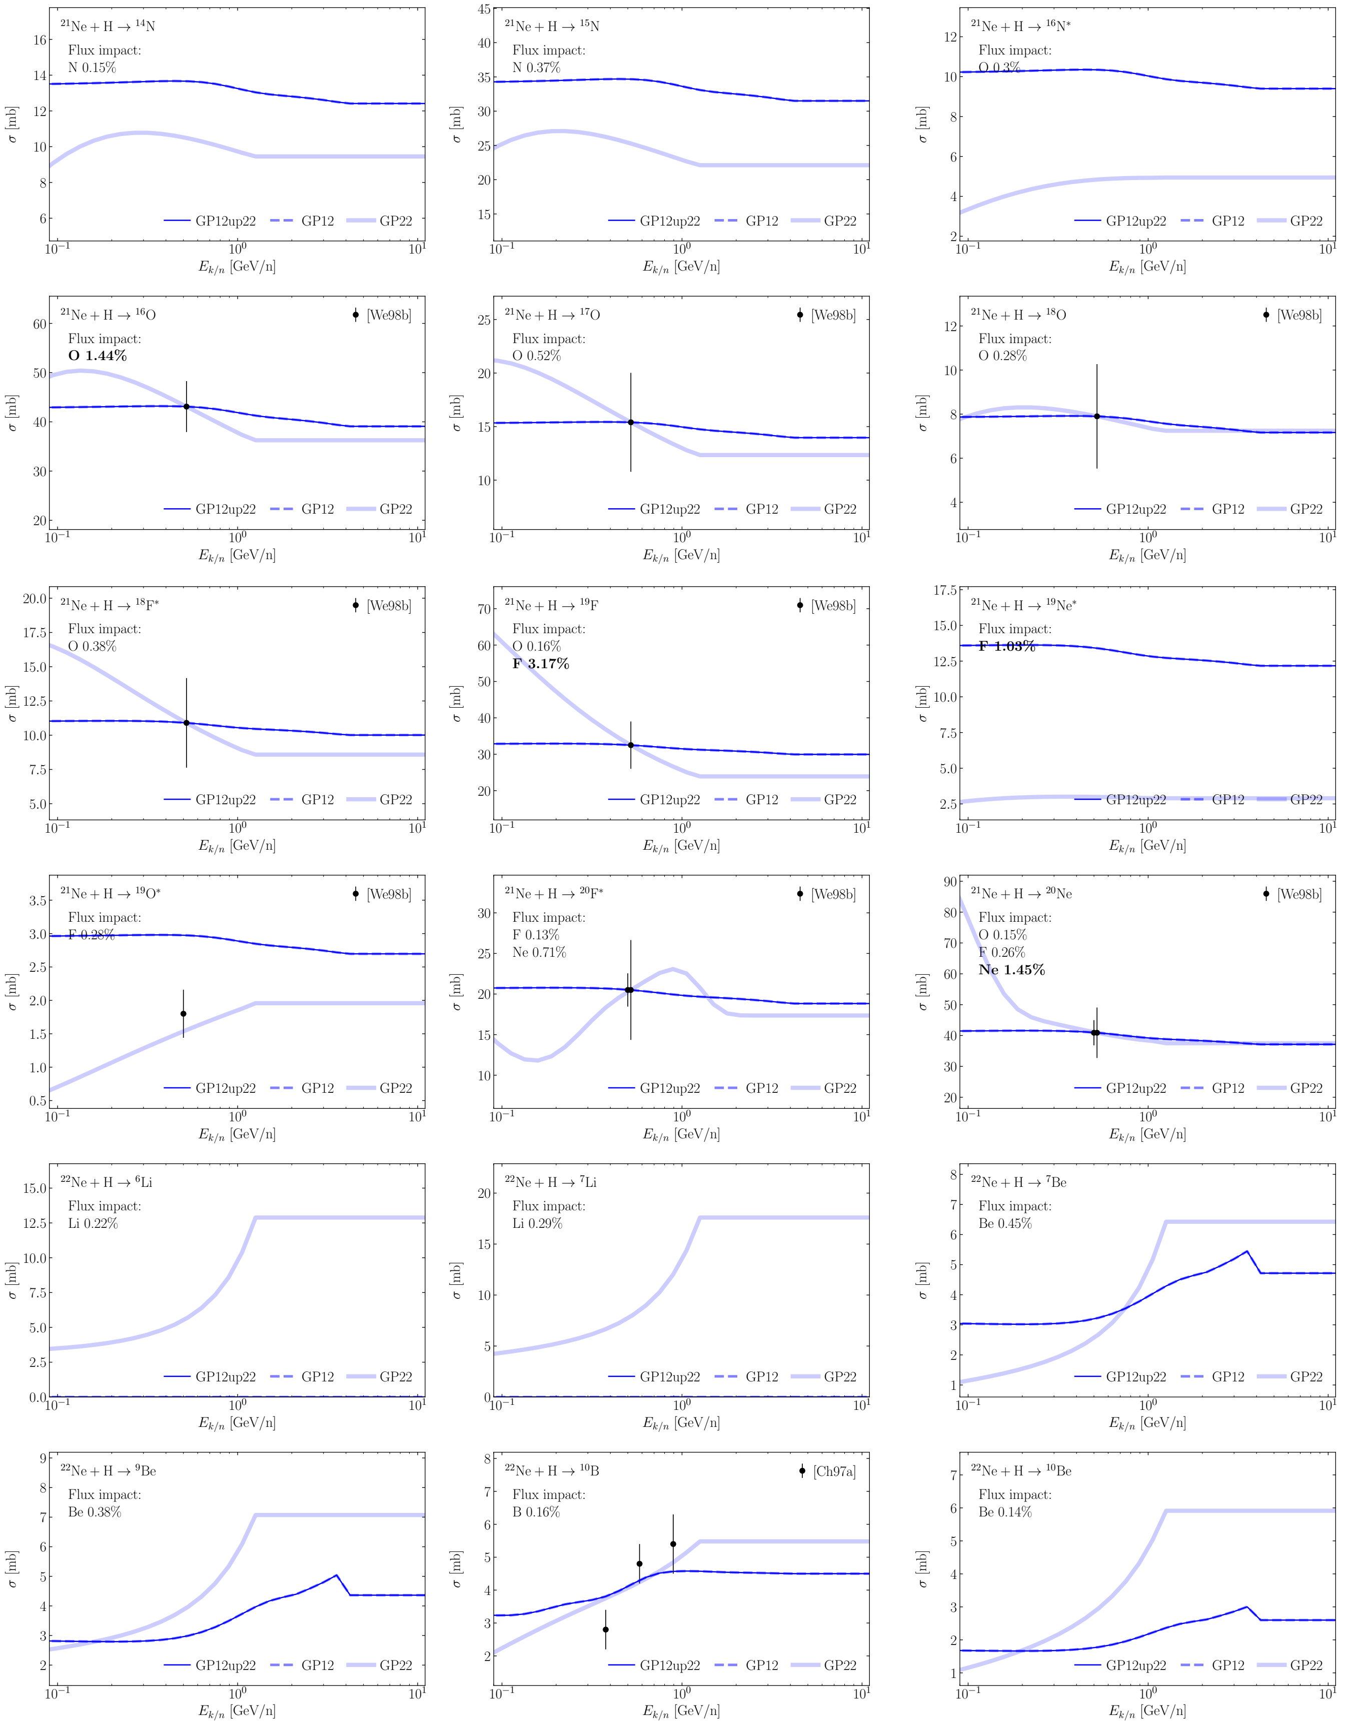

$^{21}$Ne + H → $^{14}$N
Flux impact:
N 0.15%
$^{21}$Ne + H → $^{15}$N
Flux impact:
N 0.37%
$^{21}$Ne + H → $^{16}$N*
Flux impact:
O 0.3%
$^{21}$Ne + H → $^{16}$O
[We98b]
Flux impact:
O 1.44%
$^{21}$Ne + H → $^{17}$O
[We98b]
Flux impact:
O 0.52%
$^{21}$Ne + H → $^{18}$O
[We98b]
Flux impact:
O 0.28%
$^{21}$Ne + H → $^{18}$F*
[We98b]
Flux impact:
O 0.38%
$^{21}$Ne + H → $^{19}$F
[We98b]
Flux impact:
O 0.16%
F 3.17%
$^{21}$Ne + H → $^{19}$Ne*
Flux impact:
F 1.03%
$^{21}$Ne + H → $^{19}$O*
[We98b]
Flux impact:
F 0.28%
$^{21}$Ne + H → $^{20}$F*
[We98b]
Flux impact:
F 0.13%
Ne 0.71%
$^{21}$Ne + H → $^{20}$Ne
[We98b]
Flux impact:
O 0.15%
F 0.26%
Ne 1.45%
$^{22}$Ne + H → $^{6}$Li
Flux impact:
Li 0.22%
$^{22}$Ne + H → $^{7}$Li
Flux impact:
Li 0.29%
$^{22}$Ne + H → $^{7}$Be
Flux impact:
Be 0.45%
$^{22}$Ne + H → $^{9}$Be
Flux impact:
Be 0.38%
$^{22}$Ne + H → $^{10}$B
[Ch97a]
Flux impact:
B 0.16%
$^{22}$Ne + H → $^{10}$Be
Flux impact:
Be 0.14%
GP12up22
GP12
GP22
$\sigma$ [mb]
$E_{k/n}$ [GeV/n]

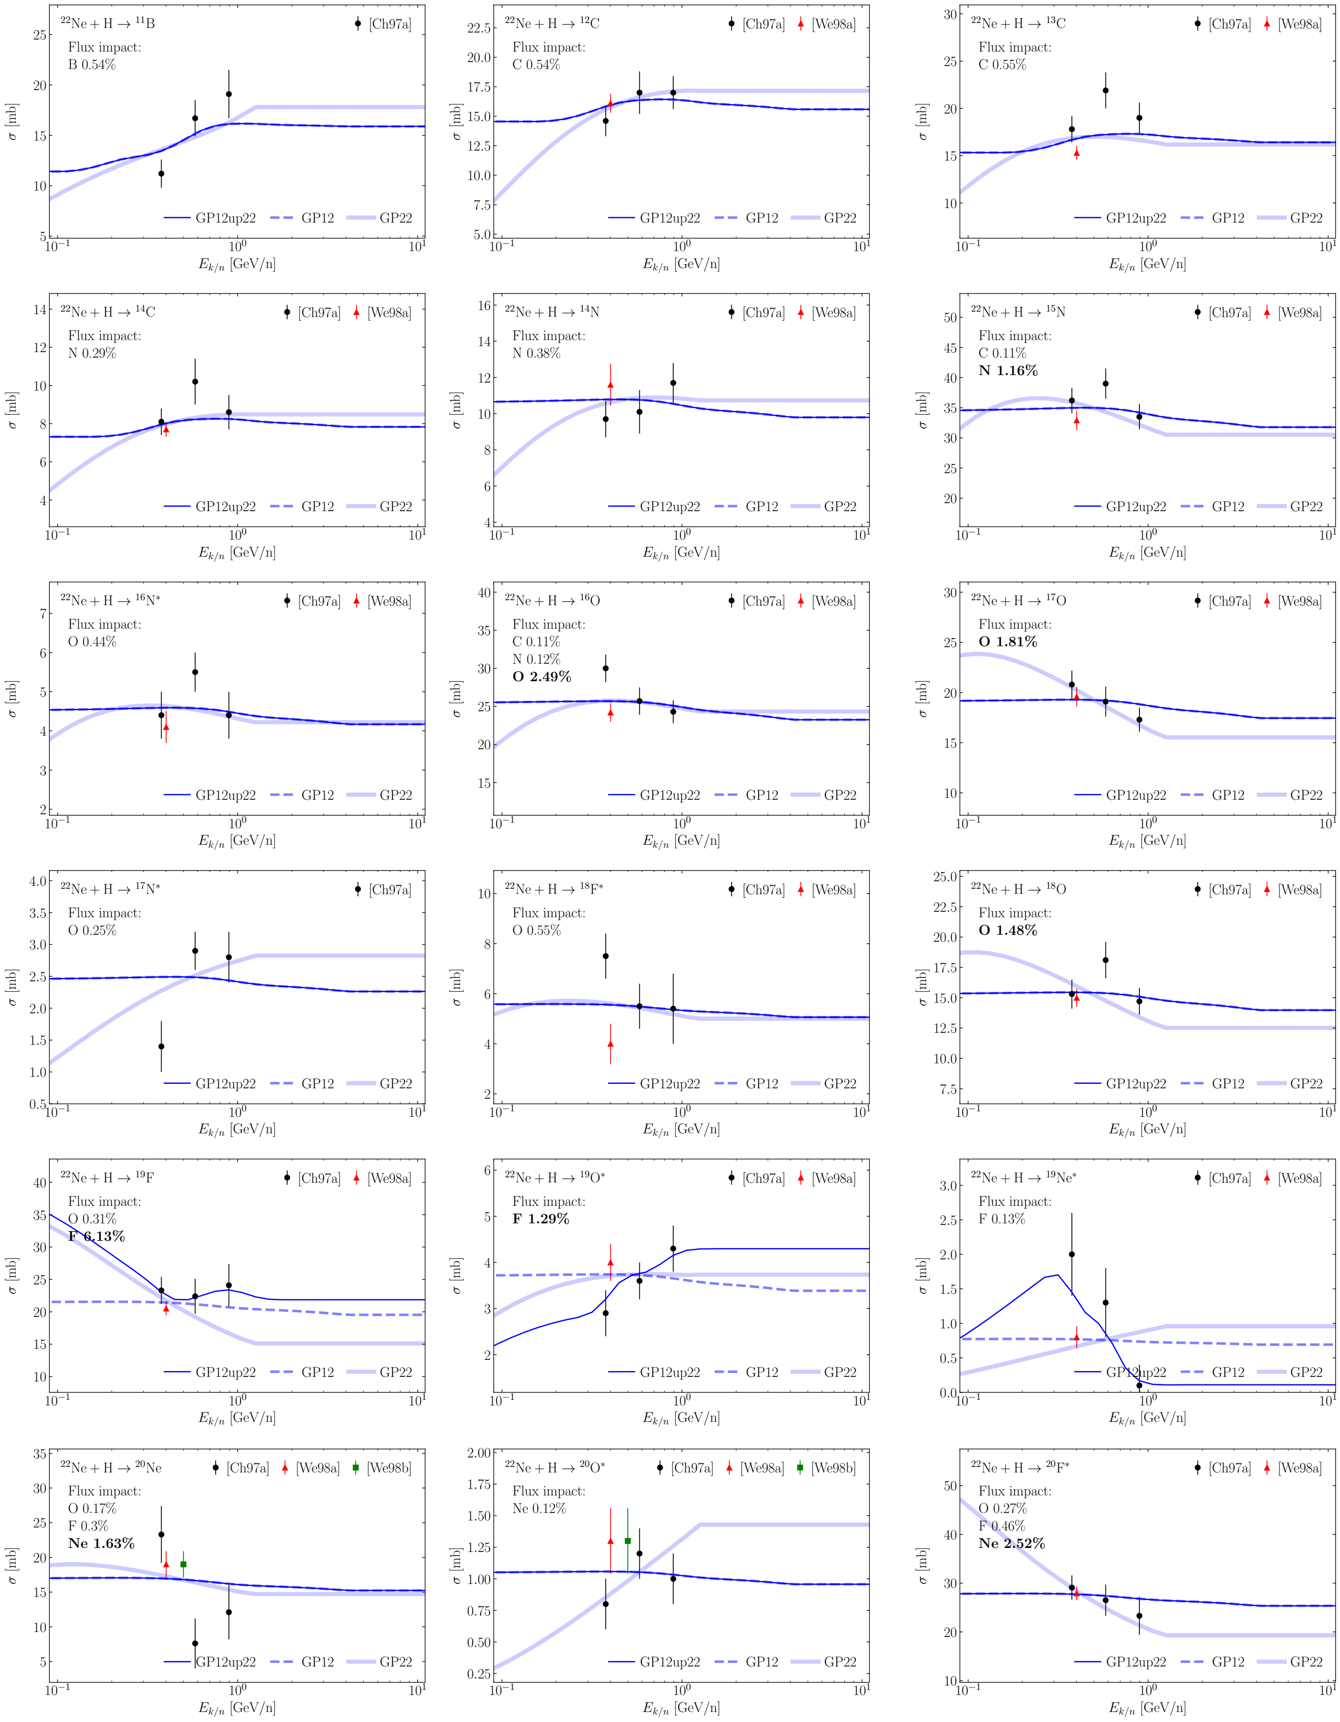

²²Ne + H → ¹¹B
[Ch97a]
Flux impact:
B 0.54%
²²Ne + H → ¹²C
[Ch97a] [We98a]
Flux impact:
C 0.54%
²²Ne + H → ¹³C
[Ch97a] [We98a]
Flux impact:
C 0.55%
²²Ne + H → ¹⁴C
[Ch97a] [We98a]
Flux impact:
N 0.29%
²²Ne + H → ¹⁴N
[Ch97a] [We98a]
Flux impact:
N 0.38%
²²Ne + H → ¹⁵N
[Ch97a] [We98a]
Flux impact:
C 0.11%
N 1.16%
²²Ne + H → ¹⁶N*
[Ch97a] [We98a]
Flux impact:
O 0.44%
²²Ne + H → ¹⁶O
[Ch97a] [We98a]
Flux impact:
C 0.11%
N 0.12%
O 2.49%
²²Ne + H → ¹⁷O
[Ch97a] [We98a]
Flux impact:
O 1.81%
²²Ne + H → ¹⁷N*
[Ch97a]
Flux impact:
O 0.25%
²²Ne + H → ¹⁸F*
[Ch97a] [We98a]
Flux impact:
O 0.55%
²²Ne + H → ¹⁸O
[Ch97a] [We98a]
Flux impact:
O 1.48%
²²Ne + H → ¹⁹F
[Ch97a] [We98a]
Flux impact:
O 0.31%
F 6.13%
²²Ne + H → ¹⁹O*
[Ch97a] [We98a]
Flux impact:
F 1.29%
²²Ne + H → ¹⁹Ne*
[Ch97a] [We98a]
Flux impact:
F 0.13%
²²Ne + H → ²⁰Ne
[Ch97a] [We98a] [We98b]
Flux impact:
O 0.17%
F 0.3%
Ne 1.63%
²²Ne + H → ²⁰O*
[Ch97a] [We98a] [We98b]
Flux impact:
Ne 0.12%
²²Ne + H → ²⁰F*
[Ch97a] [We98a]
Flux impact:
O 0.27%
F 0.46%
Ne 2.52%
GP12up22
GP12
GP22
σ [mb]
E_k/n [GeV/n]

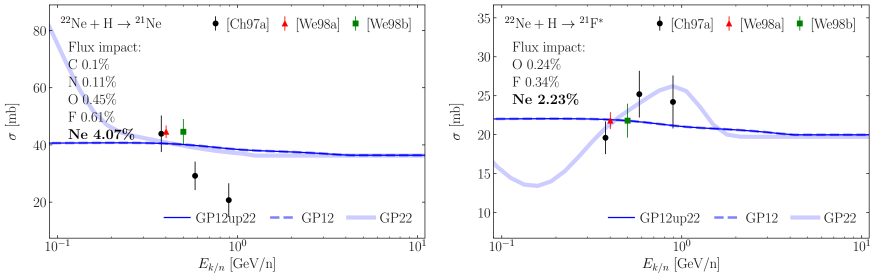


## Z=11 projectiles: $^{x}$Na + H → $^{A}_{Z}X$

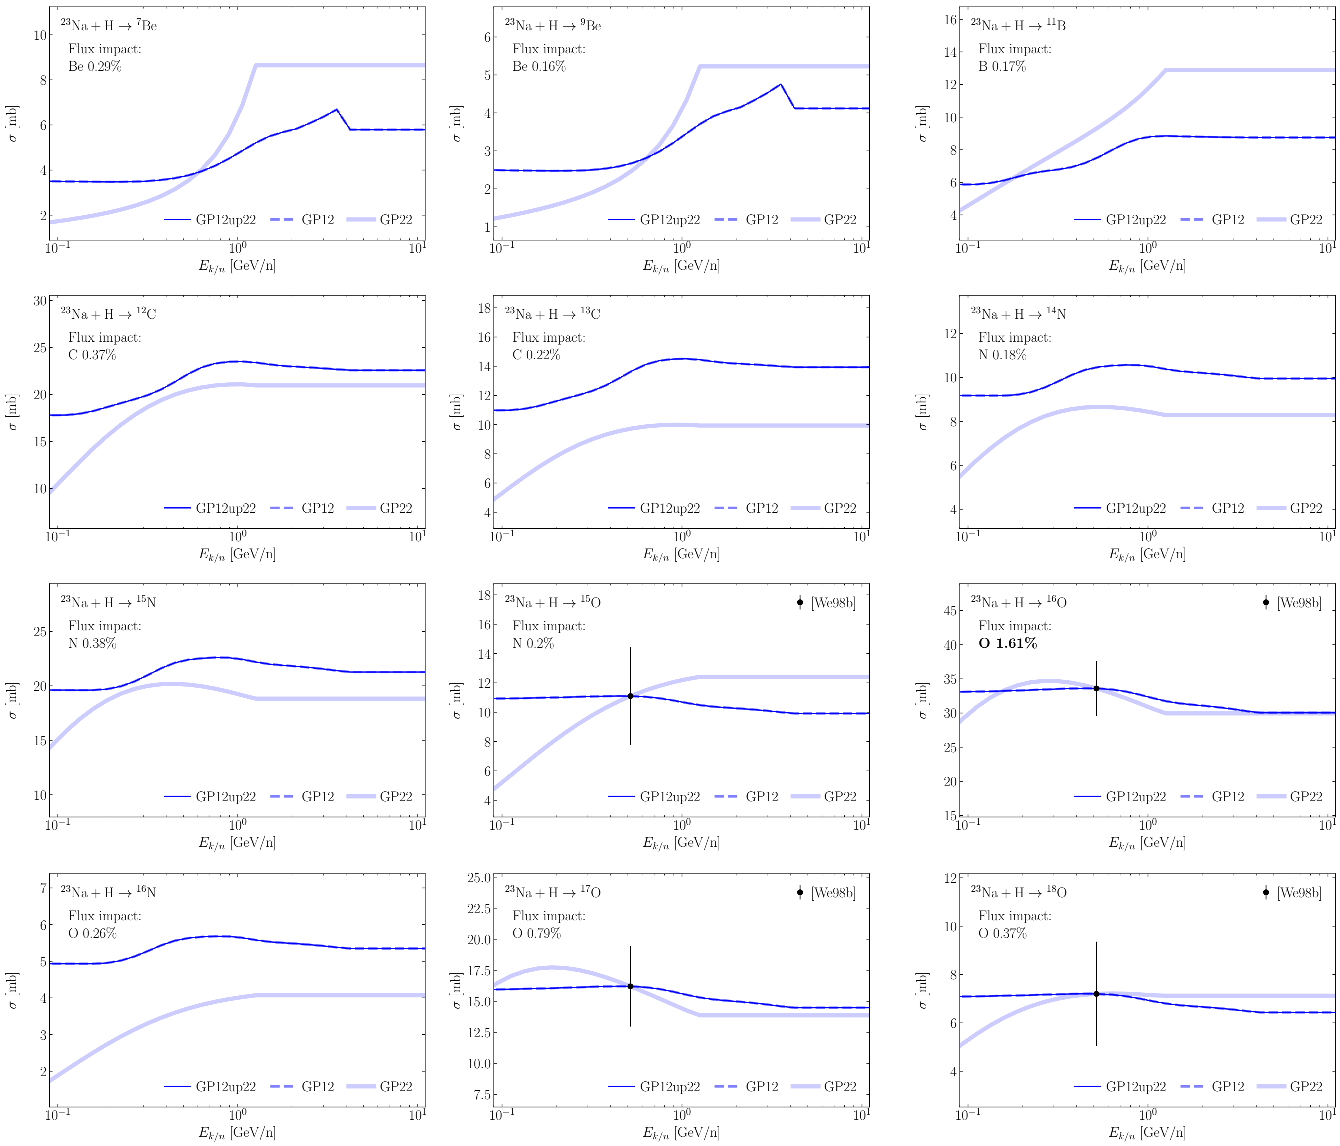

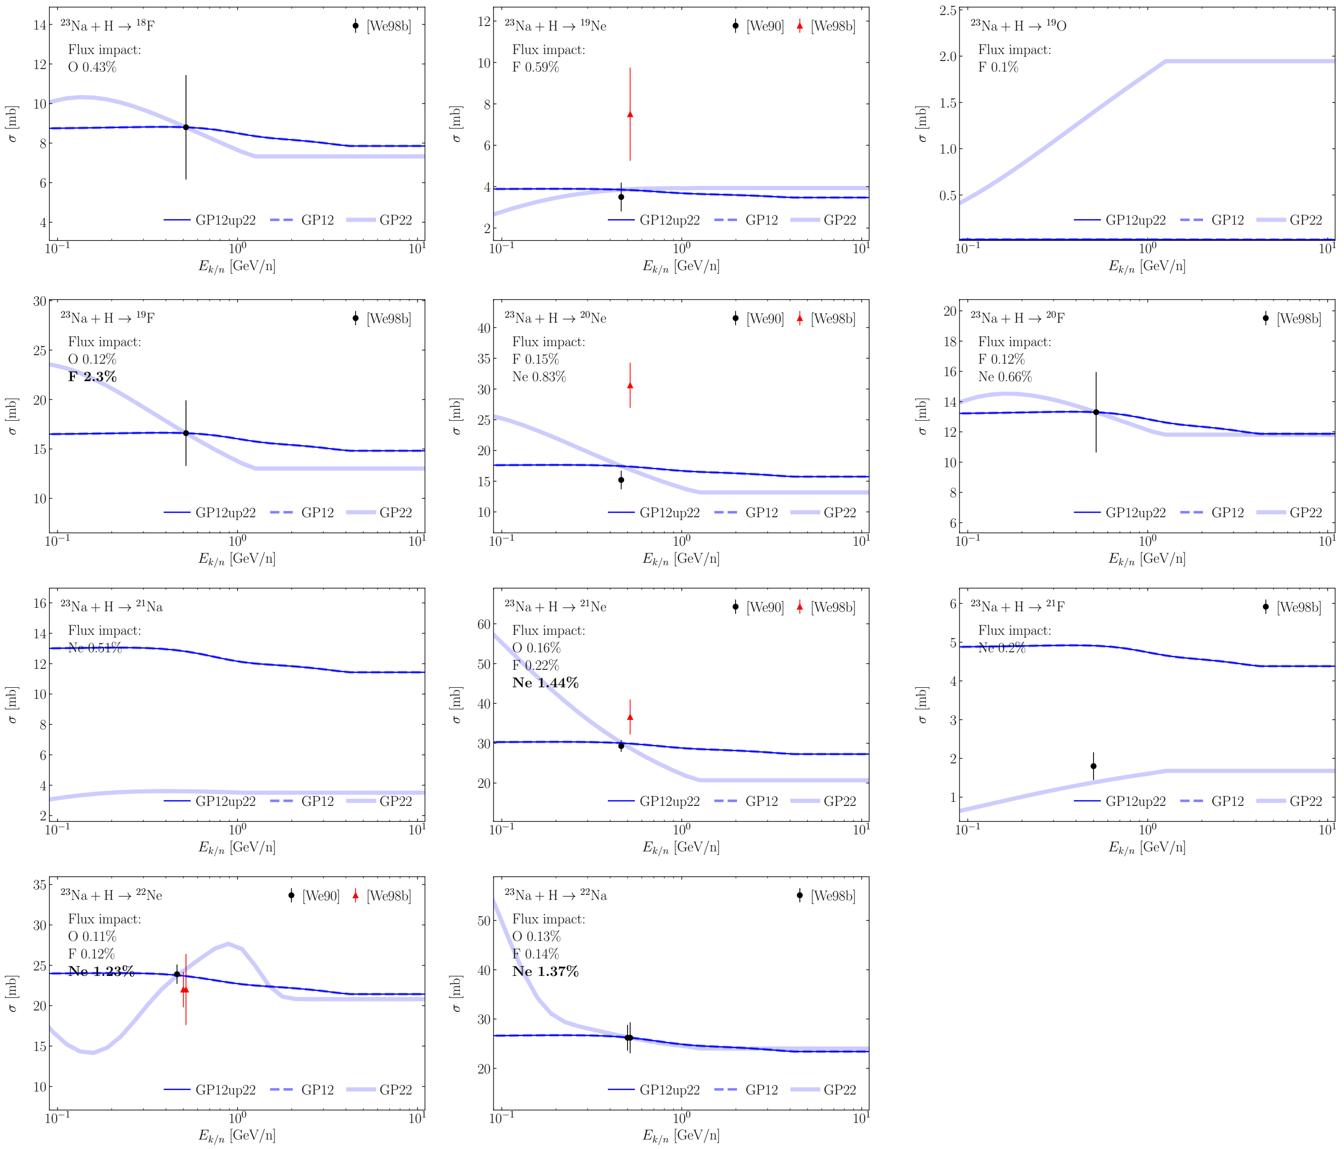


## Z=12 projectiles: $^{x}$Mg + H $\to {}^{A}_{Z}X$

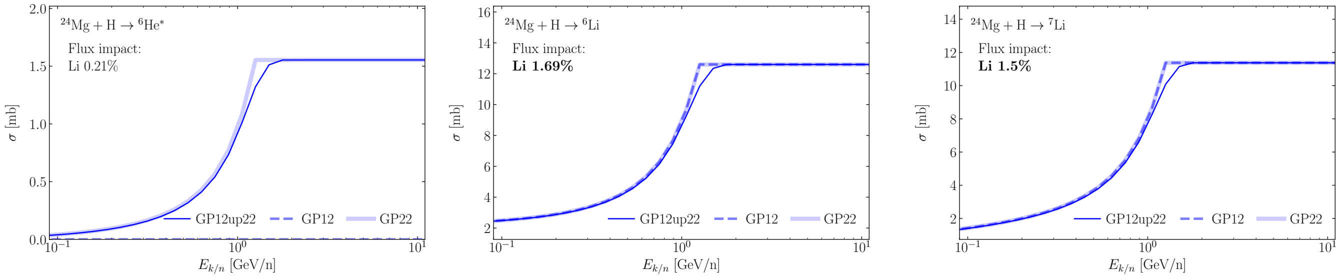

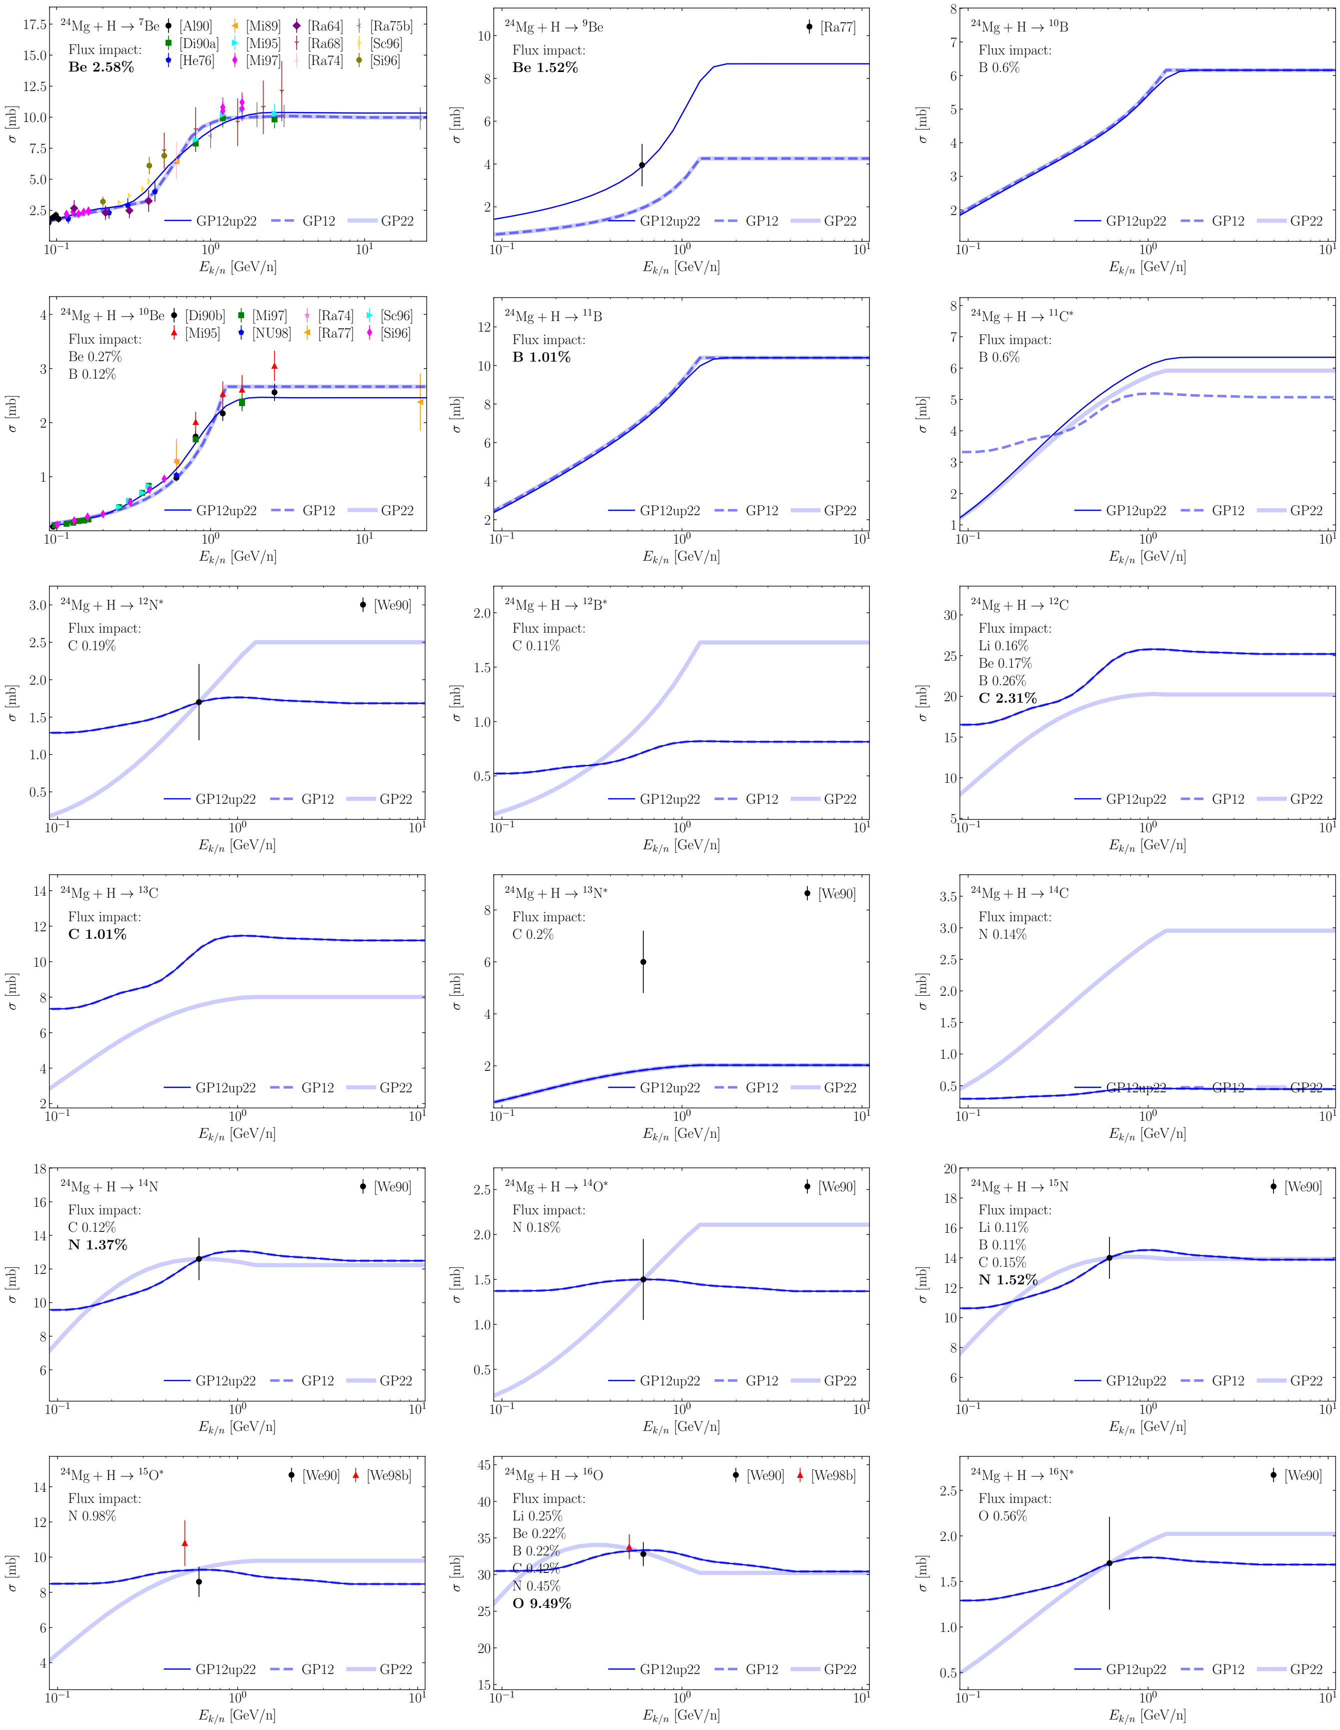

$^{24}$Mg + H → $^{7}$Be
Flux impact:
Be 2.58%
[Al90] [Di90a] [He76] [Mi89] [Mi95] [Mi97] [Ra64] [Ra68] [Ra74] [Ra75b] [Sc96] [Si96]
$^{24}$Mg + H → $^{9}$Be
Flux impact:
Be 1.52%
[Ra77]
$^{24}$Mg + H → $^{10}$B
Flux impact:
B 0.6%
$^{24}$Mg + H → $^{10}$Be
Flux impact:
Be 0.27%
B 0.12%
[Di90b] [Mi95] [Mi97] [NU98] [Ra74] [Ra77] [Sc96] [Si96]
$^{24}$Mg + H → $^{11}$B
Flux impact:
B 1.01%
$^{24}$Mg + H → $^{11}$C*
Flux impact:
B 0.6%
$^{24}$Mg + H → $^{12}$N*
Flux impact:
C 0.19%
[We90]
$^{24}$Mg + H → $^{12}$B*
Flux impact:
C 0.11%
$^{24}$Mg + H → $^{12}$C
Flux impact:
Li 0.16%
Be 0.17%
B 0.26%
C 2.31%
$^{24}$Mg + H → $^{13}$C
Flux impact:
C 1.01%
$^{24}$Mg + H → $^{13}$N*
Flux impact:
C 0.2%
[We90]
$^{24}$Mg + H → $^{14}$C
Flux impact:
N 0.14%
$^{24}$Mg + H → $^{14}$N
Flux impact:
C 0.12%
N 1.37%
[We90]
$^{24}$Mg + H → $^{14}$O*
Flux impact:
N 0.18%
[We90]
$^{24}$Mg + H → $^{15}$N
Flux impact:
Li 0.11%
B 0.11%
C 0.15%
N 1.52%
[We90]
$^{24}$Mg + H → $^{15}$O*
Flux impact:
N 0.98%
[We90] [We98b]
$^{24}$Mg + H → $^{16}$O
Flux impact:
Li 0.25%
Be 0.22%
B 0.22%
C 0.42%
N 0.45%
O 9.49%
[We90] [We98b]
$^{24}$Mg + H → $^{16}$N*
Flux impact:
O 0.56%
[We90]
GP12up22
GP12
GP22
$\sigma$ [mb]
$E_{k/n}$ [GeV/n]

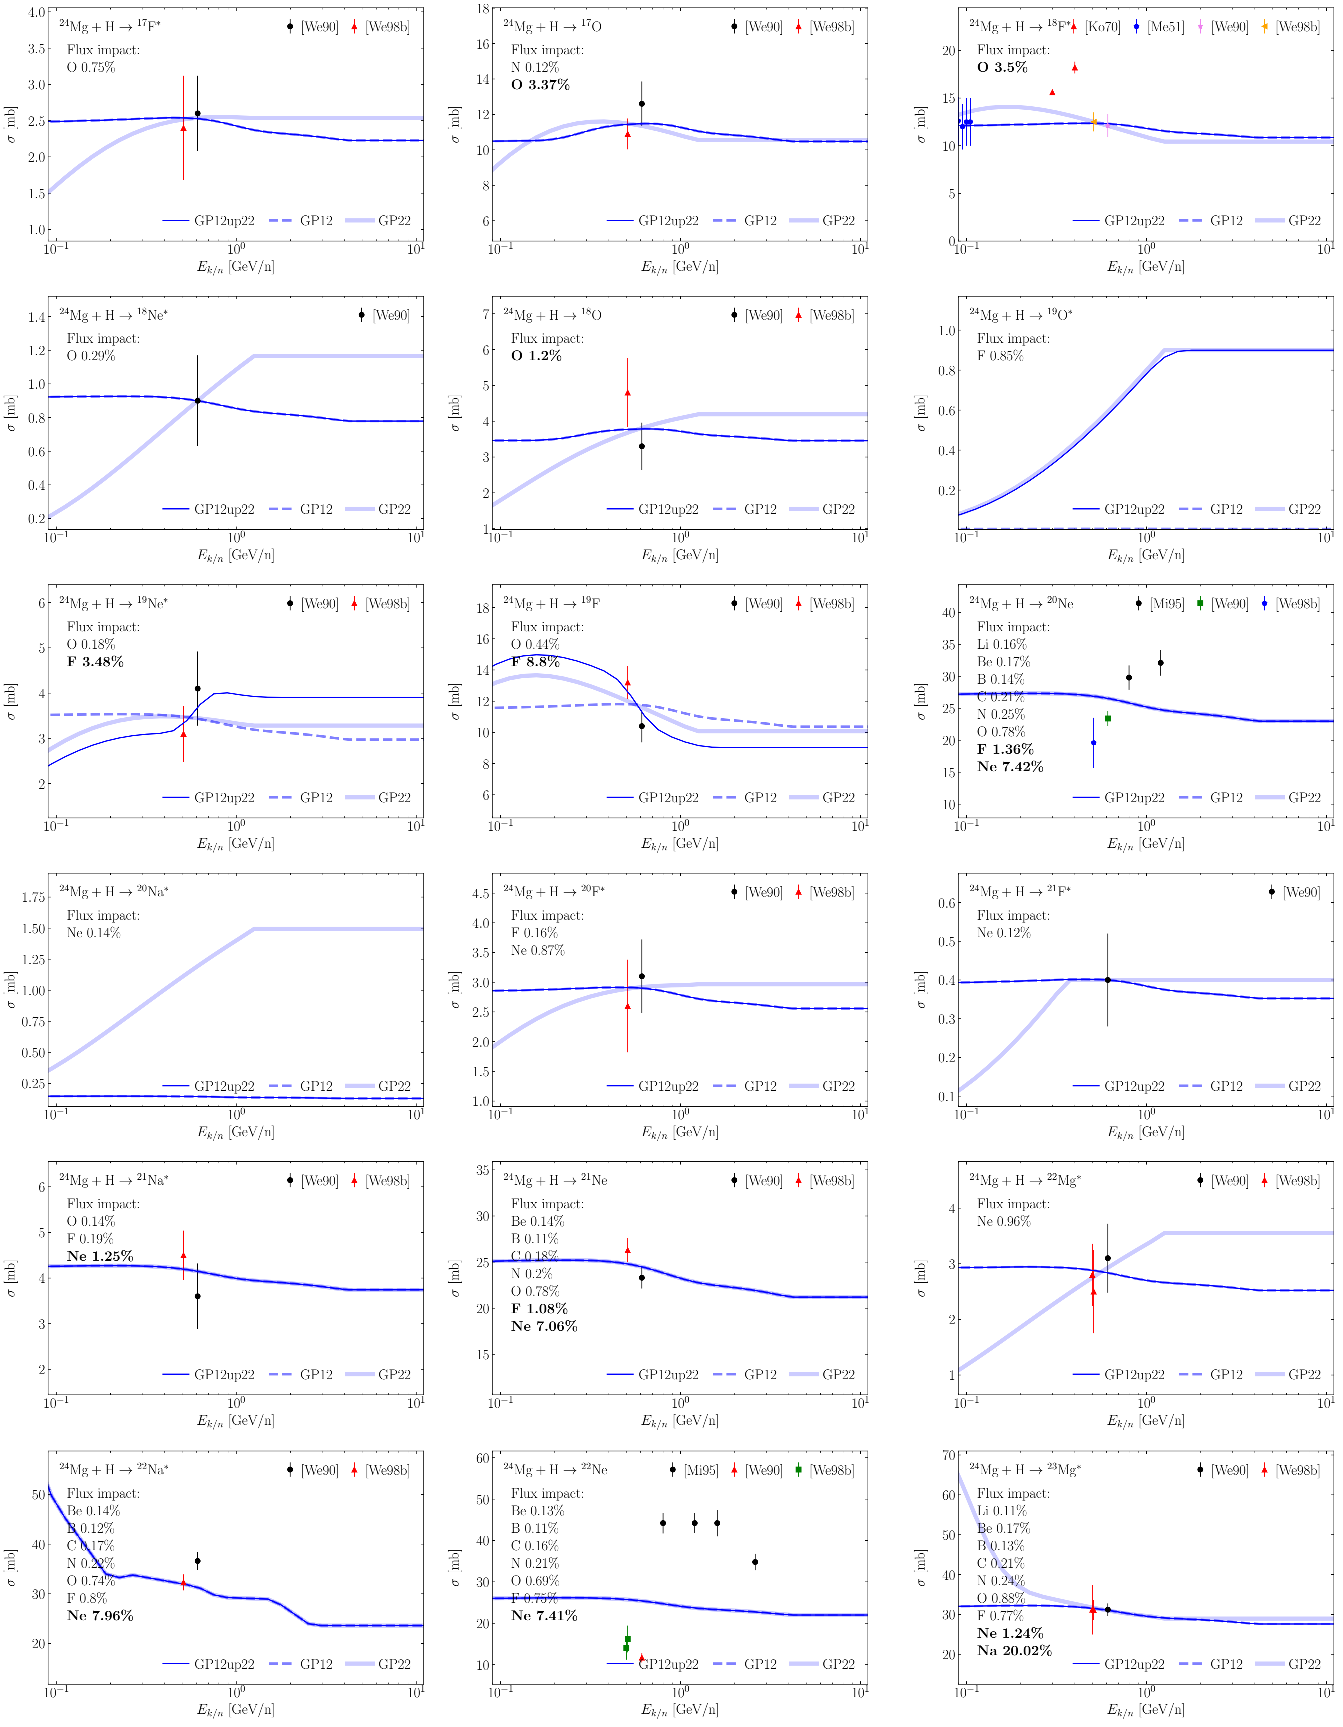

24Mg + H → 17F* [We90] [We98b] Flux impact: O 0.75%
24Mg + H → 17O [We90] [We98b] Flux impact: N 0.12% O 3.37%
24Mg + H → 18F* [Ko70] [Me51] [We90] [We98b] Flux impact: O 3.5%
24Mg + H → 18Ne* [We90] Flux impact: O 0.29%
24Mg + H → 18O [We90] [We98b] Flux impact: O 1.2%
24Mg + H → 19O* Flux impact: F 0.85%
24Mg + H → 19Ne* [We90] [We98b] Flux impact: O 0.18% F 3.48%
24Mg + H → 19F [We90] [We98b] Flux impact: O 0.44% F 8.8%
24Mg + H → 20Ne [Mi95] [We90] [We98b] Flux impact: Li 0.16% Be 0.17% B 0.14% C 0.21% N 0.25% O 0.78% F 1.36% Ne 7.42%
24Mg + H → 20Na* Flux impact: Ne 0.14%
24Mg + H → 20F* [We90] [We98b] Flux impact: F 0.16% Ne 0.87%
24Mg + H → 21F* [We90] Flux impact: Ne 0.12%
24Mg + H → 21Na* [We90] [We98b] Flux impact: O 0.14% F 0.19% Ne 1.25%
24Mg + H → 21Ne [We90] [We98b] Flux impact: Be 0.14% B 0.11% C 0.18% N 0.2% O 0.78% F 1.08% Ne 7.06%
24Mg + H → 22Mg* [We90] [We98b] Flux impact: Ne 0.96%
24Mg + H → 22Na* [We90] [We98b] Flux impact: Be 0.14% B 0.12% C 0.17% N 0.22% O 0.74% F 0.8% Ne 7.96%
24Mg + H → 22Ne [Mi95] [We90] [We98b] Flux impact: Be 0.13% B 0.11% C 0.16% N 0.21% O 0.69% F 0.75% Ne 7.41%
24Mg + H → 23Mg* [We90] [We98b] Flux impact: Li 0.11% Be 0.17% B 0.13% C 0.21% N 0.24% O 0.88% F 0.77% Ne 1.24% Na 20.02%
GP12up22 GP12 GP22
σ [mb]
Ek/n [GeV/n]

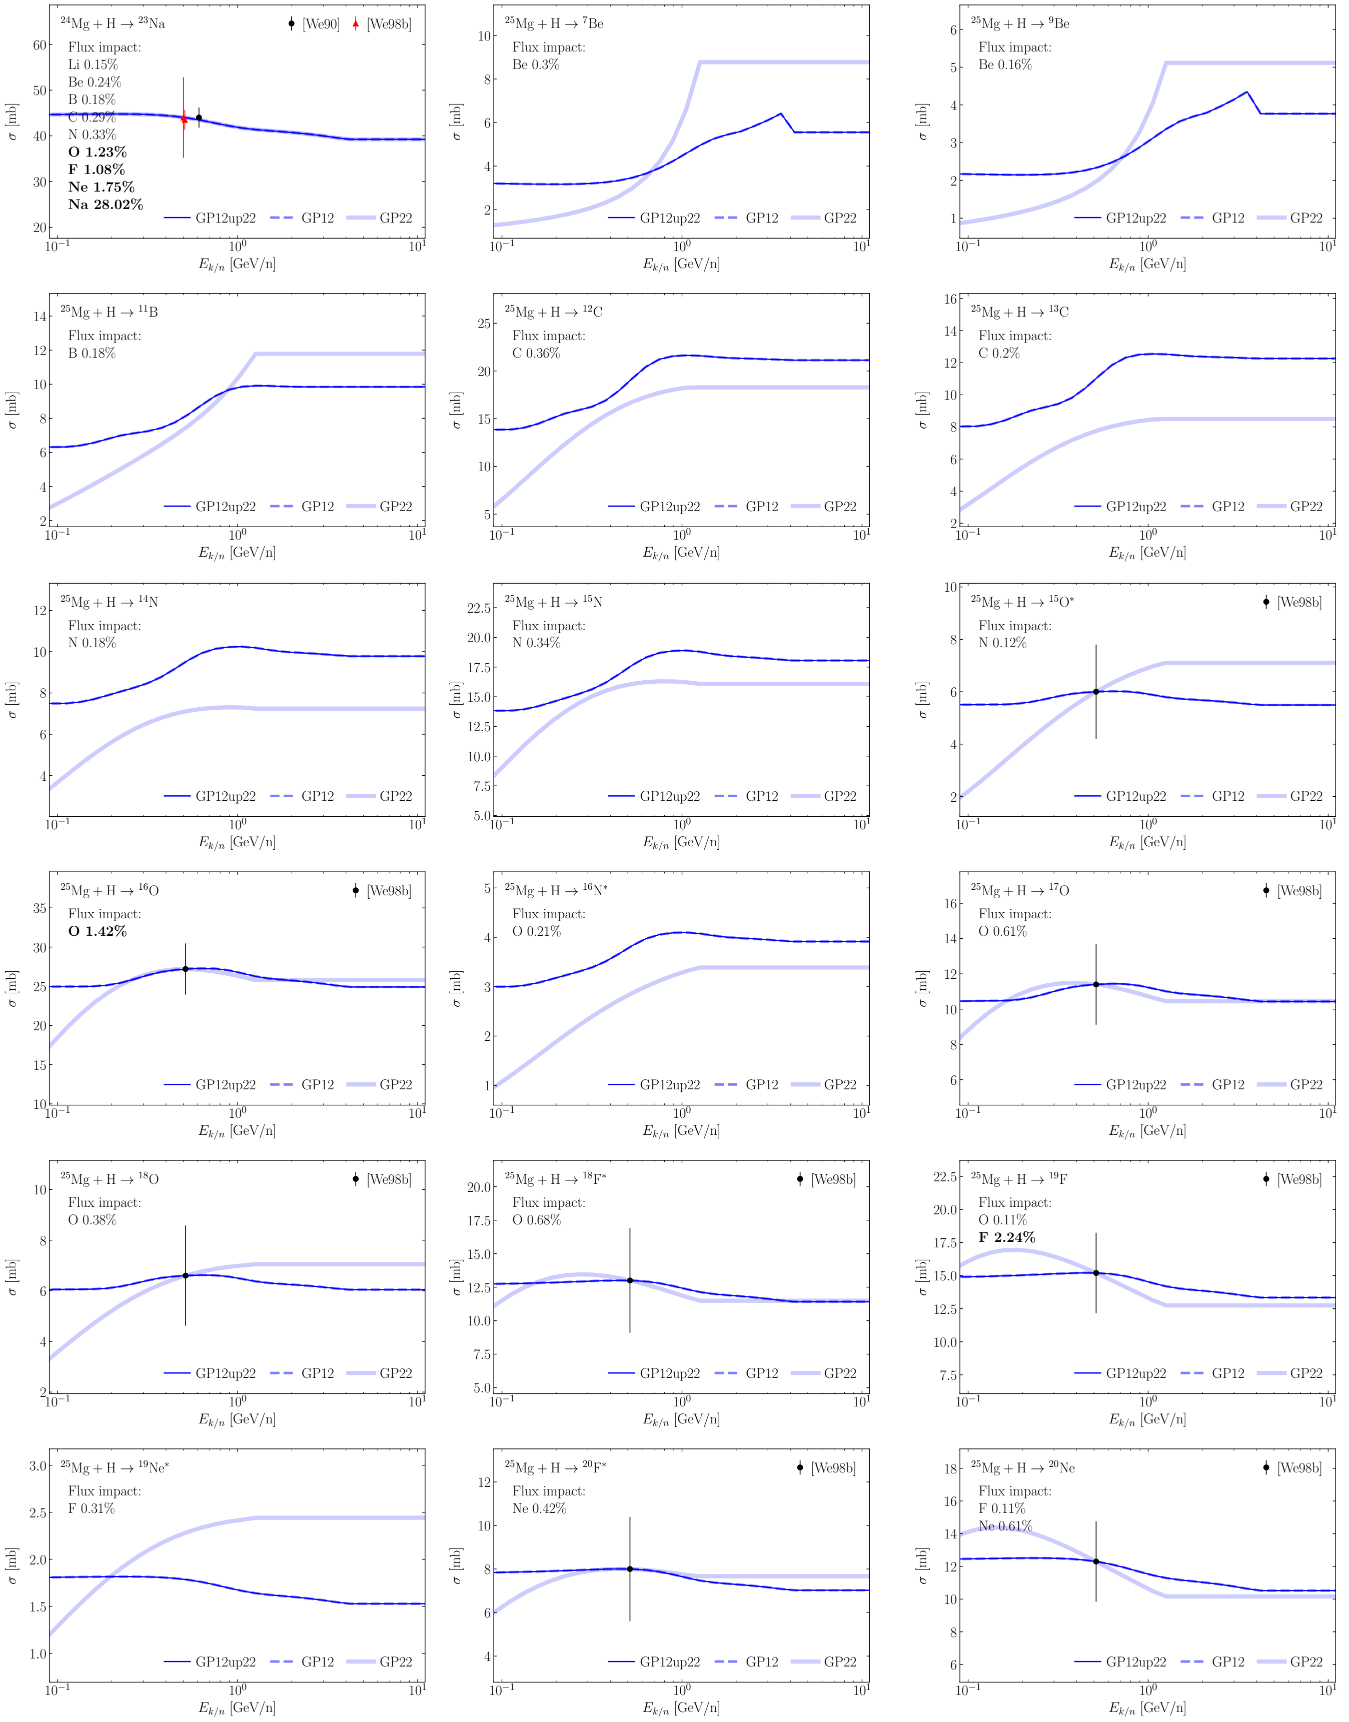
$^{24}Mg + H \to ^{23}Na$
[We90] [We98b]
Flux impact:
Li 0.15%
Be 0.24%
B 0.18%
C 0.29%
N 0.33%
O 1.23%
F 1.08%
Ne 1.75%
Na 28.02%
$^{25}Mg + H \to ^{7}Be$
Flux impact:
Be 0.3%
$^{25}Mg + H \to ^{9}Be$
Flux impact:
Be 0.16%
$^{25}Mg + H \to ^{11}B$
Flux impact:
B 0.18%
$^{25}Mg + H \to ^{12}C$
Flux impact:
C 0.36%
$^{25}Mg + H \to ^{13}C$
Flux impact:
C 0.2%
$^{25}Mg + H \to ^{14}N$
Flux impact:
N 0.18%
$^{25}Mg + H \to ^{15}N$
Flux impact:
N 0.34%
$^{25}Mg + H \to ^{15}O^*$
[We98b]
Flux impact:
N 0.12%
$^{25}Mg + H \to ^{16}O$
[We98b]
Flux impact:
O 1.42%
$^{25}Mg + H \to ^{16}N^*$
Flux impact:
O 0.21%
$^{25}Mg + H \to ^{17}O$
[We98b]
Flux impact:
O 0.61%
$^{25}Mg + H \to ^{18}O$
[We98b]
Flux impact:
O 0.38%
$^{25}Mg + H \to ^{18}F^*$
[We98b]
Flux impact:
O 0.68%
$^{25}Mg + H \to ^{19}F$
[We98b]
Flux impact:
O 0.11%
F 2.24%
$^{25}Mg + H \to ^{19}Ne^*$
Flux impact:
F 0.31%
$^{25}Mg + H \to ^{20}F^*$
[We98b]
Flux impact:
Ne 0.42%
$^{25}Mg + H \to ^{20}Ne$
[We98b]
Flux impact:
F 0.11%
Ne 0.61%
GP12up22
GP12
GP22
$\sigma$ [mb]
$E_{k/n}$ [GeV/n]

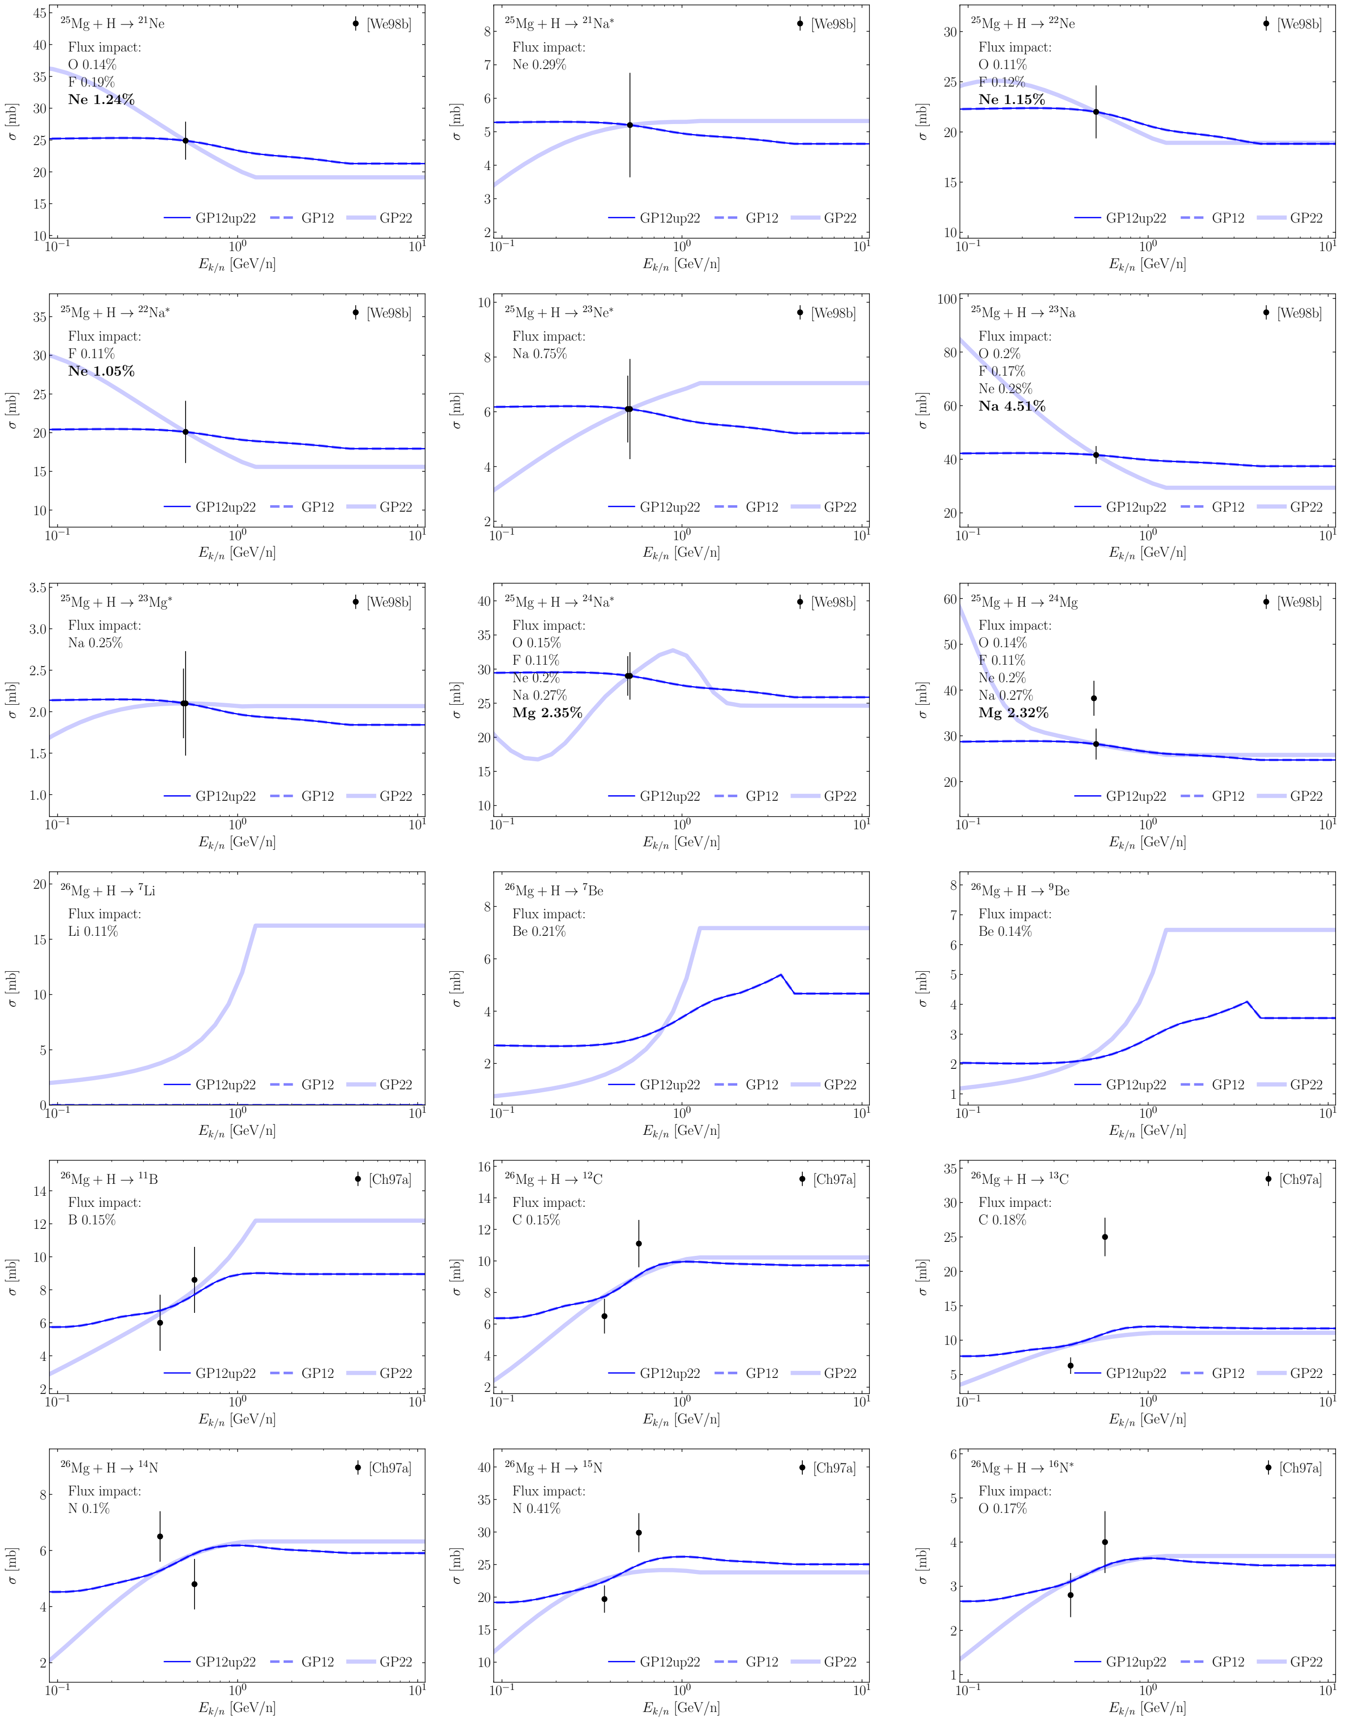
$^{25}$Mg + H → $^{21}$Ne
[We98b]
Flux impact:
O 0.14%
F 0.19%
**Ne 1.24%**
$^{25}$Mg + H → $^{21}$Na*
[We98b]
Flux impact:
Ne 0.29%
$^{25}$Mg + H → $^{22}$Ne
[We98b]
Flux impact:
O 0.11%
F 0.12%
**Ne 1.15%**
$^{25}$Mg + H → $^{22}$Na*
[We98b]
Flux impact:
F 0.11%
**Ne 1.05%**
$^{25}$Mg + H → $^{23}$Ne*
[We98b]
Flux impact:
Na 0.75%
$^{25}$Mg + H → $^{23}$Na
[We98b]
Flux impact:
O 0.2%
F 0.17%
Ne 0.28%
**Na 4.51%**
$^{25}$Mg + H → $^{23}$Mg*
[We98b]
Flux impact:
Na 0.25%
$^{25}$Mg + H → $^{24}$Na*
[We98b]
Flux impact:
O 0.15%
F 0.11%
Ne 0.2%
Na 0.27%
**Mg 2.35%**
$^{25}$Mg + H → $^{24}$Mg
[We98b]
Flux impact:
O 0.14%
F 0.11%
Ne 0.2%
Na 0.27%
**Mg 2.32%**
$^{26}$Mg + H → $^{7}$Li
Flux impact:
Li 0.11%
$^{26}$Mg + H → $^{7}$Be
Flux impact:
Be 0.21%
$^{26}$Mg + H → $^{9}$Be
Flux impact:
Be 0.14%
$^{26}$Mg + H → $^{11}$B
[Ch97a]
Flux impact:
B 0.15%
$^{26}$Mg + H → $^{12}$C
[Ch97a]
Flux impact:
C 0.15%
$^{26}$Mg + H → $^{13}$C
[Ch97a]
Flux impact:
C 0.18%
$^{26}$Mg + H → $^{14}$N
[Ch97a]
Flux impact:
N 0.1%
$^{26}$Mg + H → $^{15}$N
[Ch97a]
Flux impact:
N 0.41%
$^{26}$Mg + H → $^{16}$N*
[Ch97a]
Flux impact:
O 0.17%
GP12up22
GP12
GP22
$\sigma$ [mb]
$E_{k/n}$ [GeV/n]

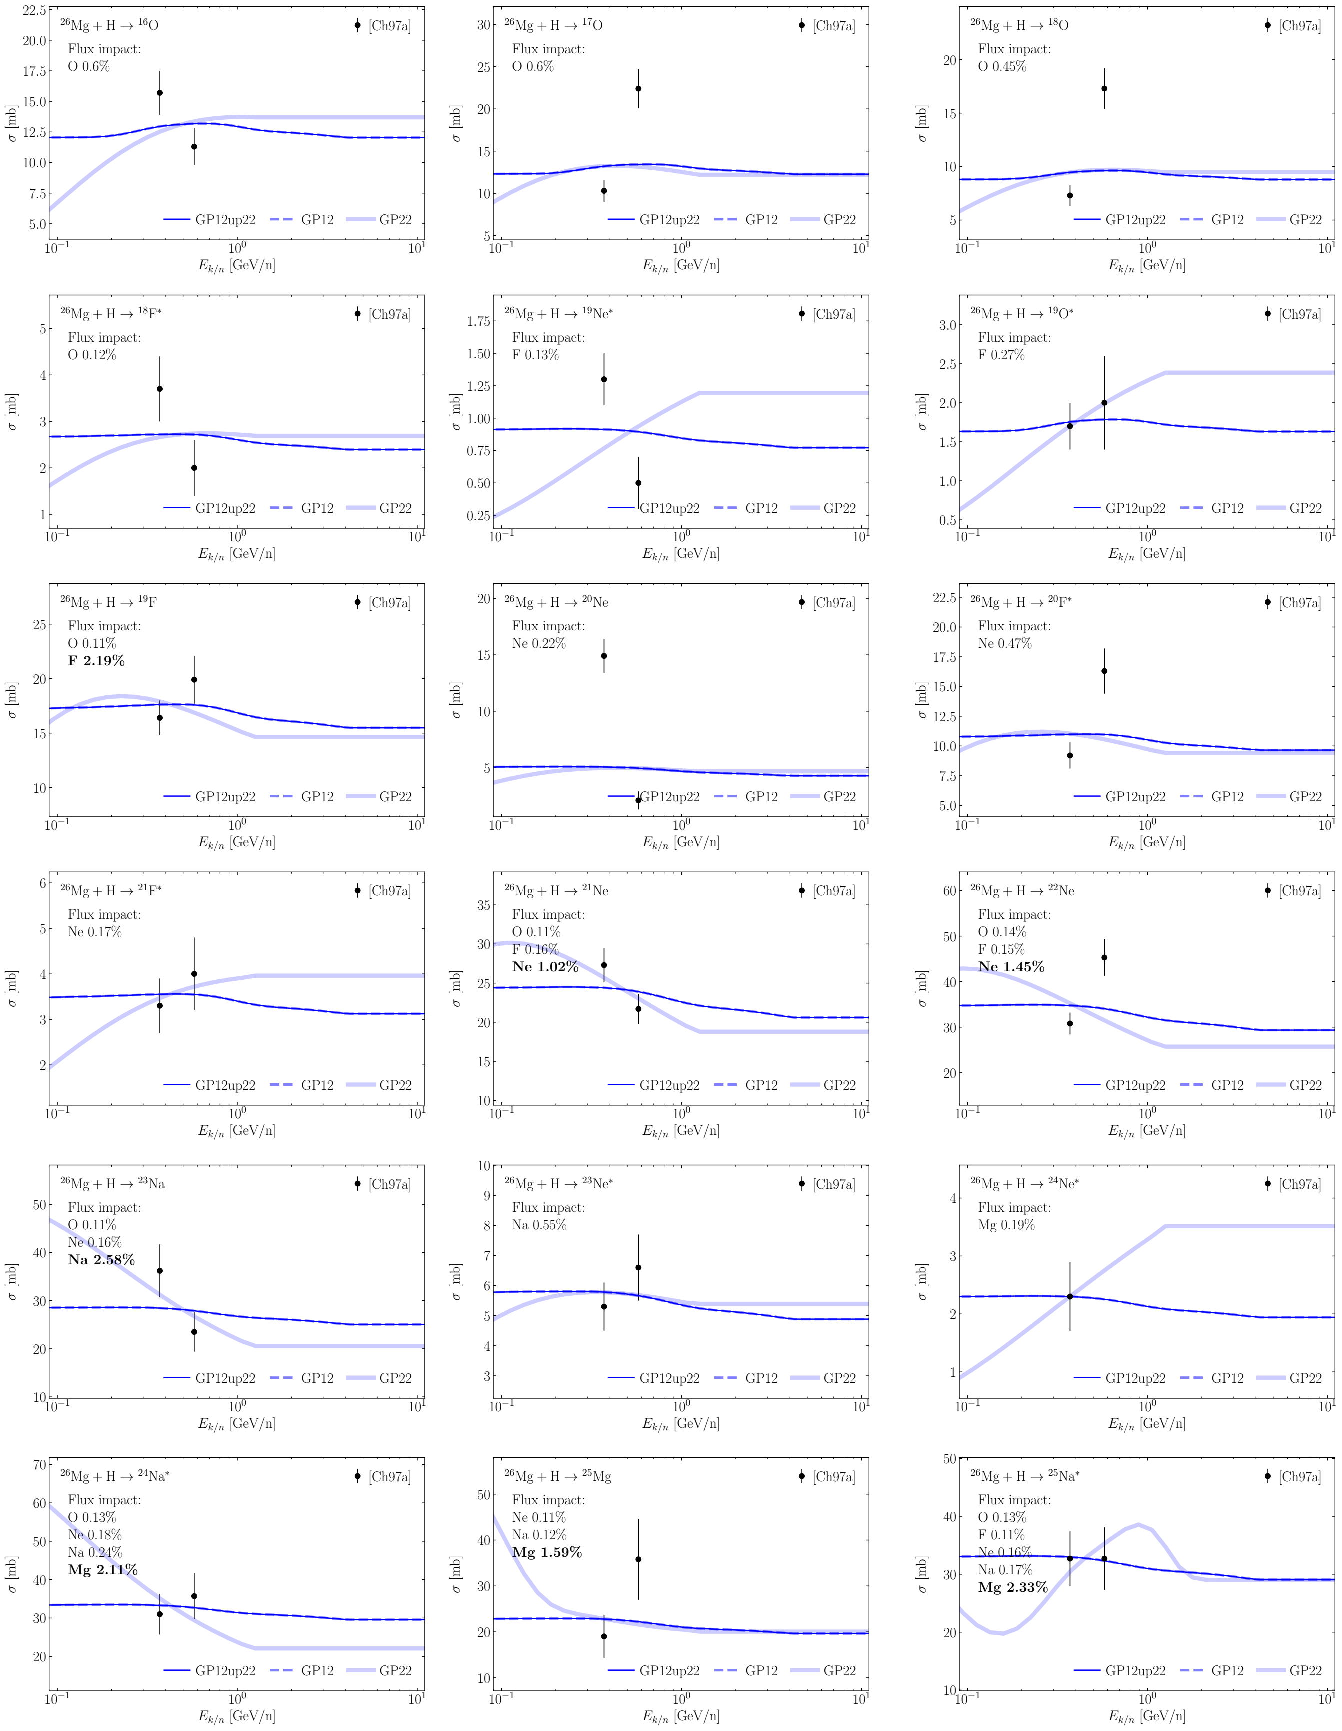

$^{26}$Mg + H → $^{16}$O
[Ch97a]
Flux impact:
O 0.6%
$^{26}$Mg + H → $^{17}$O
[Ch97a]
Flux impact:
O 0.6%
$^{26}$Mg + H → $^{18}$O
[Ch97a]
Flux impact:
O 0.45%
$^{26}$Mg + H → $^{18}$F*
[Ch97a]
Flux impact:
O 0.12%
$^{26}$Mg + H → $^{19}$Ne*
[Ch97a]
Flux impact:
F 0.13%
$^{26}$Mg + H → $^{19}$O*
[Ch97a]
Flux impact:
F 0.27%
$^{26}$Mg + H → $^{19}$F
[Ch97a]
Flux impact:
O 0.11%
F 2.19%
$^{26}$Mg + H → $^{20}$Ne
[Ch97a]
Flux impact:
Ne 0.22%
$^{26}$Mg + H → $^{20}$F*
[Ch97a]
Flux impact:
Ne 0.47%
$^{26}$Mg + H → $^{21}$F*
[Ch97a]
Flux impact:
Ne 0.17%
$^{26}$Mg + H → $^{21}$Ne
[Ch97a]
Flux impact:
O 0.11%
F 0.16%
Ne 1.02%
$^{26}$Mg + H → $^{22}$Ne
[Ch97a]
Flux impact:
O 0.14%
F 0.15%
Ne 1.45%
$^{26}$Mg + H → $^{23}$Na
[Ch97a]
Flux impact:
O 0.11%
Ne 0.16%
Na 2.58%
$^{26}$Mg + H → $^{23}$Ne*
[Ch97a]
Flux impact:
Na 0.55%
$^{26}$Mg + H → $^{24}$Ne*
[Ch97a]
Flux impact:
Mg 0.19%
$^{26}$Mg + H → $^{24}$Na*
[Ch97a]
Flux impact:
O 0.13%
Ne 0.18%
Na 0.24%
Mg 2.11%
$^{26}$Mg + H → $^{25}$Mg
[Ch97a]
Flux impact:
Ne 0.11%
Na 0.12%
Mg 1.59%
$^{26}$Mg + H → $^{25}$Na*
[Ch97a]
Flux impact:
O 0.13%
F 0.11%
Ne 0.16%
Na 0.17%
Mg 2.33%
GP12up22
GP12
GP22
$\sigma$ [mb]
$E_{k/n}$ [GeV/n]

## Z=13 projectiles: $^{x}$Al + H → $^{A}_{Z}X$

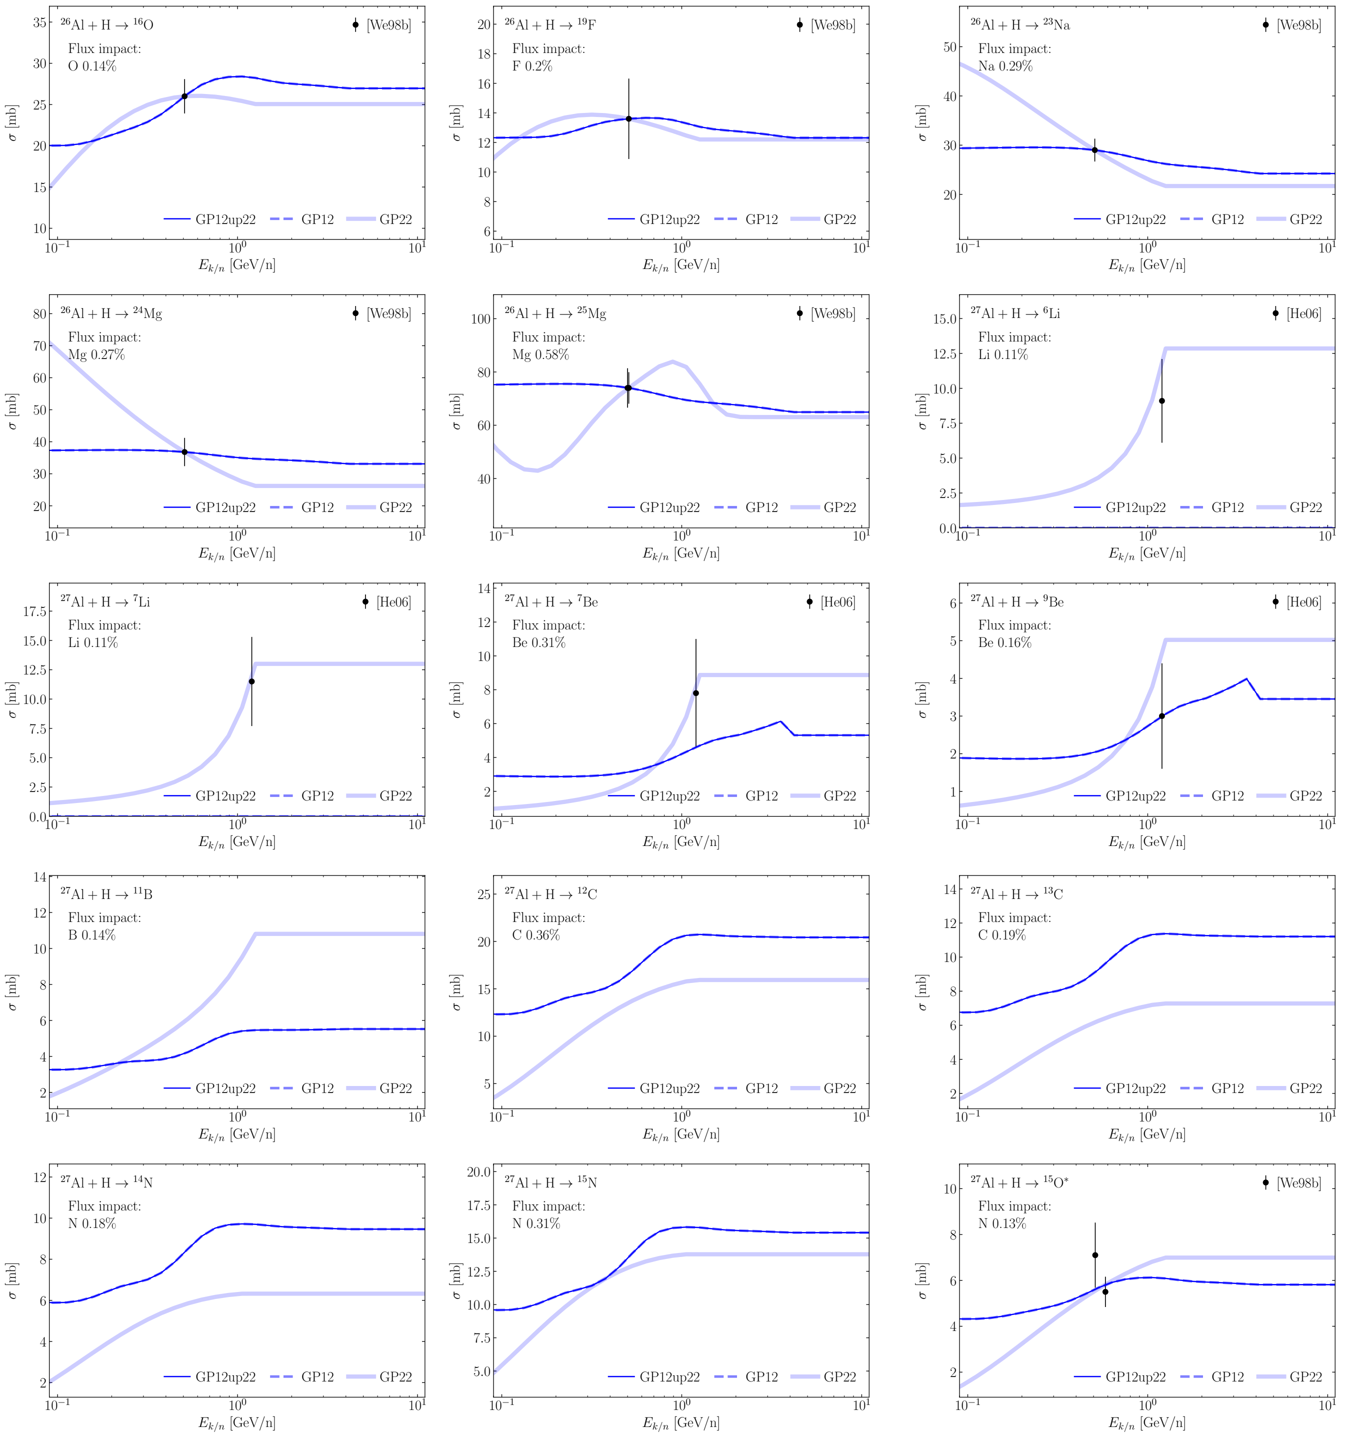

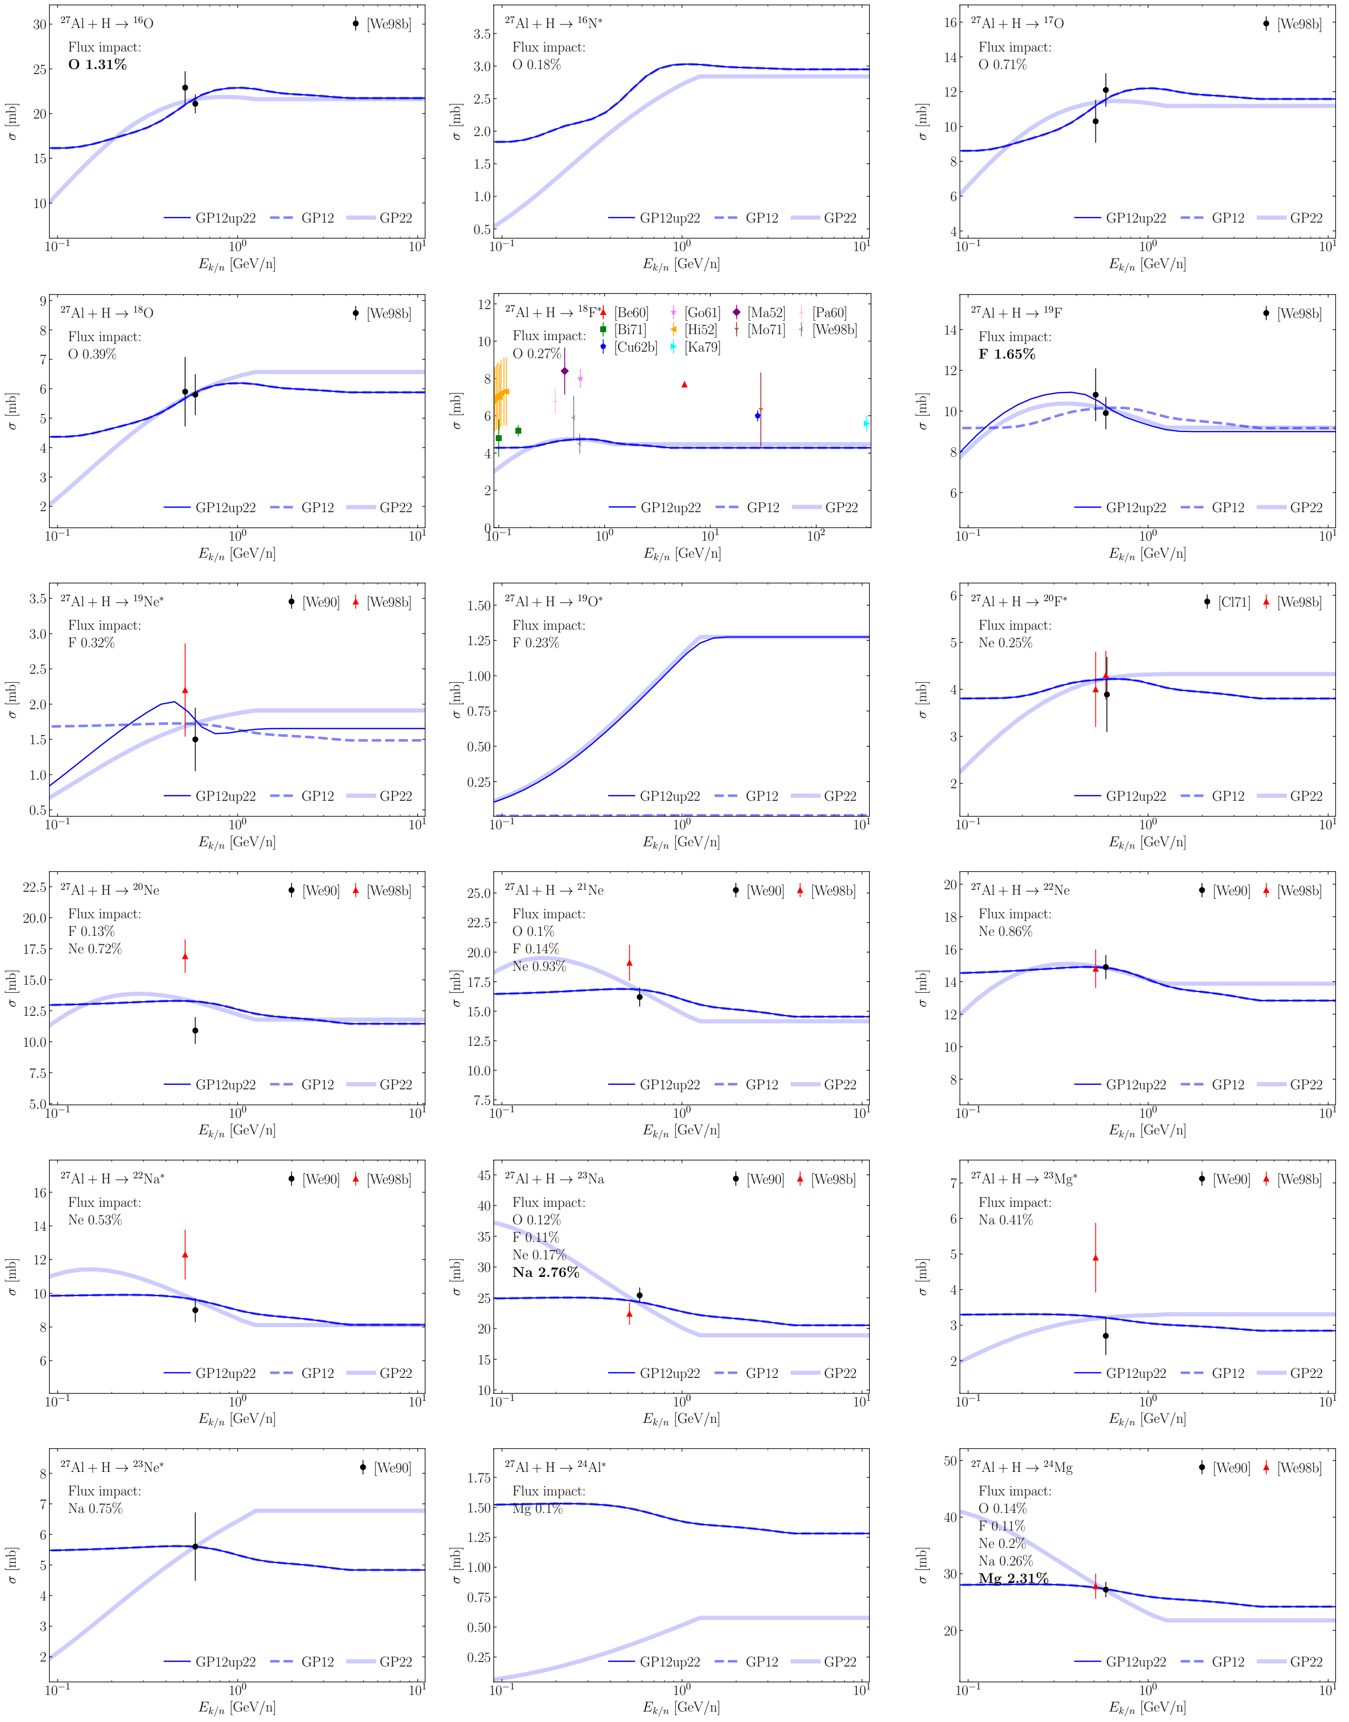
27Al + H → 16O
[We98b]
Flux impact:
O 1.31%
27Al + H → 16N*
Flux impact:
O 0.18%
27Al + H → 17O
[We98b]
Flux impact:
O 0.71%
27Al + H → 18O
[We98b]
Flux impact:
O 0.39%
27Al + H → 18F*
[Be60] [Go61] [Ma52] [Pa60] [Bi71] [Hi52] [Mo71] [We98b] [Cu62b] [Ka79]
Flux impact:
O 0.27%
27Al + H → 19F
[We98b]
Flux impact:
F 1.65%
27Al + H → 19Ne*
[We90] [We98b]
Flux impact:
F 0.32%
27Al + H → 19O*
Flux impact:
F 0.23%
27Al + H → 20F*
[Cl71] [We98b]
Flux impact:
Ne 0.25%
27Al + H → 20Ne
[We90] [We98b]
Flux impact:
F 0.13%
Ne 0.72%
27Al + H → 21Ne
[We90] [We98b]
Flux impact:
O 0.1%
F 0.14%
Ne 0.93%
27Al + H → 22Ne
[We90] [We98b]
Flux impact:
Ne 0.86%
27Al + H → 22Na*
[We90] [We98b]
Flux impact:
Ne 0.53%
27Al + H → 23Na
[We90] [We98b]
Flux impact:
O 0.12%
F 0.11%
Ne 0.17%
Na 2.76%
27Al + H → 23Mg*
[We90] [We98b]
Flux impact:
Na 0.41%
27Al + H → 23Ne*
[We90]
Flux impact:
Na 0.75%
27Al + H → 24Al*
Flux impact:
Mg 0.1%
27Al + H → 24Mg
[We90] [We98b]
Flux impact:
O 0.14%
F 0.11%
Ne 0.2%
Na 0.26%
Mg 2.31%
GP12up22
GP12
GP22
σ [mb]
Ek/n [GeV/n]

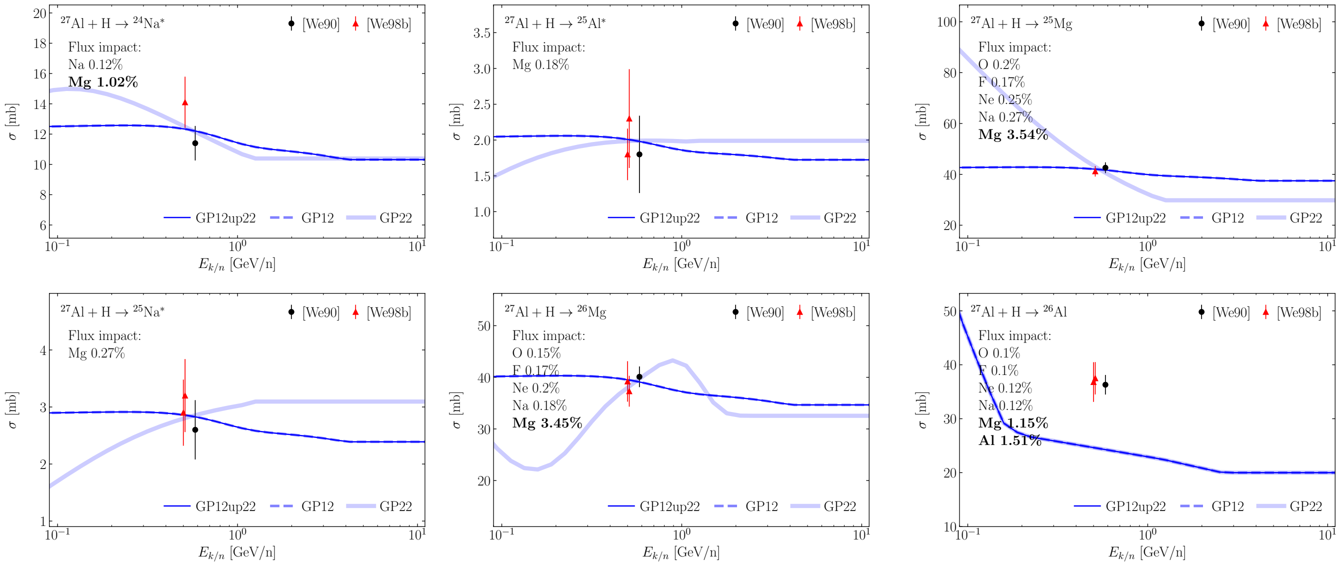


## Z=14 projectiles: $^{x}$Si + H → $^{A}_{Z}X$

---

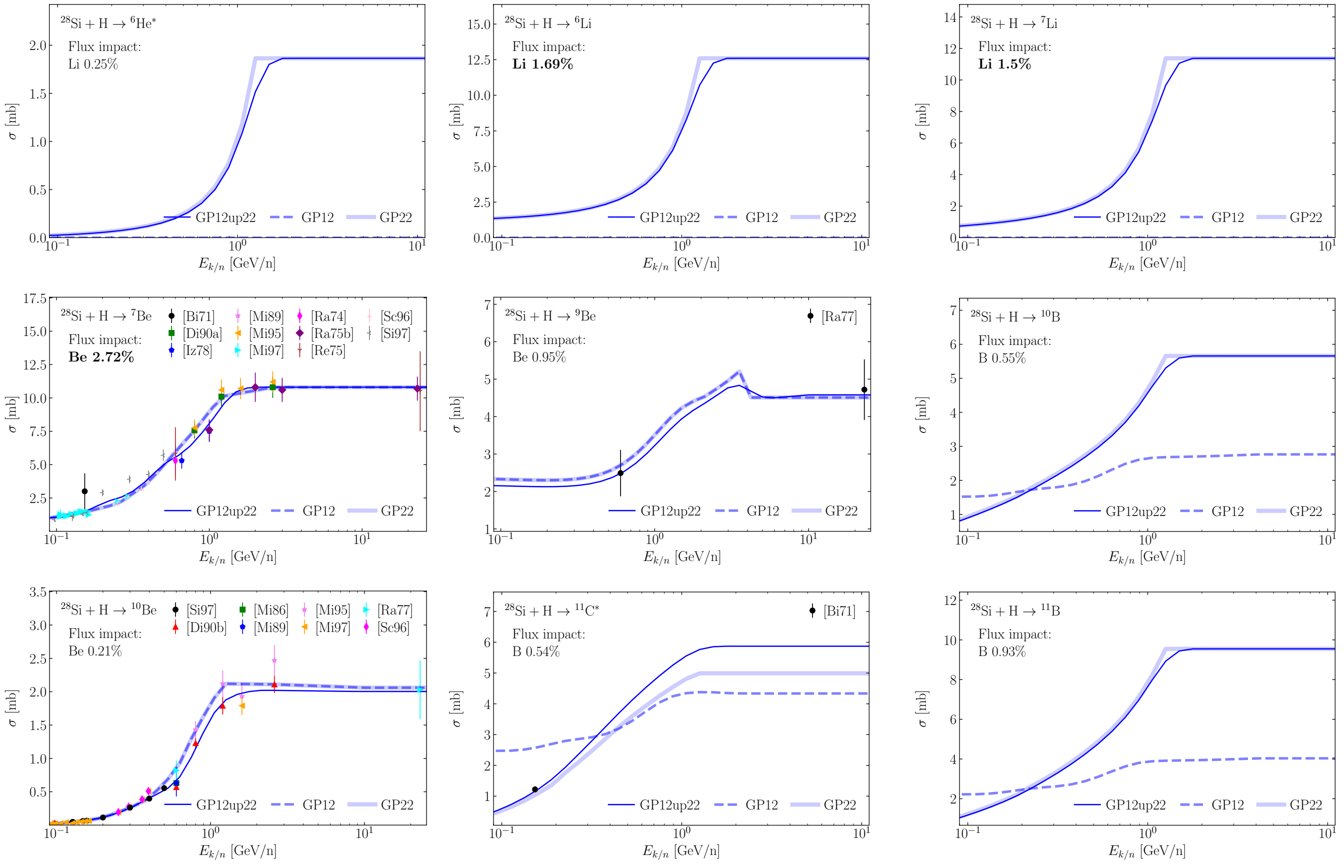

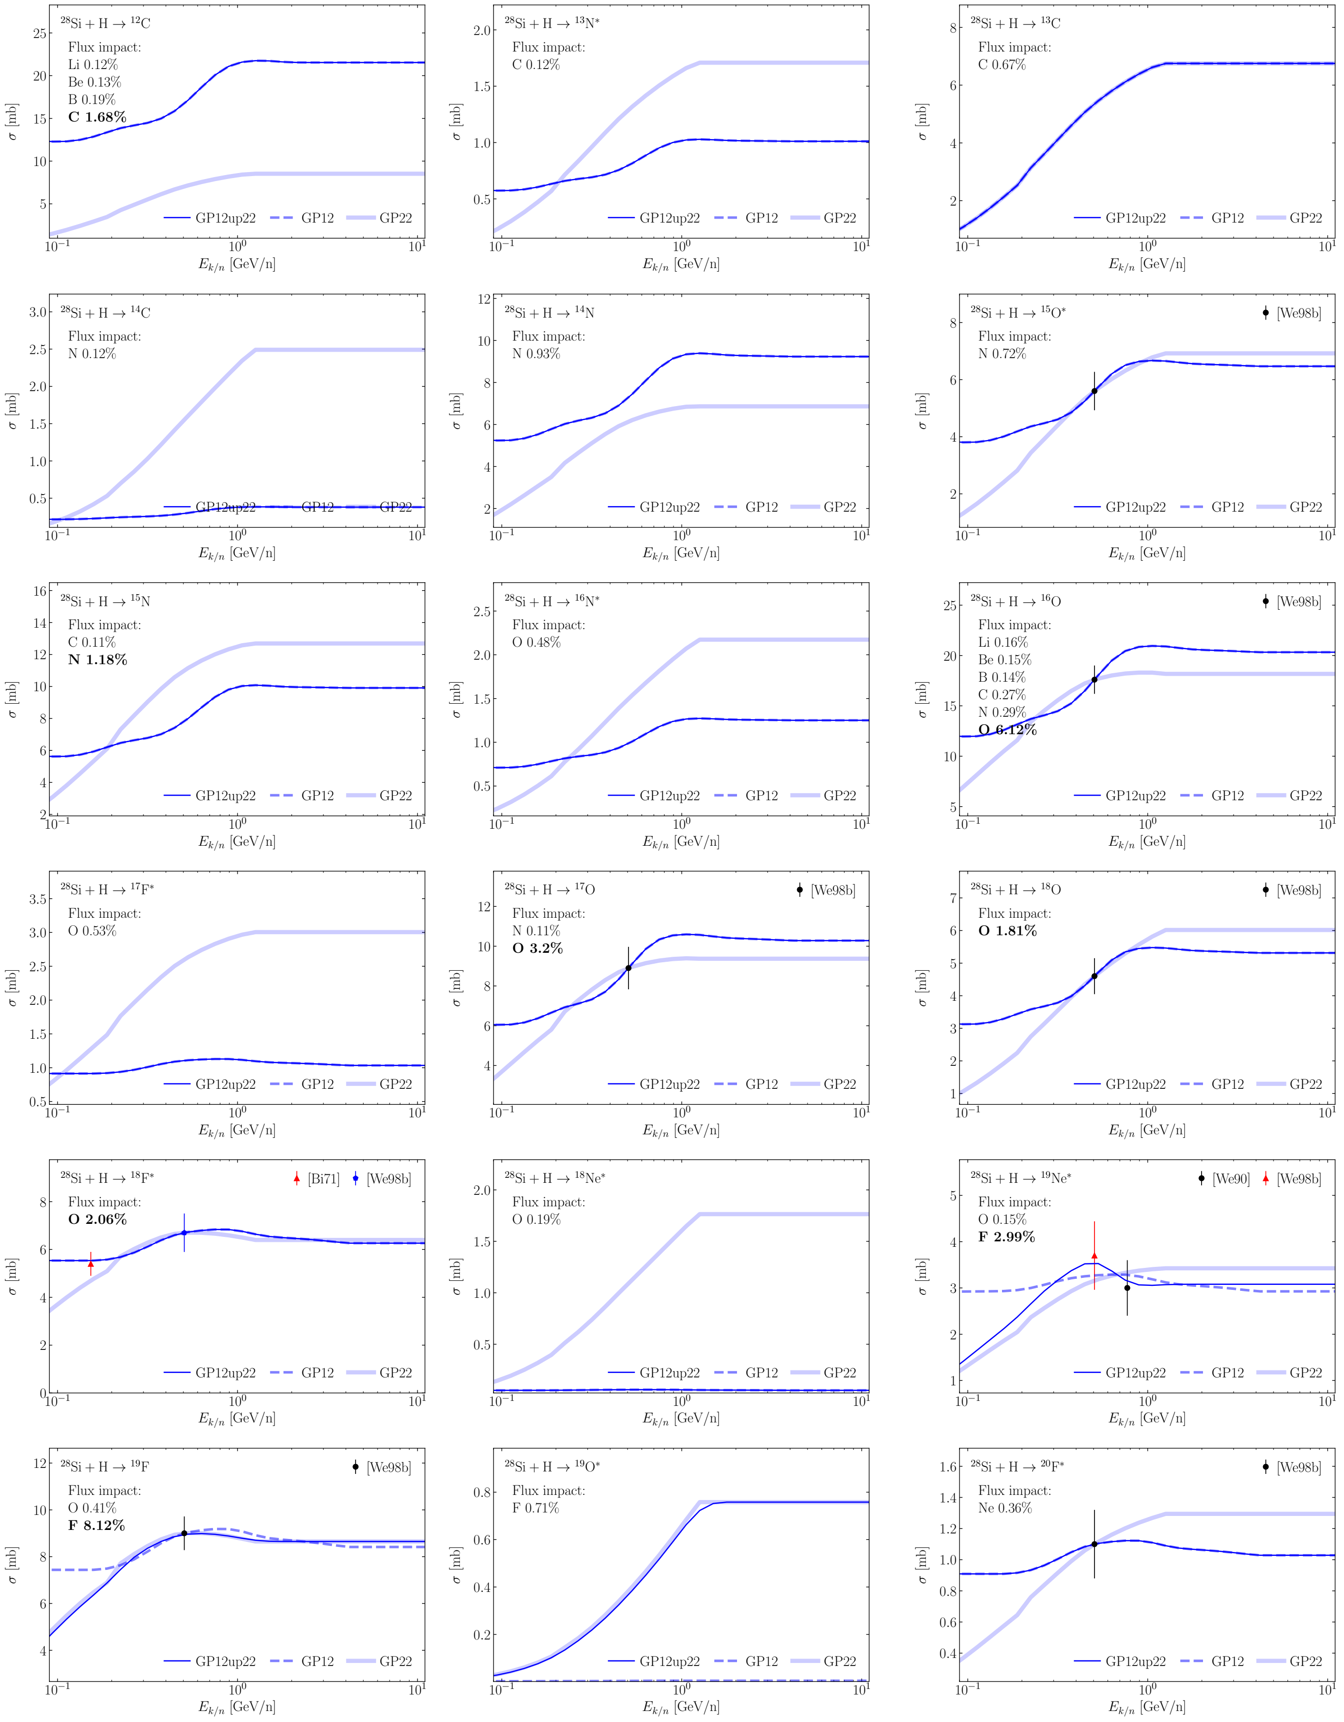

$^{28}$Si + H → $^{12}$C
Flux impact:
Li 0.12%
Be 0.13%
B 0.19%
**C 1.68%**
$^{28}$Si + H → $^{13}$N*
Flux impact:
C 0.12%
$^{28}$Si + H → $^{13}$C
Flux impact:
C 0.67%
$^{28}$Si + H → $^{14}$C
Flux impact:
N 0.12%
$^{28}$Si + H → $^{14}$N
Flux impact:
N 0.93%
$^{28}$Si + H → $^{15}$O*
[We98b]
Flux impact:
N 0.72%
$^{28}$Si + H → $^{15}$N
Flux impact:
C 0.11%
**N 1.18%**
$^{28}$Si + H → $^{16}$N*
Flux impact:
O 0.48%
$^{28}$Si + H → $^{16}$O
[We98b]
Flux impact:
Li 0.16%
Be 0.15%
B 0.14%
C 0.27%
N 0.29%
**O 6.12%**
$^{28}$Si + H → $^{17}$F*
Flux impact:
O 0.53%
$^{28}$Si + H → $^{17}$O
[We98b]
Flux impact:
N 0.11%
**O 3.2%**
$^{28}$Si + H → $^{18}$O
[We98b]
Flux impact:
**O 1.81%**
$^{28}$Si + H → $^{18}$F*
[Bi71] [We98b]
Flux impact:
**O 2.06%**
$^{28}$Si + H → $^{18}$Ne*
Flux impact:
O 0.19%
$^{28}$Si + H → $^{19}$Ne*
[We90] [We98b]
Flux impact:
O 0.15%
**F 2.99%**
$^{28}$Si + H → $^{19}$F
[We98b]
Flux impact:
O 0.41%
**F 8.12%**
$^{28}$Si + H → $^{19}$O*
Flux impact:
F 0.71%
$^{28}$Si + H → $^{20}$F*
[We98b]
Flux impact:
Ne 0.36%
GP12up22
GP12
GP22
$\sigma$ [mb]
$E_{k/n}$ [GeV/n]

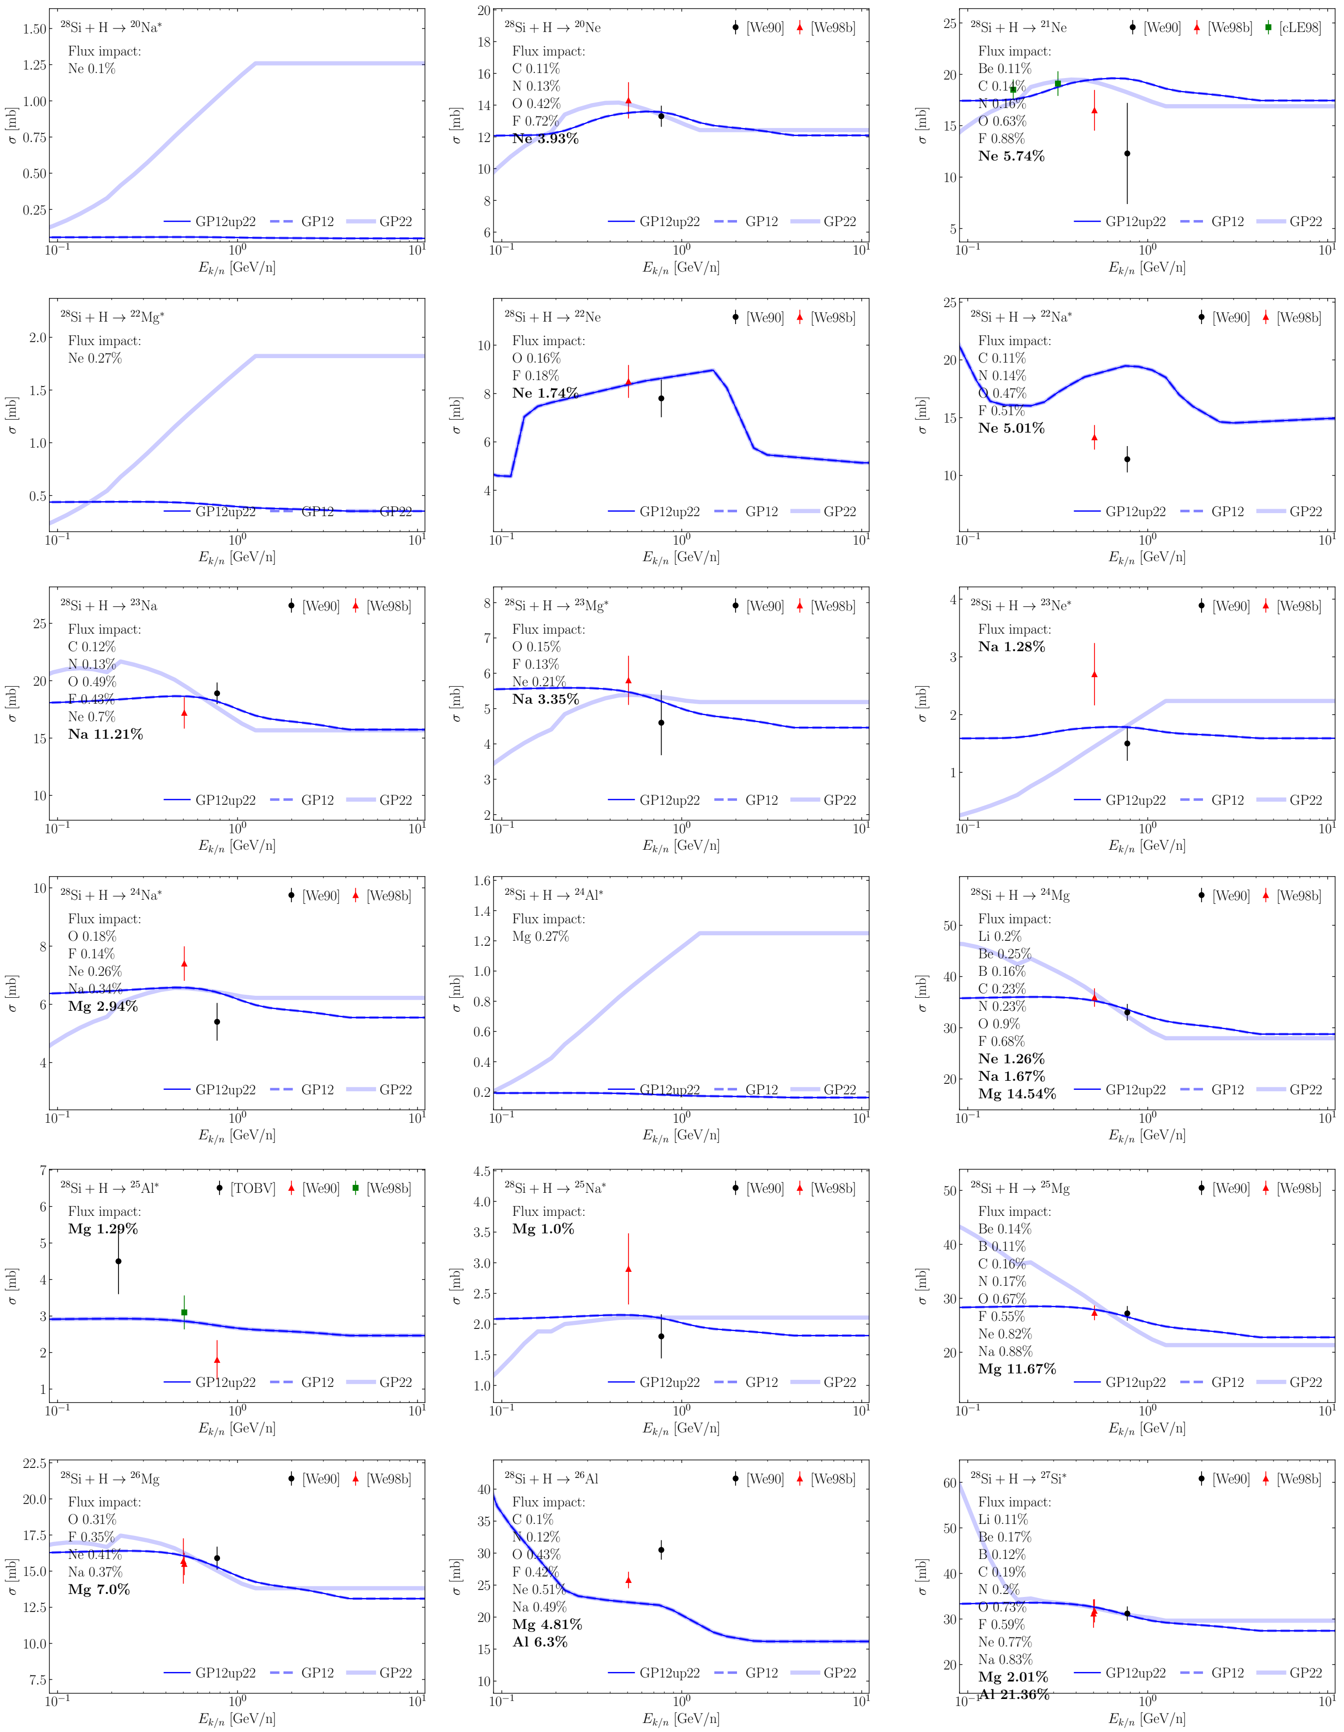

$^{28}$Si + H → $^{20}$Na*
Flux impact:
Ne 0.1%
$^{28}$Si + H → $^{20}$Ne
[We90] [We98b]
Flux impact:
C 0.11%
N 0.13%
O 0.42%
F 0.72%
**Ne 3.93%**
$^{28}$Si + H → $^{21}$Ne
[We90] [We98b] [cLE98]
Flux impact:
Be 0.11%
C 0.14%
N 0.16%
O 0.63%
F 0.88%
**Ne 5.74%**
$^{28}$Si + H → $^{22}$Mg*
Flux impact:
Ne 0.27%
$^{28}$Si + H → $^{22}$Ne
[We90] [We98b]
Flux impact:
O 0.16%
F 0.18%
**Ne 1.74%**
$^{28}$Si + H → $^{22}$Na*
[We90] [We98b]
Flux impact:
C 0.11%
N 0.14%
O 0.47%
F 0.51%
**Ne 5.01%**
$^{28}$Si + H → $^{23}$Na
[We90] [We98b]
Flux impact:
C 0.12%
N 0.13%
O 0.49%
F 0.43%
Ne 0.7%
**Na 11.21%**
$^{28}$Si + H → $^{23}$Mg*
[We90] [We98b]
Flux impact:
O 0.15%
F 0.13%
Ne 0.21%
**Na 3.35%**
$^{28}$Si + H → $^{23}$Ne*
[We90] [We98b]
Flux impact:
**Na 1.28%**
$^{28}$Si + H → $^{24}$Na*
[We90] [We98b]
Flux impact:
O 0.18%
F 0.14%
Ne 0.26%
Na 0.34%
**Mg 2.94%**
$^{28}$Si + H → $^{24}$Al*
Flux impact:
Mg 0.27%
$^{28}$Si + H → $^{24}$Mg
[We90] [We98b]
Flux impact:
Li 0.2%
Be 0.25%
B 0.16%
C 0.23%
N 0.23%
O 0.9%
F 0.68%
**Ne 1.26%**
**Na 1.67%**
**Mg 14.54%**
$^{28}$Si + H → $^{25}$Al*
[TOBV] [We90] [We98b]
Flux impact:
**Mg 1.29%**
$^{28}$Si + H → $^{25}$Na*
[We90] [We98b]
Flux impact:
**Mg 1.0%**
$^{28}$Si + H → $^{25}$Mg
[We90] [We98b]
Flux impact:
Be 0.14%
B 0.11%
C 0.16%
N 0.17%
O 0.67%
F 0.55%
Ne 0.82%
Na 0.88%
**Mg 11.67%**
$^{28}$Si + H → $^{26}$Mg
[We90] [We98b]
Flux impact:
O 0.31%
F 0.35%
Ne 0.41%
Na 0.37%
**Mg 7.0%**
$^{28}$Si + H → $^{26}$Al
[We90] [We98b]
Flux impact:
C 0.1%
N 0.12%
O 0.43%
F 0.42%
Ne 0.51%
Na 0.49%
**Mg 4.81%**
**Al 6.3%**
$^{28}$Si + H → $^{27}$Si*
[We90] [We98b]
Flux impact:
Li 0.11%
Be 0.17%
B 0.12%
C 0.19%
N 0.2%
O 0.73%
F 0.59%
Ne 0.77%
Na 0.83%
**Mg 2.01%**
**Al 21.36%**
GP12up22 GP12 GP22
$\sigma$ [mb]
$E_{k/n}$ [GeV/n]

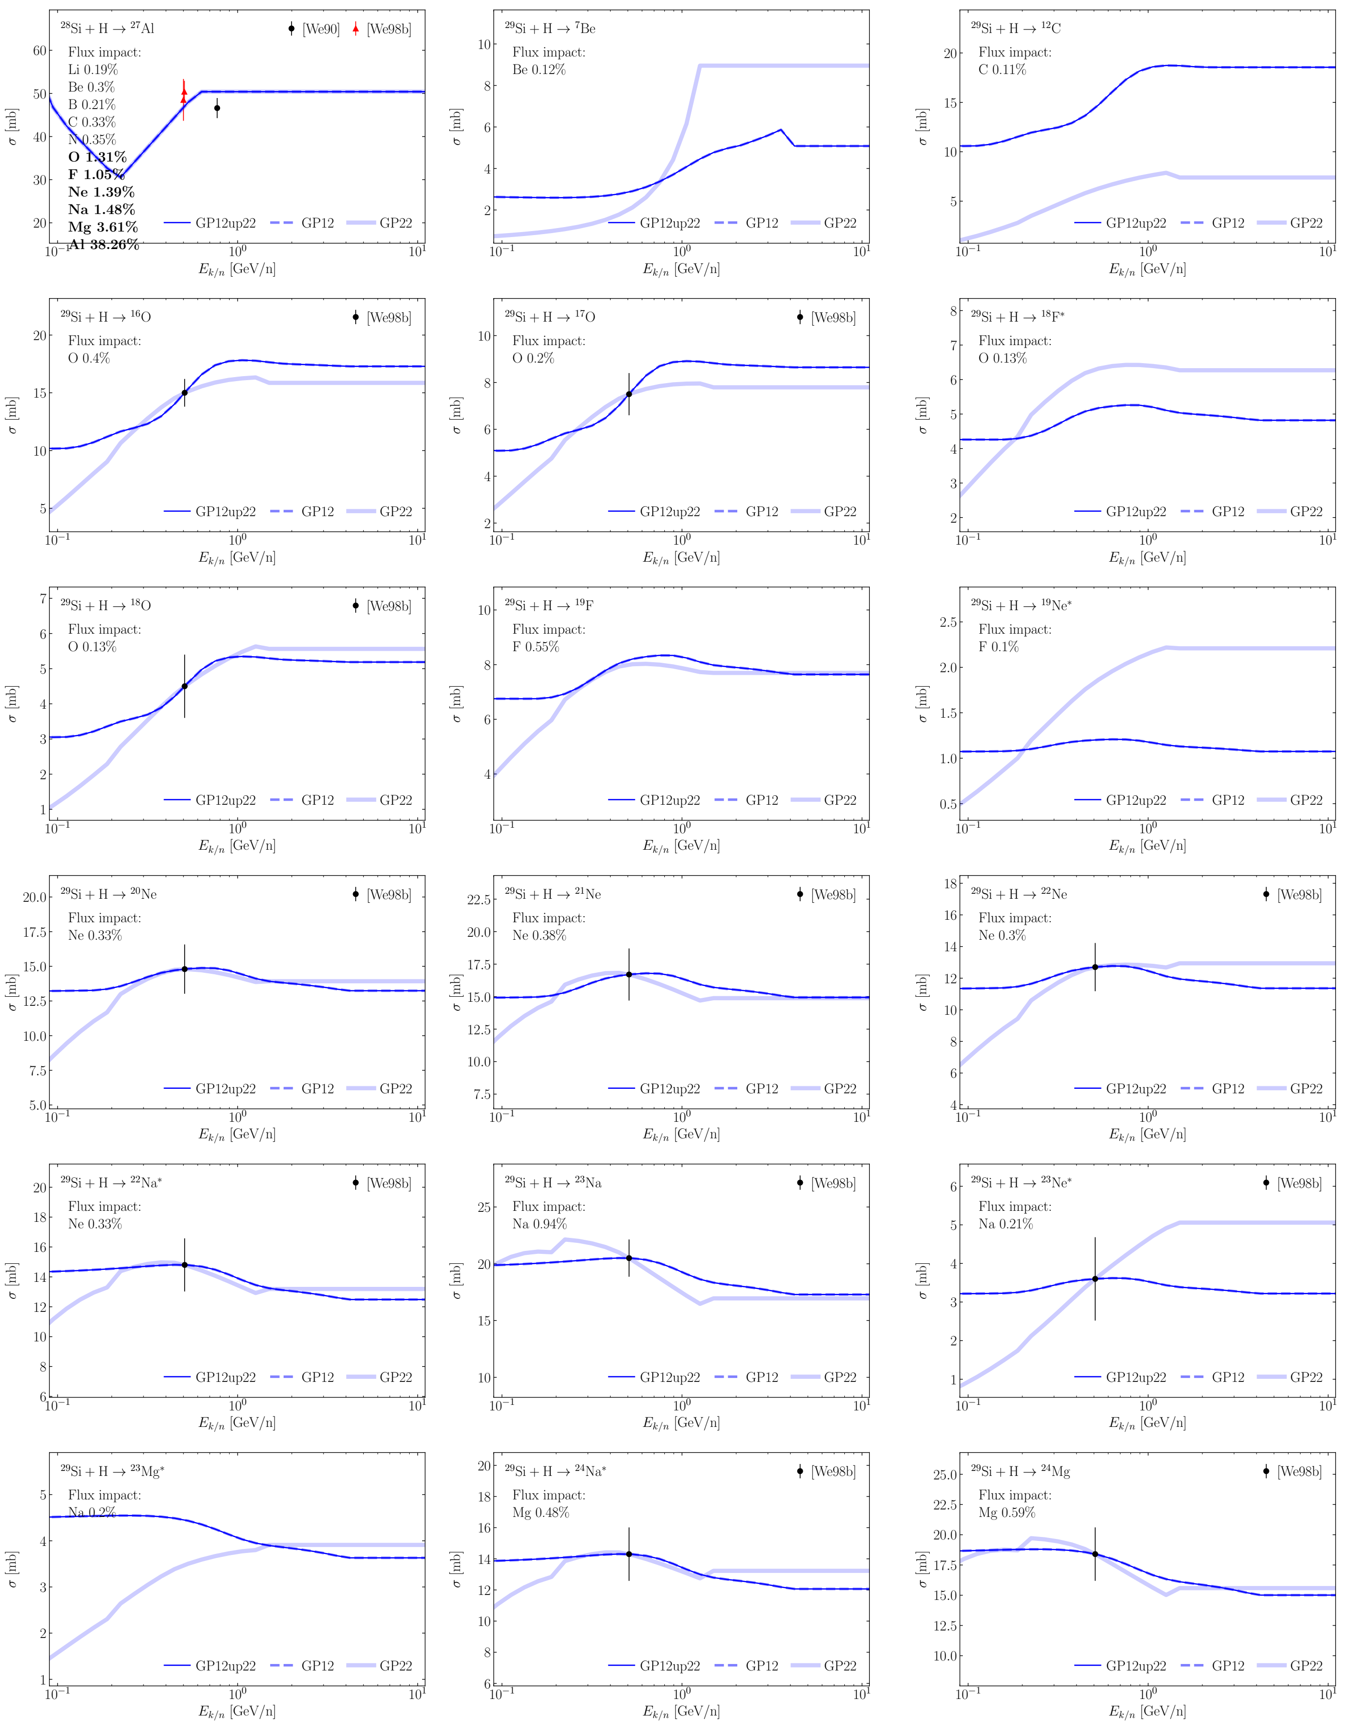

28Si + H → 27Al
[We90] [We98b]
Flux impact:
Li 0.19%
Be 0.3%
B 0.21%
C 0.33%
N 0.35%
O 1.31%
F 1.05%
Ne 1.39%
Na 1.48%
Mg 3.61%
Al 38.26%
29Si + H → 7Be
Flux impact:
Be 0.12%
29Si + H → 12C
Flux impact:
C 0.11%
29Si + H → 16O
[We98b]
Flux impact:
O 0.4%
29Si + H → 17O
[We98b]
Flux impact:
O 0.2%
29Si + H → 18F*
Flux impact:
O 0.13%
29Si + H → 18O
[We98b]
Flux impact:
O 0.13%
29Si + H → 19F
Flux impact:
F 0.55%
29Si + H → 19Ne*
Flux impact:
F 0.1%
29Si + H → 20Ne
[We98b]
Flux impact:
Ne 0.33%
29Si + H → 21Ne
[We98b]
Flux impact:
Ne 0.38%
29Si + H → 22Ne
[We98b]
Flux impact:
Ne 0.3%
29Si + H → 22Na*
[We98b]
Flux impact:
Ne 0.33%
29Si + H → 23Na
[We98b]
Flux impact:
Na 0.94%
29Si + H → 23Ne*
[We98b]
Flux impact:
Na 0.21%
29Si + H → 23Mg*
Flux impact:
Na 0.2%
29Si + H → 24Na*
[We98b]
Flux impact:
Mg 0.48%
29Si + H → 24Mg
[We98b]
Flux impact:
Mg 0.59%
GP12up22 GP12 GP22
σ [mb]
E_k/n [GeV/n]

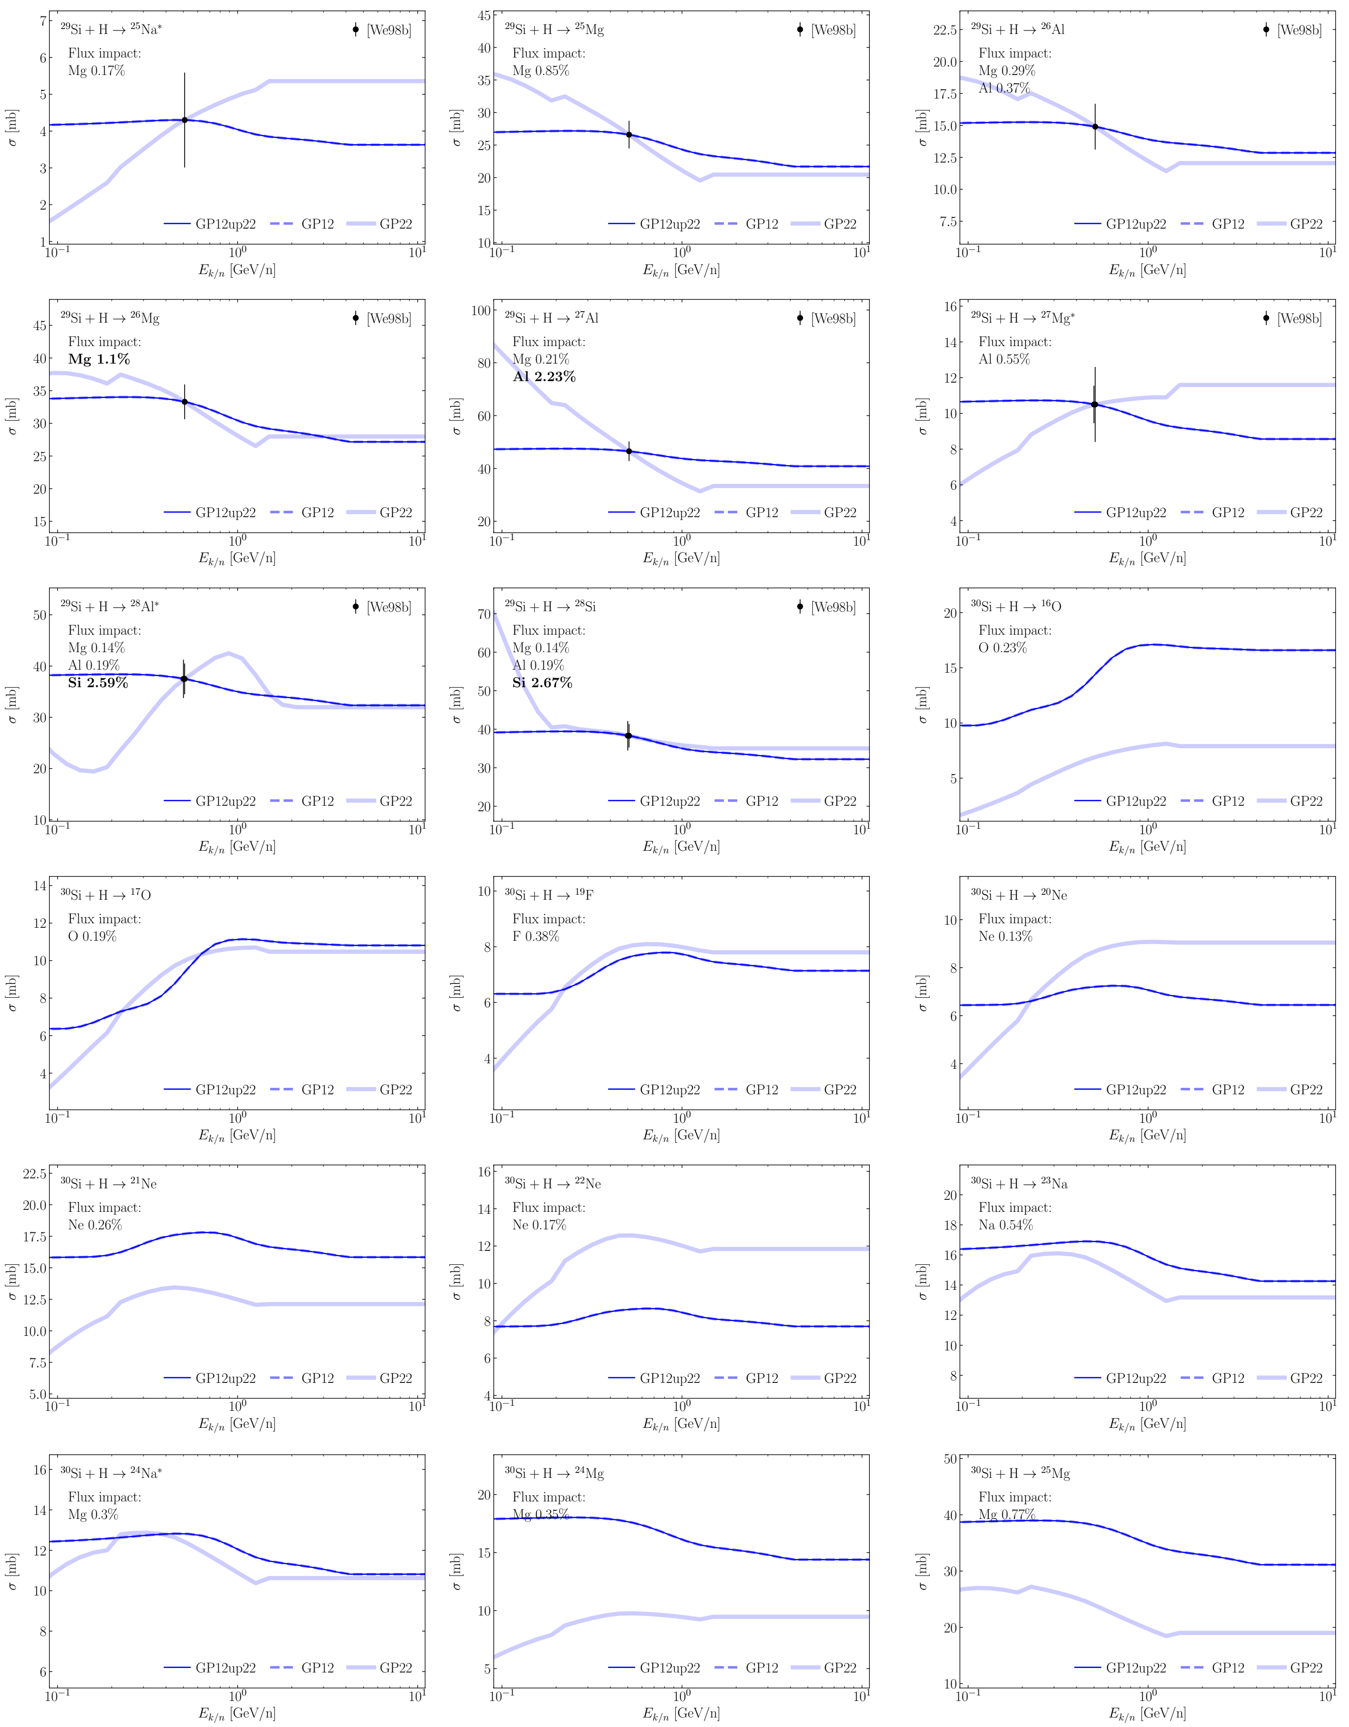

$^{29}$Si + H → $^{25}$Na*
[We98b]
Flux impact:
Mg 0.17%
$^{29}$Si + H → $^{25}$Mg
[We98b]
Flux impact:
Mg 0.85%
$^{29}$Si + H → $^{26}$Al
[We98b]
Flux impact:
Mg 0.29%
Al 0.37%
$^{29}$Si + H → $^{26}$Mg
[We98b]
Flux impact:
Mg 1.1%
$^{29}$Si + H → $^{27}$Al
[We98b]
Flux impact:
Mg 0.21%
Al 2.23%
$^{29}$Si + H → $^{27}$Mg*
[We98b]
Flux impact:
Al 0.55%
$^{29}$Si + H → $^{28}$Al*
[We98b]
Flux impact:
Mg 0.14%
Al 0.19%
Si 2.59%
$^{29}$Si + H → $^{28}$Si
[We98b]
Flux impact:
Mg 0.14%
Al 0.19%
Si 2.67%
$^{30}$Si + H → $^{16}$O
Flux impact:
O 0.23%
$^{30}$Si + H → $^{17}$O
Flux impact:
O 0.19%
$^{30}$Si + H → $^{19}$F
Flux impact:
F 0.38%
$^{30}$Si + H → $^{20}$Ne
Flux impact:
Ne 0.13%
$^{30}$Si + H → $^{21}$Ne
Flux impact:
Ne 0.26%
$^{30}$Si + H → $^{22}$Ne
Flux impact:
Ne 0.17%
$^{30}$Si + H → $^{23}$Na
Flux impact:
Na 0.54%
$^{30}$Si + H → $^{24}$Na*
Flux impact:
Mg 0.3%
$^{30}$Si + H → $^{24}$Mg
Flux impact:
Mg 0.35%
$^{30}$Si + H → $^{25}$Mg
Flux impact:
Mg 0.77%
GP12up22
GP12
GP22
$\sigma$ [mb]
$E_{k/n}$ [GeV/n]

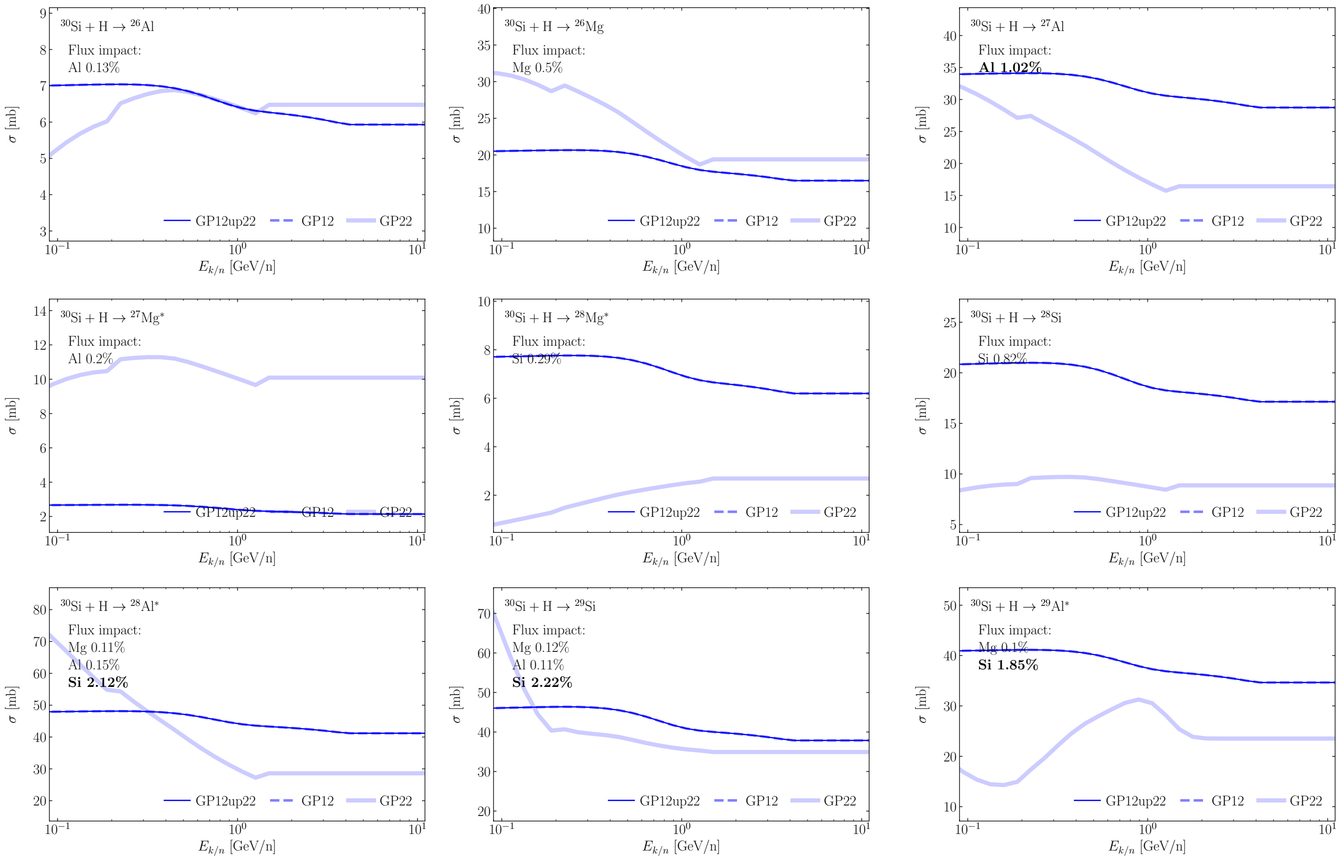


## Z=15 projectiles: $^{x}$P + H → $^{A}_{Z}X$

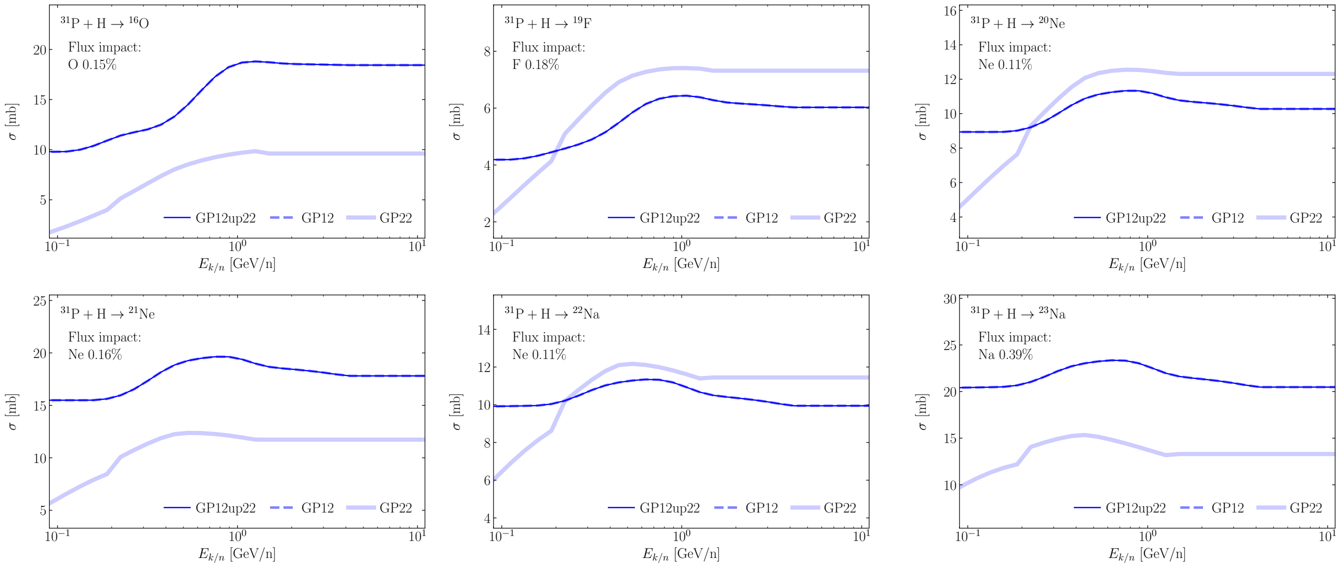

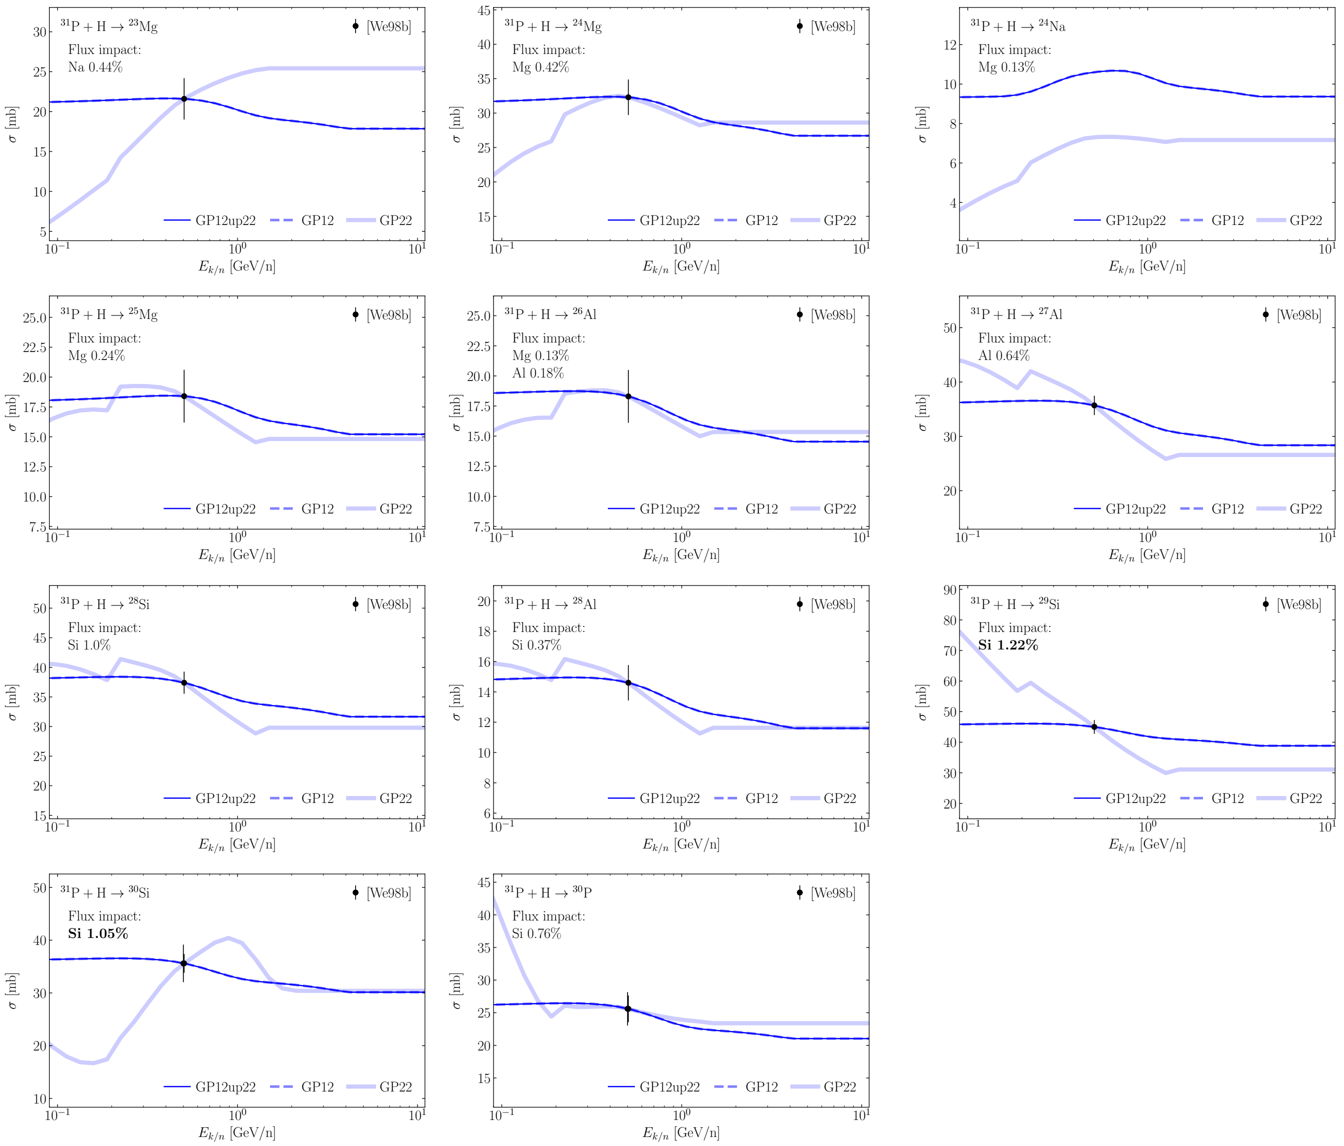


## Z=16 projectiles: $^{x}$S + H → $^{A}_{Z}X$

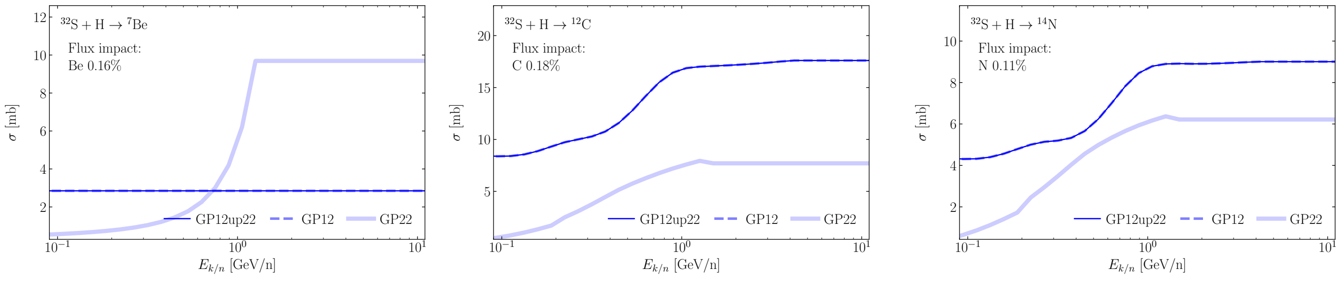

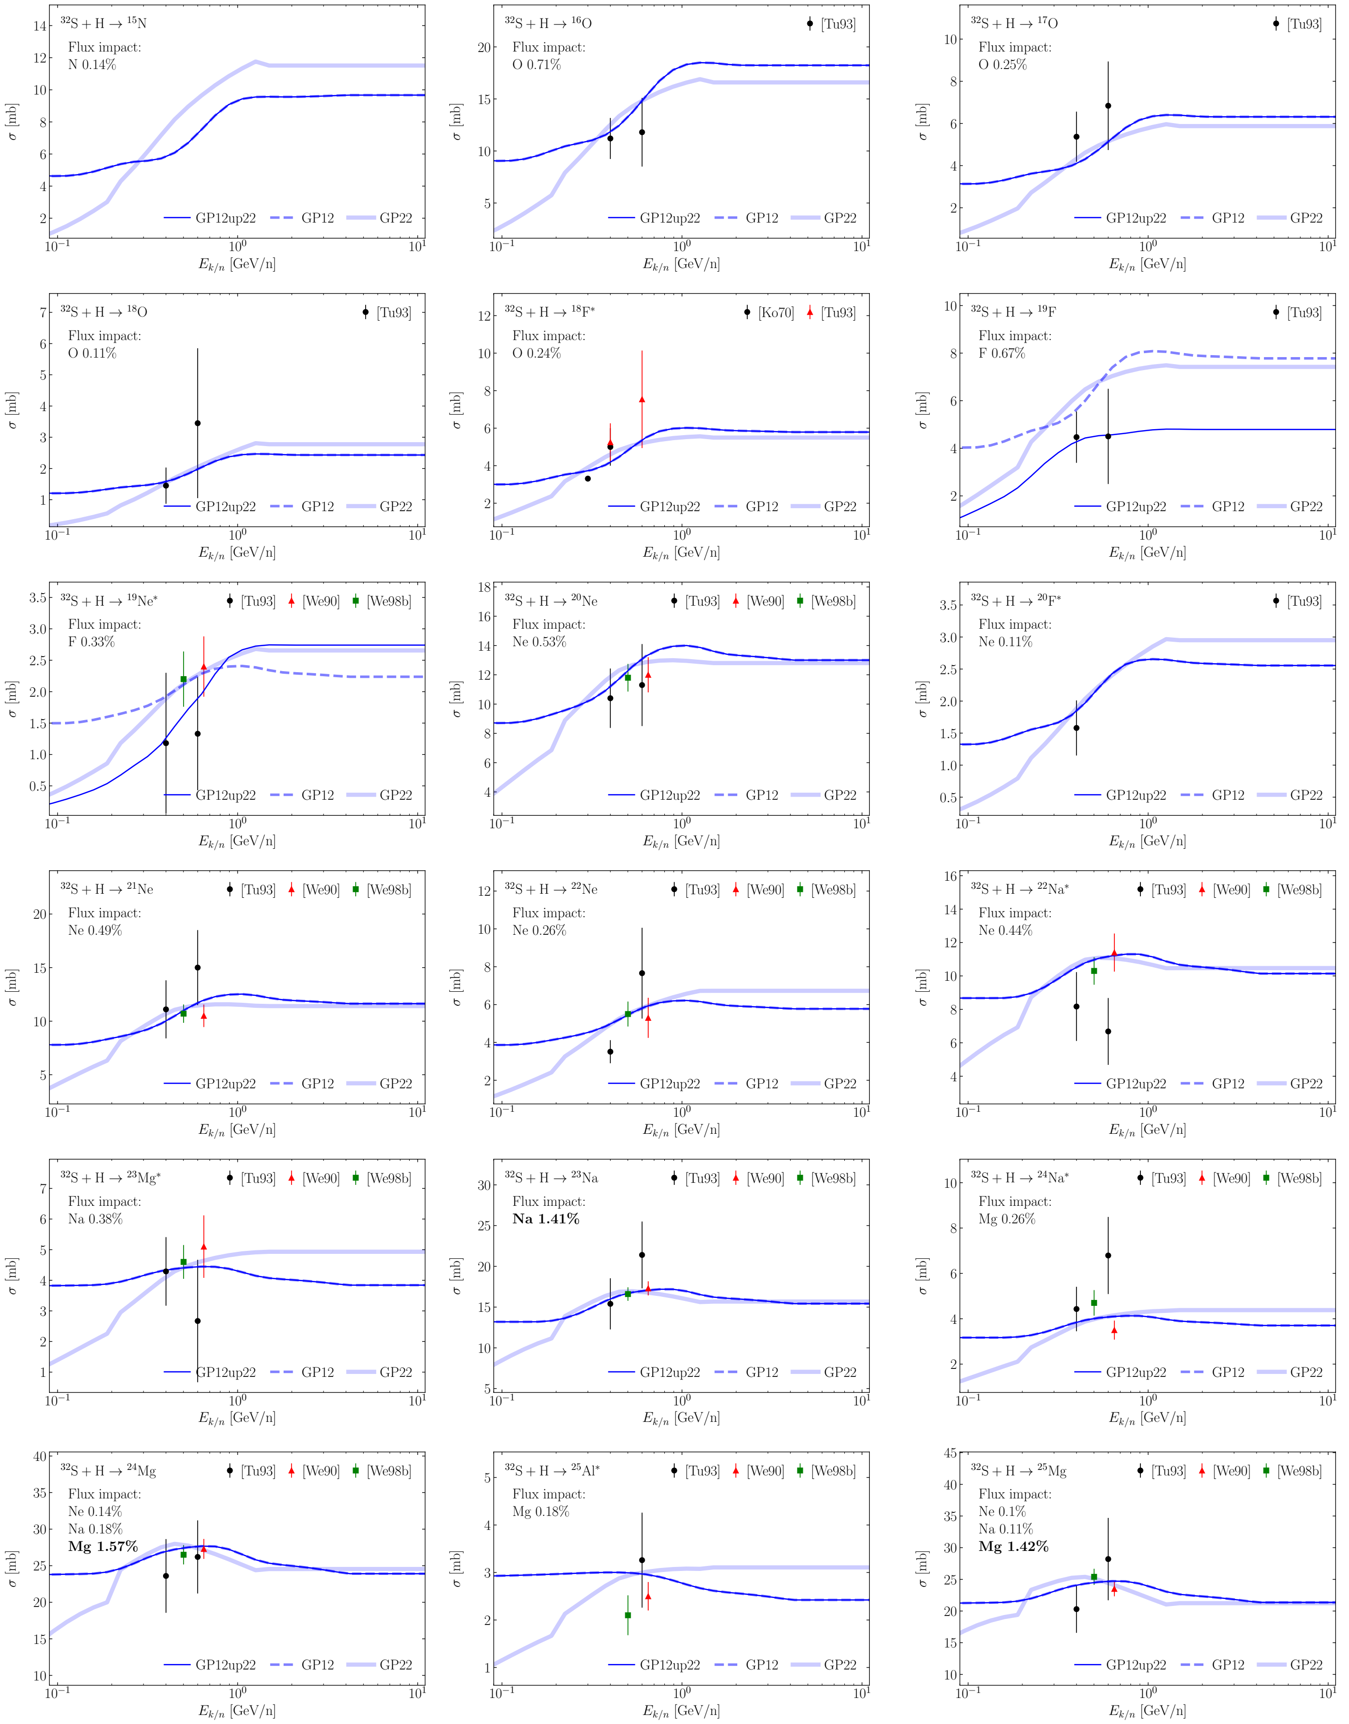

$^{32}$S + H → $^{15}$N
Flux impact:
N 0.14%
$^{32}$S + H → $^{16}$O
[Tu93]
Flux impact:
O 0.71%
$^{32}$S + H → $^{17}$O
[Tu93]
Flux impact:
O 0.25%
$^{32}$S + H → $^{18}$O
[Tu93]
Flux impact:
O 0.11%
$^{32}$S + H → $^{18}$F*
[Ko70] [Tu93]
Flux impact:
O 0.24%
$^{32}$S + H → $^{19}$F
[Tu93]
Flux impact:
F 0.67%
$^{32}$S + H → $^{19}$Ne*
[Tu93] [We90] [We98b]
Flux impact:
F 0.33%
$^{32}$S + H → $^{20}$Ne
[Tu93] [We90] [We98b]
Flux impact:
Ne 0.53%
$^{32}$S + H → $^{20}$F*
[Tu93]
Flux impact:
Ne 0.11%
$^{32}$S + H → $^{21}$Ne
[Tu93] [We90] [We98b]
Flux impact:
Ne 0.49%
$^{32}$S + H → $^{22}$Ne
[Tu93] [We90] [We98b]
Flux impact:
Ne 0.26%
$^{32}$S + H → $^{22}$Na*
[Tu93] [We90] [We98b]
Flux impact:
Ne 0.44%
$^{32}$S + H → $^{23}$Mg*
[Tu93] [We90] [We98b]
Flux impact:
Na 0.38%
$^{32}$S + H → $^{23}$Na
[Tu93] [We90] [We98b]
Flux impact:
Na 1.41%
$^{32}$S + H → $^{24}$Na*
[Tu93] [We90] [We98b]
Flux impact:
Mg 0.26%
$^{32}$S + H → $^{24}$Mg
[Tu93] [We90] [We98b]
Flux impact:
Ne 0.14%
Na 0.18%
Mg 1.57%
$^{32}$S + H → $^{25}$Al*
[Tu93] [We90] [We98b]
Flux impact:
Mg 0.18%
$^{32}$S + H → $^{25}$Mg
[Tu93] [We90] [We98b]
Flux impact:
Ne 0.1%
Na 0.11%
Mg 1.42%
GP12up22
GP12
GP22
$\sigma$ [mb]
$E_{k/n}$ [GeV/n]

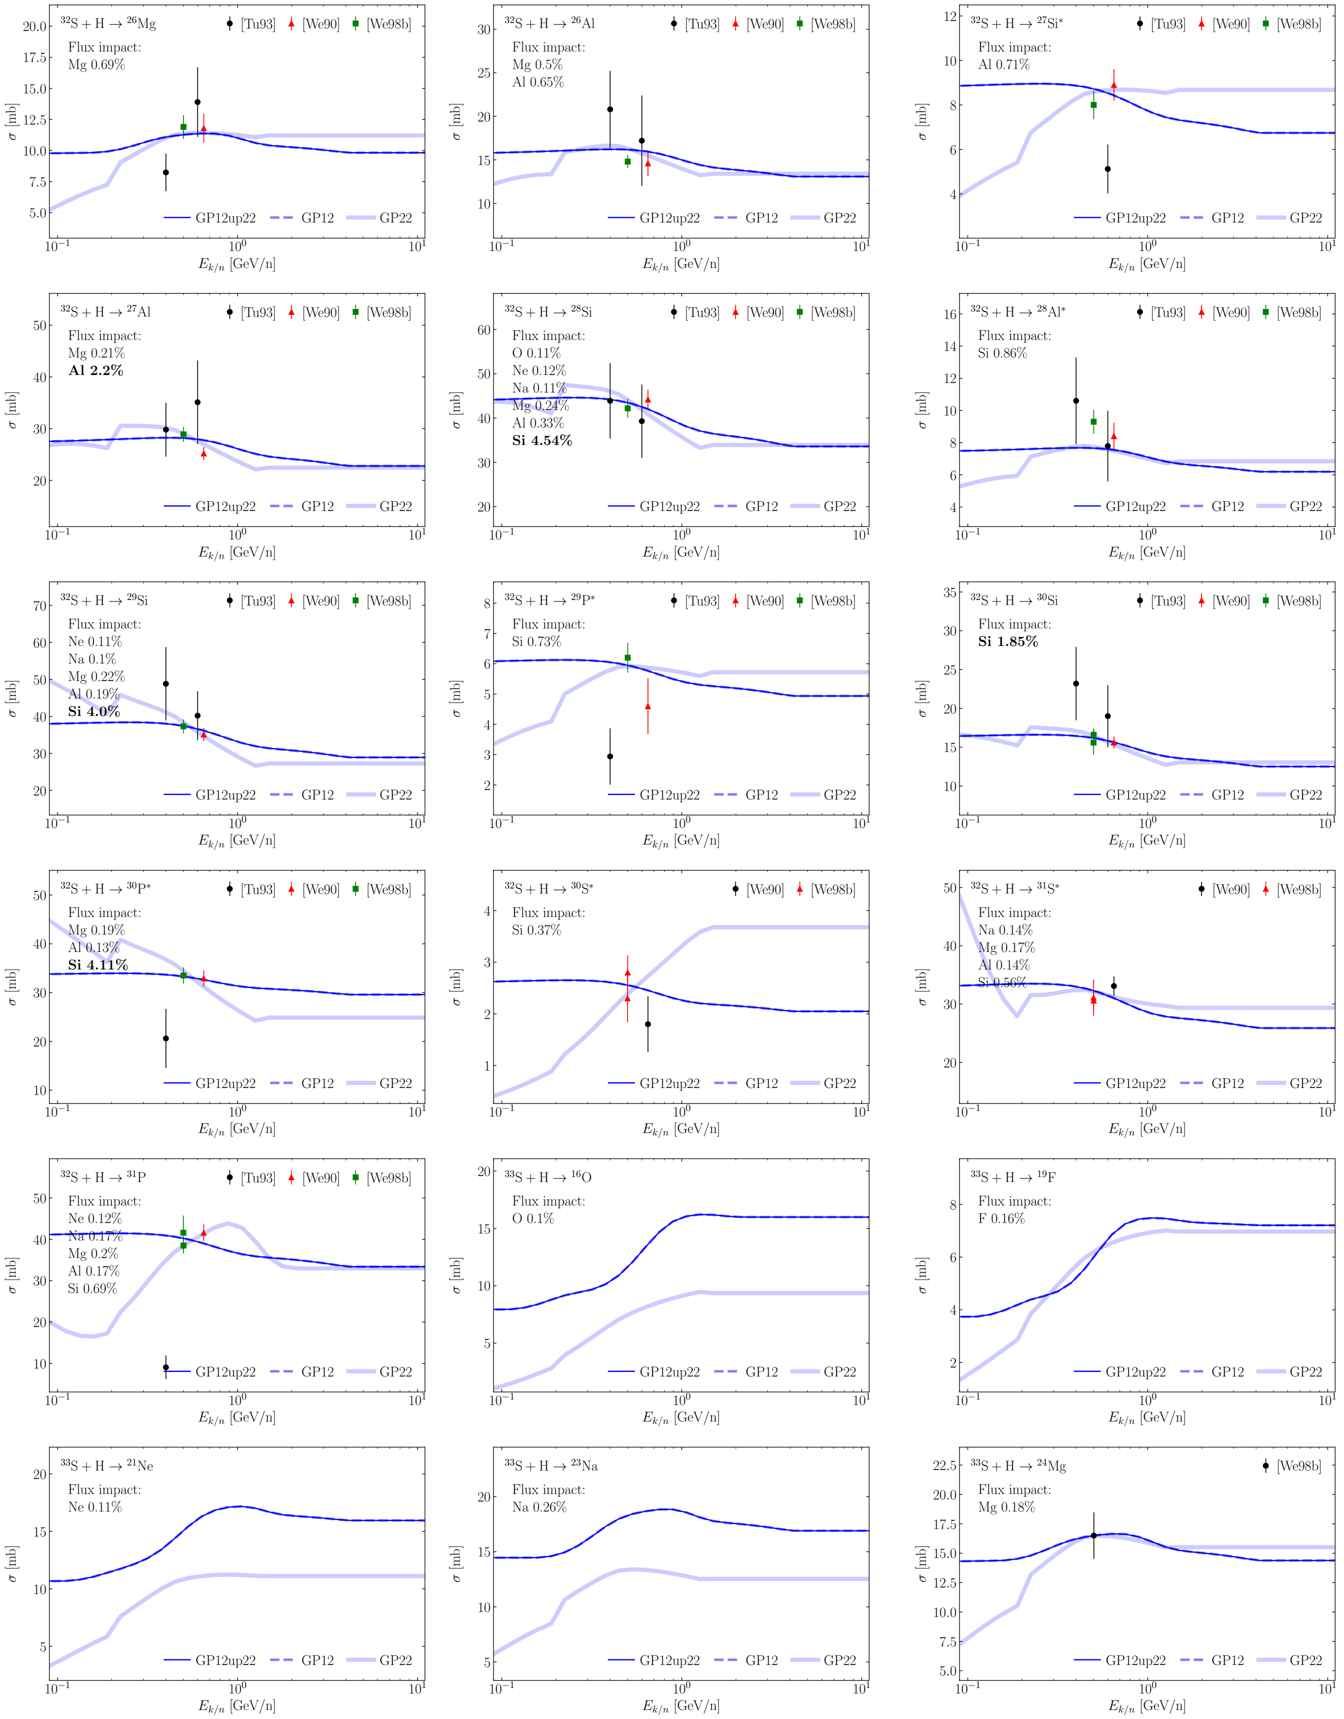

32S + H → 26Mg
Flux impact:
Mg 0.69%
32S + H → 26Al
Flux impact:
Mg 0.5%
Al 0.65%
32S + H → 27Si*
Flux impact:
Al 0.71%
32S + H → 27Al
Flux impact:
Mg 0.21%
Al 2.2%
32S + H → 28Si
Flux impact:
O 0.11%
Ne 0.12%
Na 0.11%
Mg 0.24%
Al 0.33%
Si 4.54%
32S + H → 28Al*
Flux impact:
Si 0.86%
32S + H → 29Si
Flux impact:
Ne 0.11%
Na 0.1%
Mg 0.22%
Al 0.19%
Si 4.0%
32S + H → 29P*
Flux impact:
Si 0.73%
32S + H → 30Si
Flux impact:
Si 1.85%
32S + H → 30P*
Flux impact:
Mg 0.19%
Al 0.13%
Si 4.11%
32S + H → 30S*
Flux impact:
Si 0.37%
32S + H → 31S*
Flux impact:
Na 0.14%
Mg 0.17%
Al 0.14%
Si 0.56%
32S + H → 31P
Flux impact:
Ne 0.12%
Na 0.17%
Mg 0.2%
Al 0.17%
Si 0.69%
33S + H → 16O
Flux impact:
O 0.1%
33S + H → 19F
Flux impact:
F 0.16%
33S + H → 21Ne
Flux impact:
Ne 0.11%
33S + H → 23Na
Flux impact:
Na 0.26%
33S + H → 24Mg
Flux impact:
Mg 0.18%
[Tu93] [We90] [We98b]
GP12up22 GP12 GP22
σ [mb]
E_k/n [GeV/n]

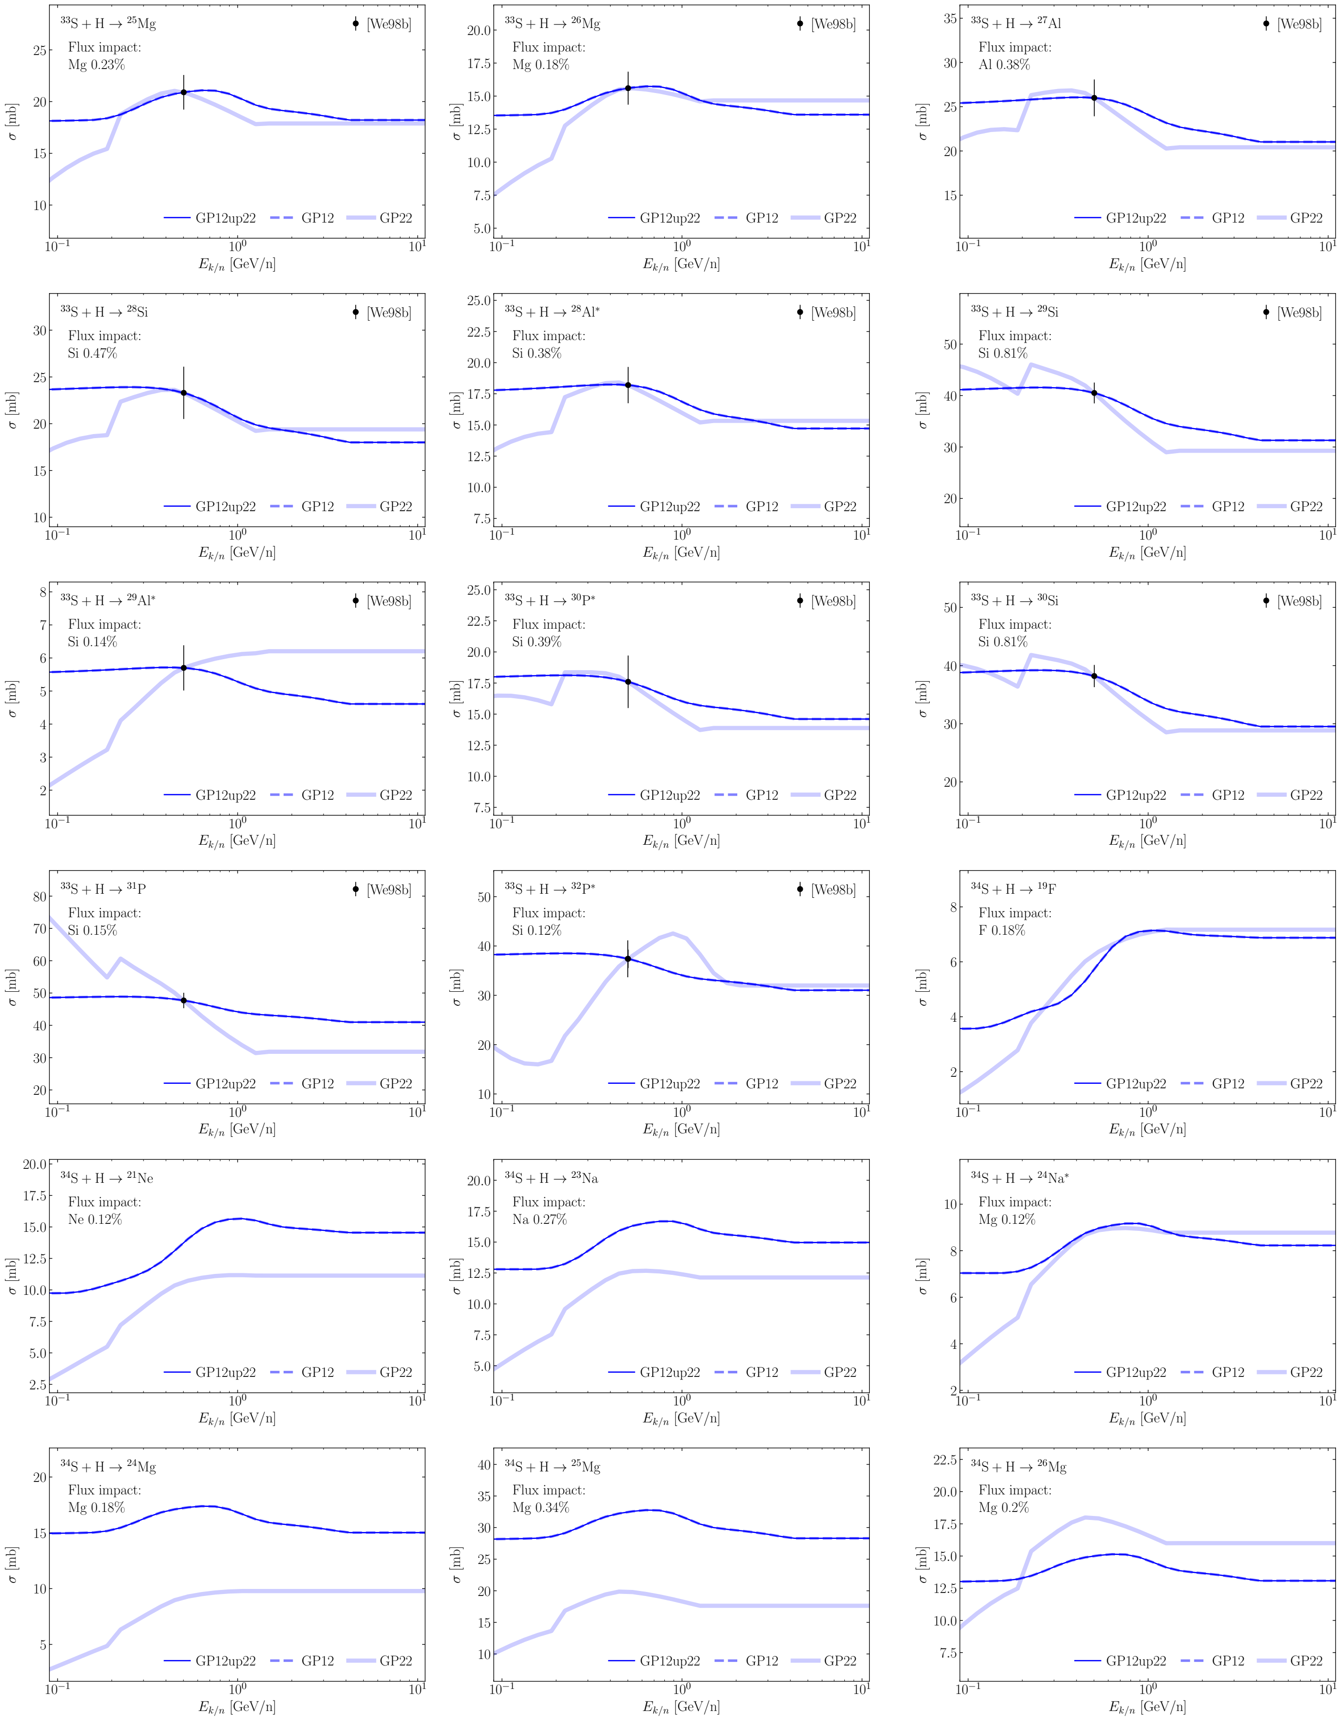
$^{33}$S + H → $^{25}$Mg
Flux impact:
Mg 0.23%
$^{33}$S + H → $^{26}$Mg
Flux impact:
Mg 0.18%
$^{33}$S + H → $^{27}$Al
Flux impact:
Al 0.38%
$^{33}$S + H → $^{28}$Si
Flux impact:
Si 0.47%
$^{33}$S + H → $^{28}$Al*
Flux impact:
Si 0.38%
$^{33}$S + H → $^{29}$Si
Flux impact:
Si 0.81%
$^{33}$S + H → $^{29}$Al*
Flux impact:
Si 0.14%
$^{33}$S + H → $^{30}$P*
Flux impact:
Si 0.39%
$^{33}$S + H → $^{30}$Si
Flux impact:
Si 0.81%
$^{33}$S + H → $^{31}$P
Flux impact:
Si 0.15%
$^{33}$S + H → $^{32}$P*
Flux impact:
Si 0.12%
$^{34}$S + H → $^{19}$F
Flux impact:
F 0.18%
$^{34}$S + H → $^{21}$Ne
Flux impact:
Ne 0.12%
$^{34}$S + H → $^{23}$Na
Flux impact:
Na 0.27%
$^{34}$S + H → $^{24}$Na*
Flux impact:
Mg 0.12%
$^{34}$S + H → $^{24}$Mg
Flux impact:
Mg 0.18%
$^{34}$S + H → $^{25}$Mg
Flux impact:
Mg 0.34%
$^{34}$S + H → $^{26}$Mg
Flux impact:
Mg 0.2%
[We98b]
GP12up22
GP12
GP22
$\sigma$ [mb]
$E_{k/n}$ [GeV/n]

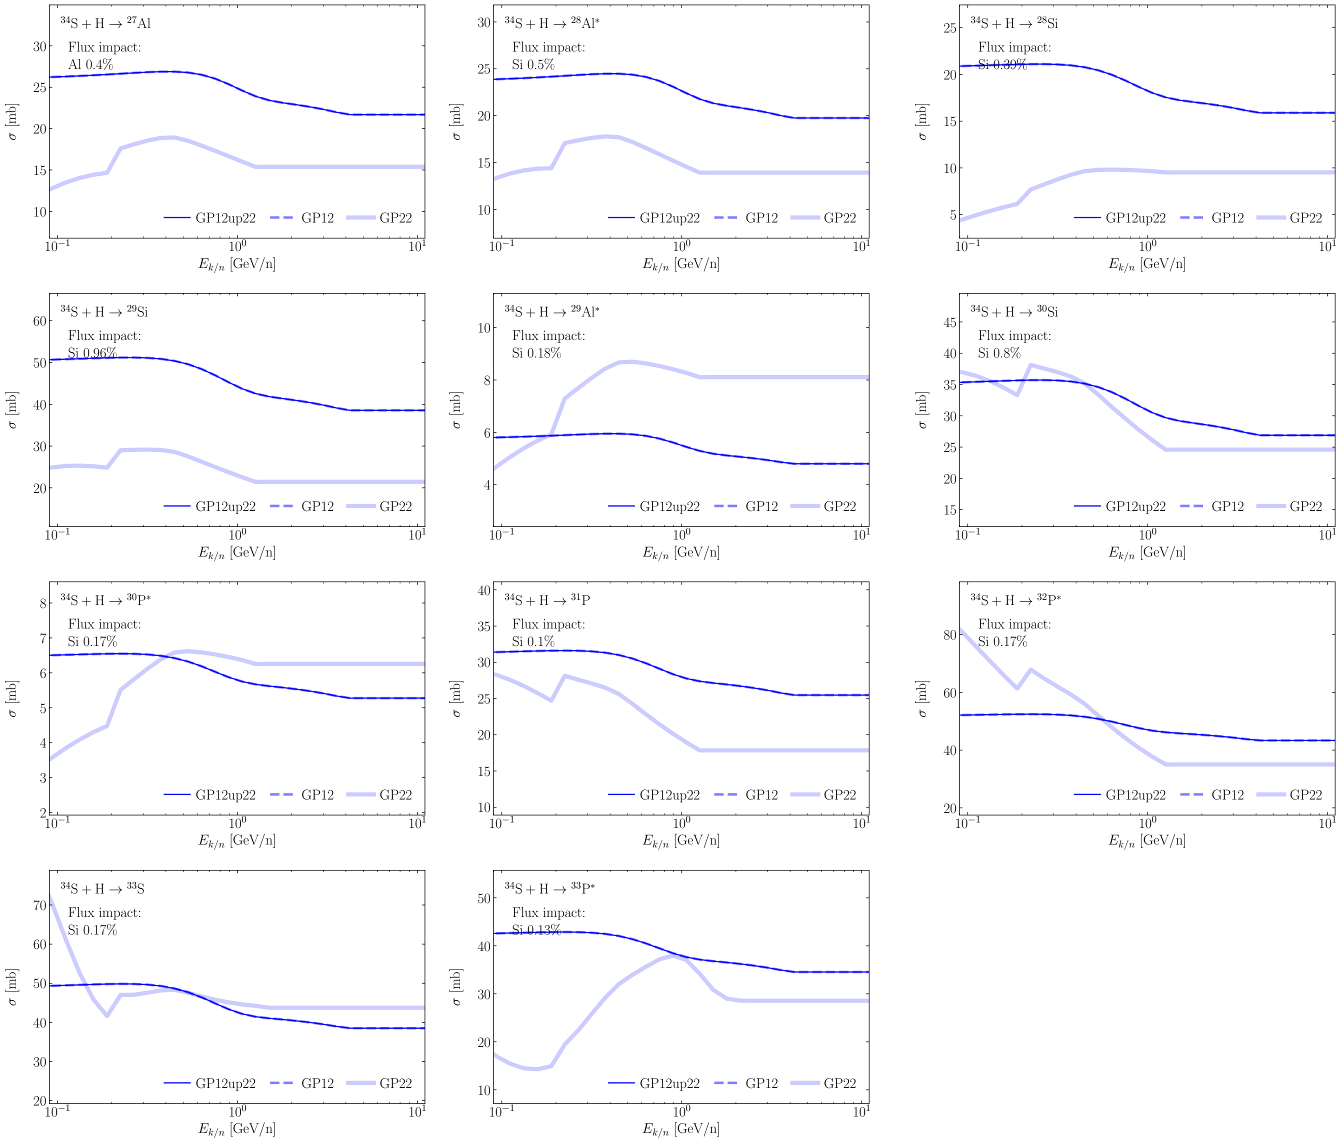


## Z=17 projectiles: $^{x}$Cl + H $\to$ $^{A}_{Z}X$

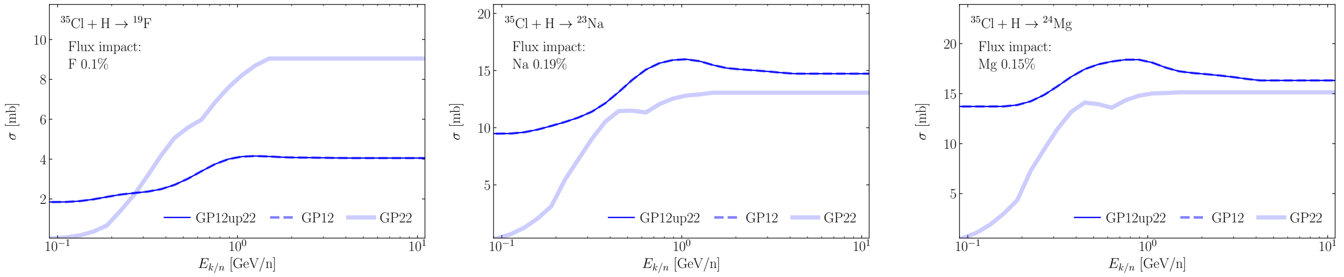

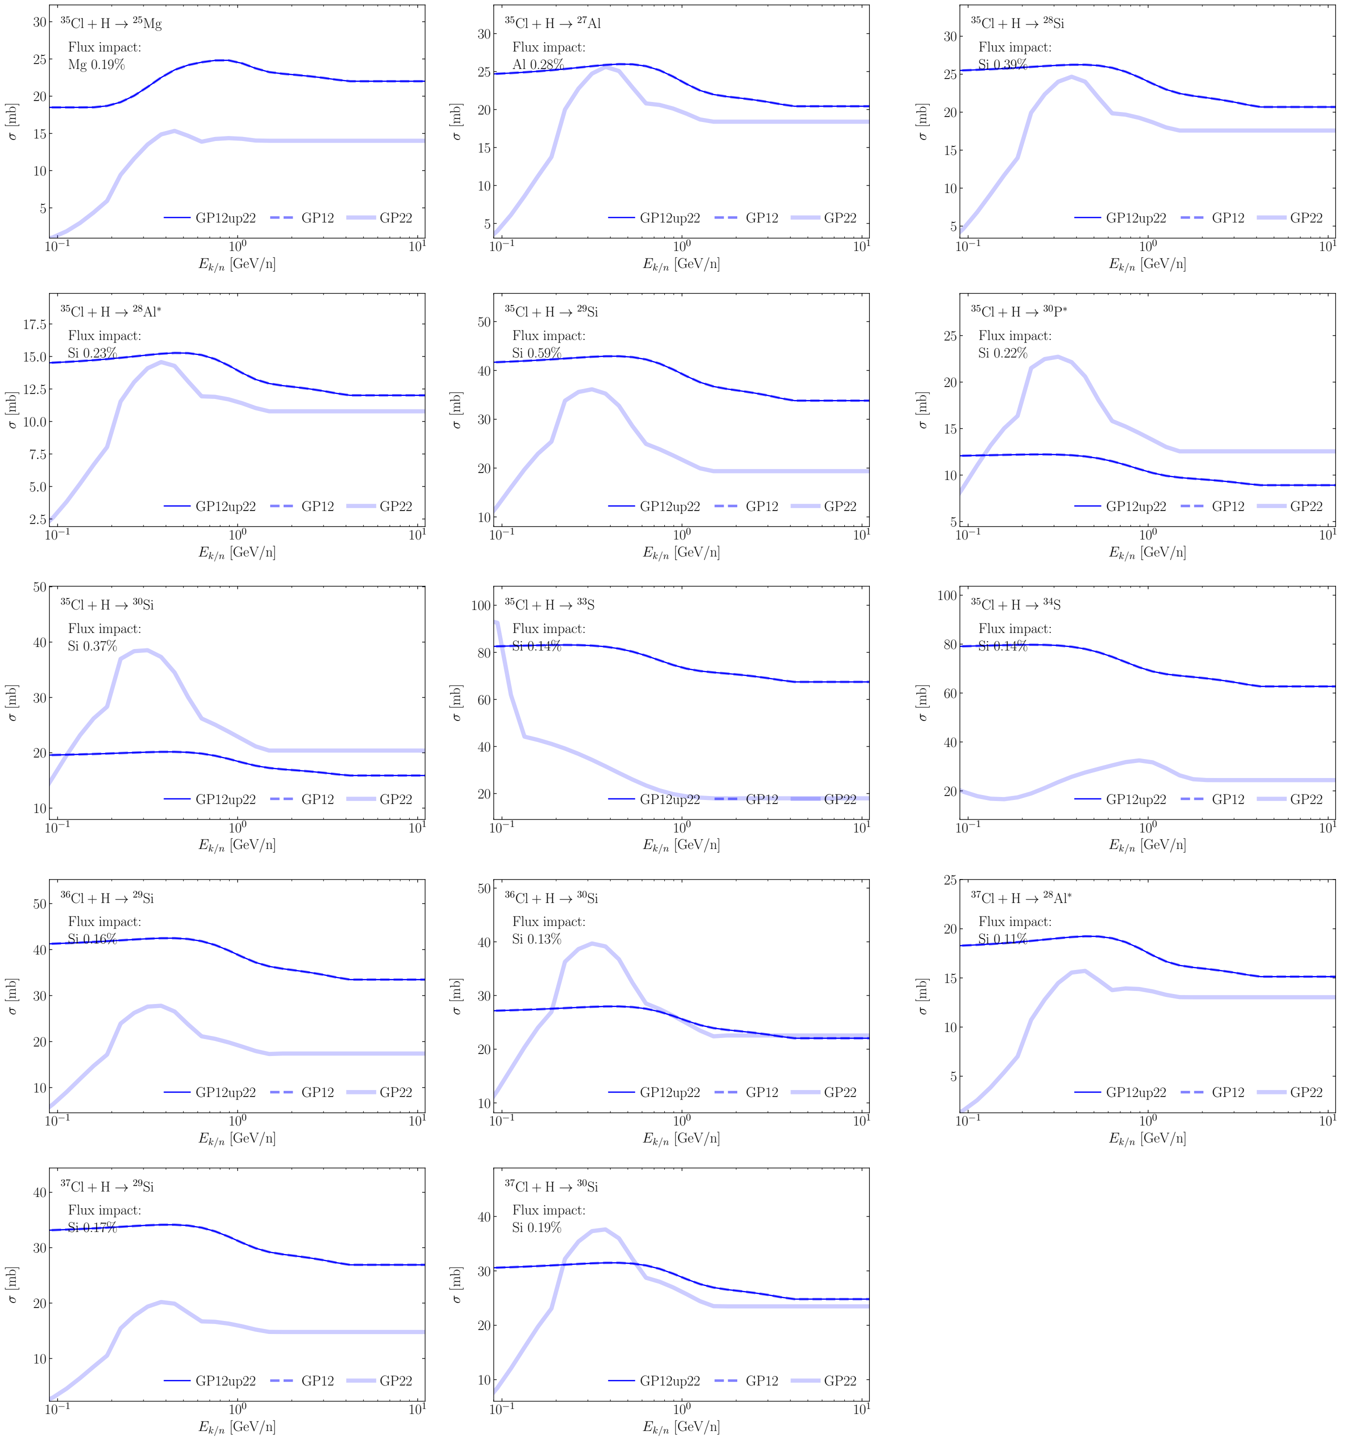


**Z=18 projectiles: $^{x}$Ar + H → $^{A}_{Z}X$**

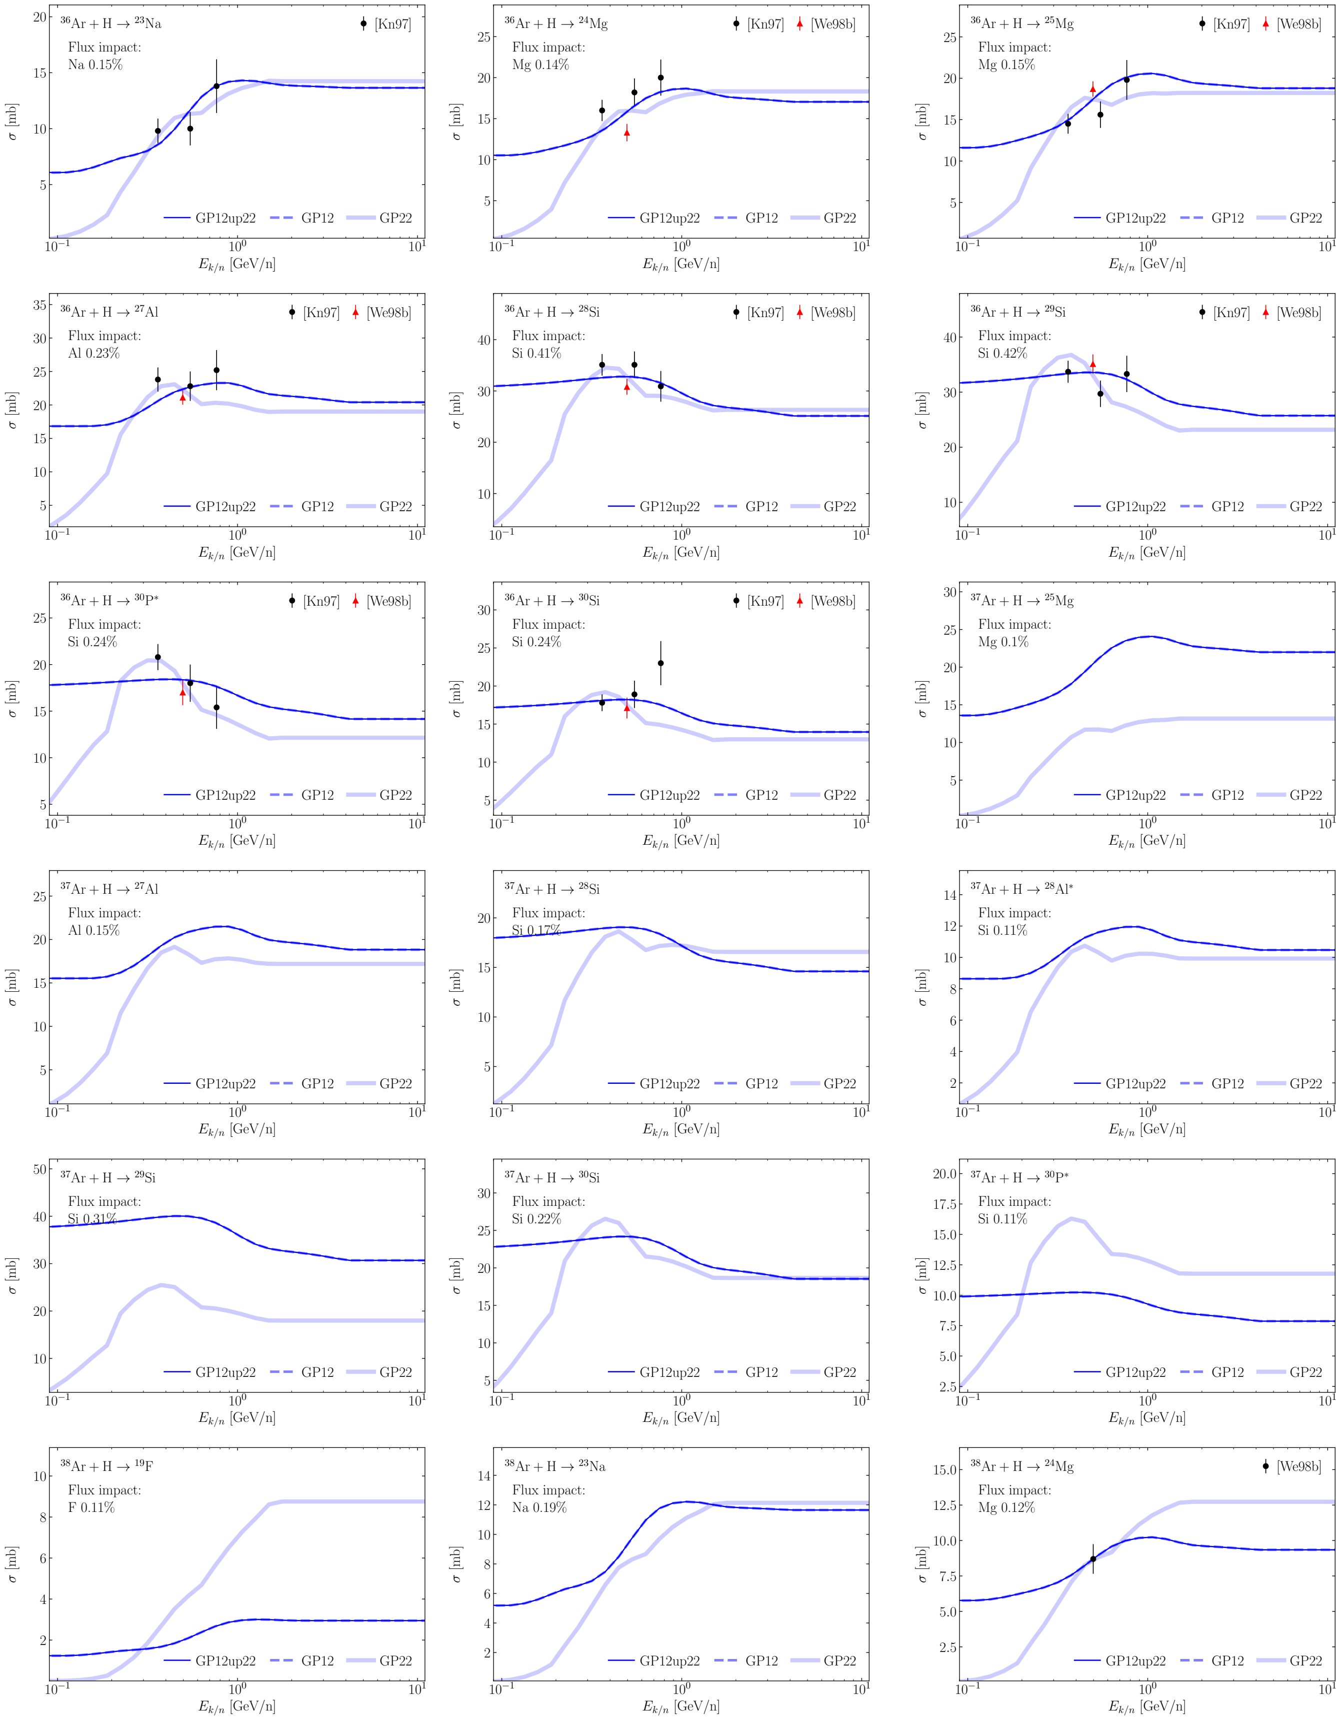
36Ar + H → 23Na
[Kn97]
Flux impact:
Na 0.15%
36Ar + H → 24Mg
[Kn97] [We98b]
Flux impact:
Mg 0.14%
36Ar + H → 25Mg
[Kn97] [We98b]
Flux impact:
Mg 0.15%
36Ar + H → 27Al
[Kn97] [We98b]
Flux impact:
Al 0.23%
36Ar + H → 28Si
[Kn97] [We98b]
Flux impact:
Si 0.41%
36Ar + H → 29Si
[Kn97] [We98b]
Flux impact:
Si 0.42%
36Ar + H → 30P*
[Kn97] [We98b]
Flux impact:
Si 0.24%
36Ar + H → 30Si
[Kn97] [We98b]
Flux impact:
Si 0.24%
37Ar + H → 25Mg
Flux impact:
Mg 0.1%
37Ar + H → 27Al
Flux impact:
Al 0.15%
37Ar + H → 28Si
Flux impact:
Si 0.17%
37Ar + H → 28Al*
Flux impact:
Si 0.11%
37Ar + H → 29Si
Flux impact:
Si 0.31%
37Ar + H → 30Si
Flux impact:
Si 0.22%
37Ar + H → 30P*
Flux impact:
Si 0.11%
38Ar + H → 19F
Flux impact:
F 0.11%
38Ar + H → 23Na
Flux impact:
Na 0.19%
38Ar + H → 24Mg
[We98b]
Flux impact:
Mg 0.12%
GP12up22
GP12
GP22
σ [mb]
Ek/n [GeV/n]

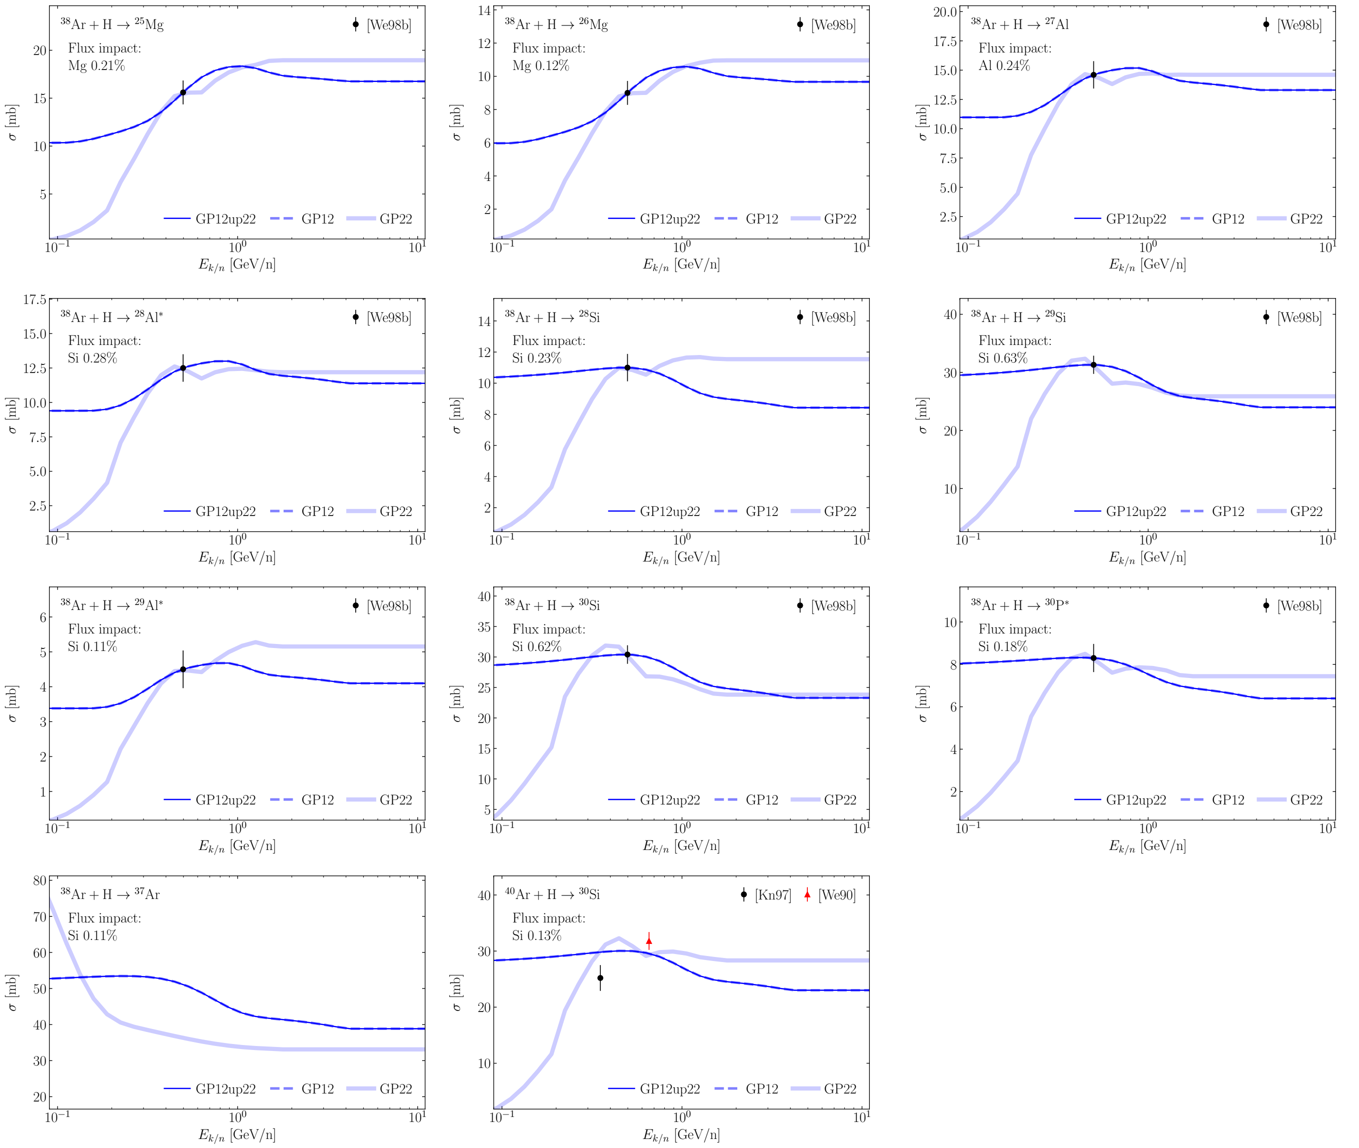


## Z=19 projectiles: $^{x}$K + H $\rightarrow\, ^{A}_{Z}X$

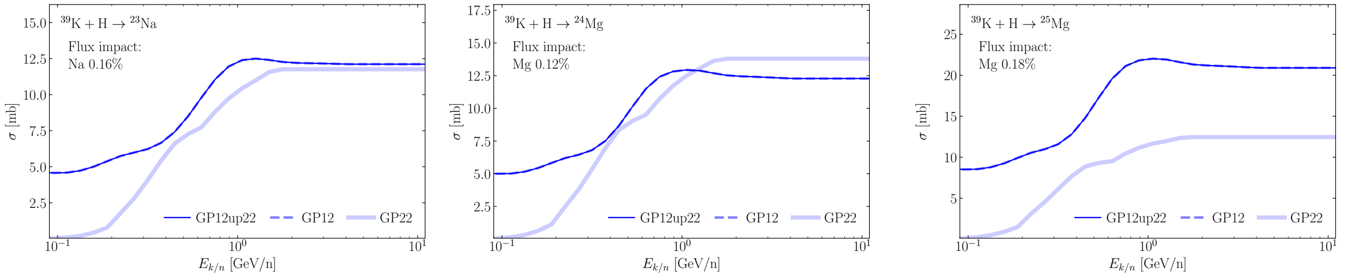

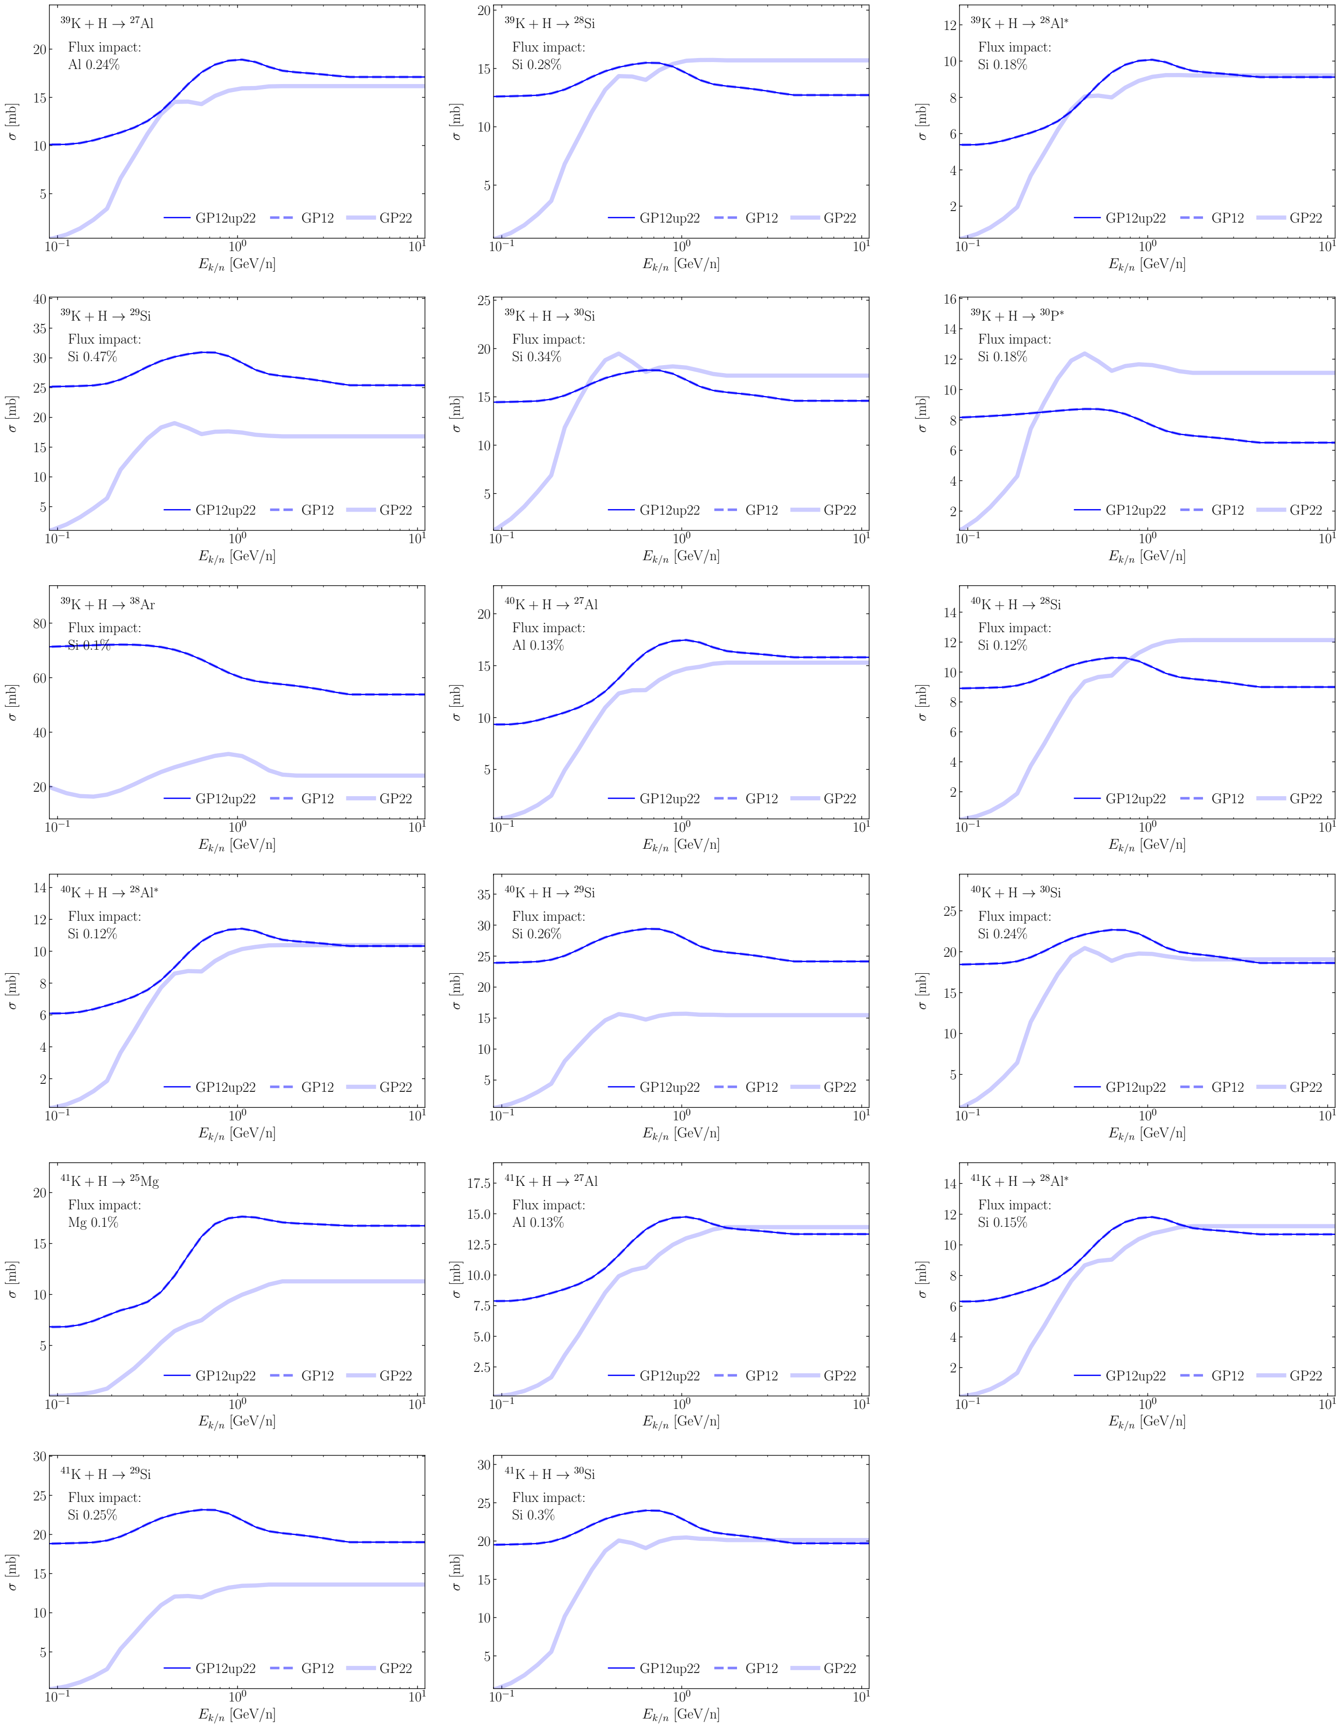


**Z=20 projectiles: $^{x}$Ca + H → $^{A}_{Z}X$**

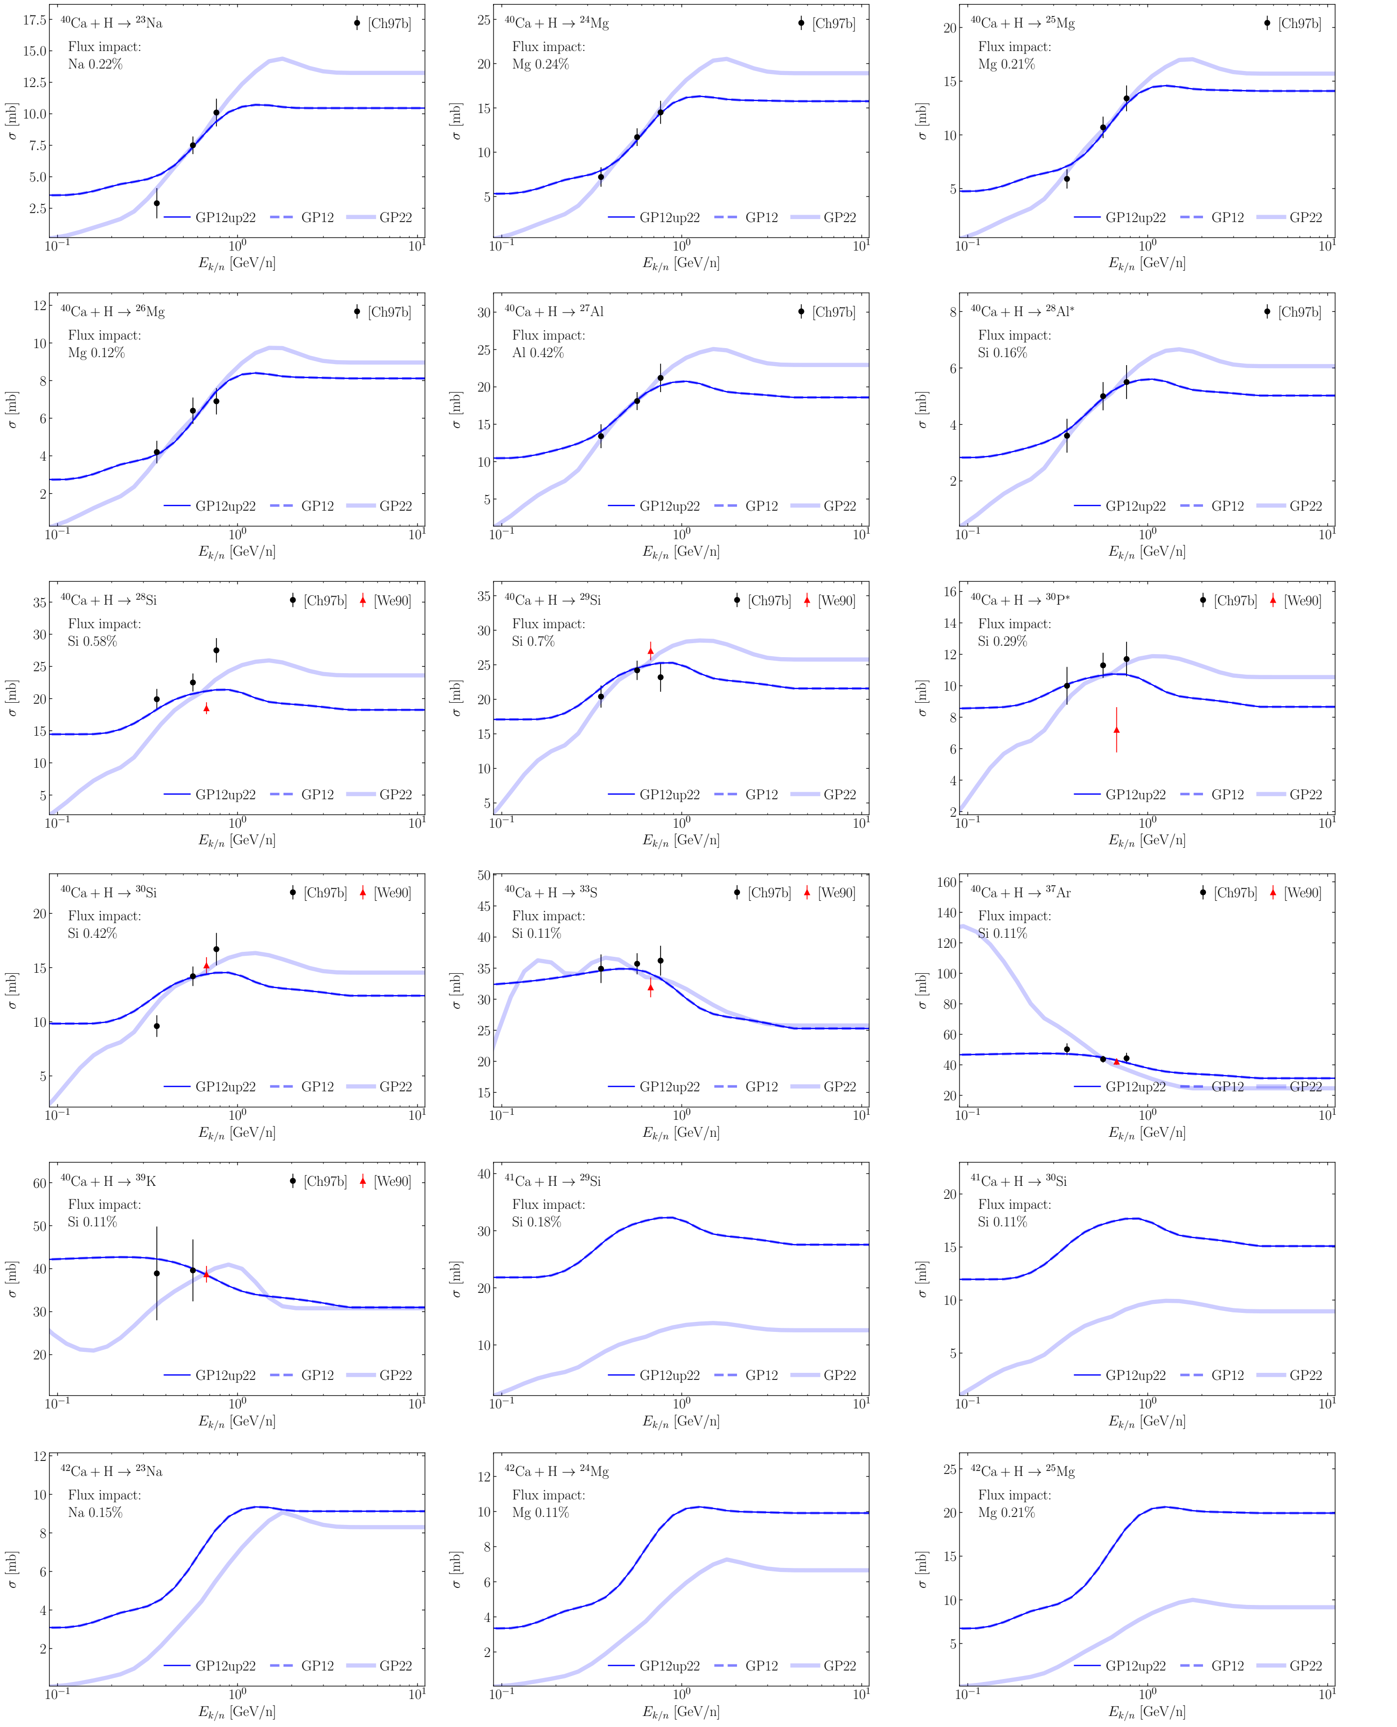

$^{40}$Ca + H → $^{23}$Na
Flux impact:
Na 0.22%
$^{40}$Ca + H → $^{24}$Mg
Flux impact:
Mg 0.24%
$^{40}$Ca + H → $^{25}$Mg
Flux impact:
Mg 0.21%
$^{40}$Ca + H → $^{26}$Mg
Flux impact:
Mg 0.12%
$^{40}$Ca + H → $^{27}$Al
Flux impact:
Al 0.42%
$^{40}$Ca + H → $^{28}$Al*
Flux impact:
Si 0.16%
$^{40}$Ca + H → $^{28}$Si
Flux impact:
Si 0.58%
$^{40}$Ca + H → $^{29}$Si
Flux impact:
Si 0.7%
$^{40}$Ca + H → $^{30}$P*
Flux impact:
Si 0.29%
$^{40}$Ca + H → $^{30}$Si
Flux impact:
Si 0.42%
$^{40}$Ca + H → $^{33}$S
Flux impact:
Si 0.11%
$^{40}$Ca + H → $^{37}$Ar
Flux impact:
Si 0.11%
$^{40}$Ca + H → $^{39}$K
Flux impact:
Si 0.11%
$^{41}$Ca + H → $^{29}$Si
Flux impact:
Si 0.18%
$^{41}$Ca + H → $^{30}$Si
Flux impact:
Si 0.11%
$^{42}$Ca + H → $^{23}$Na
Flux impact:
Na 0.15%
$^{42}$Ca + H → $^{24}$Mg
Flux impact:
Mg 0.11%
$^{42}$Ca + H → $^{25}$Mg
Flux impact:
Mg 0.21%
[Ch97b]
[We90]
GP12up22
GP12
GP22
$\sigma$ [mb]
$E_{k/n}$ [GeV/n]

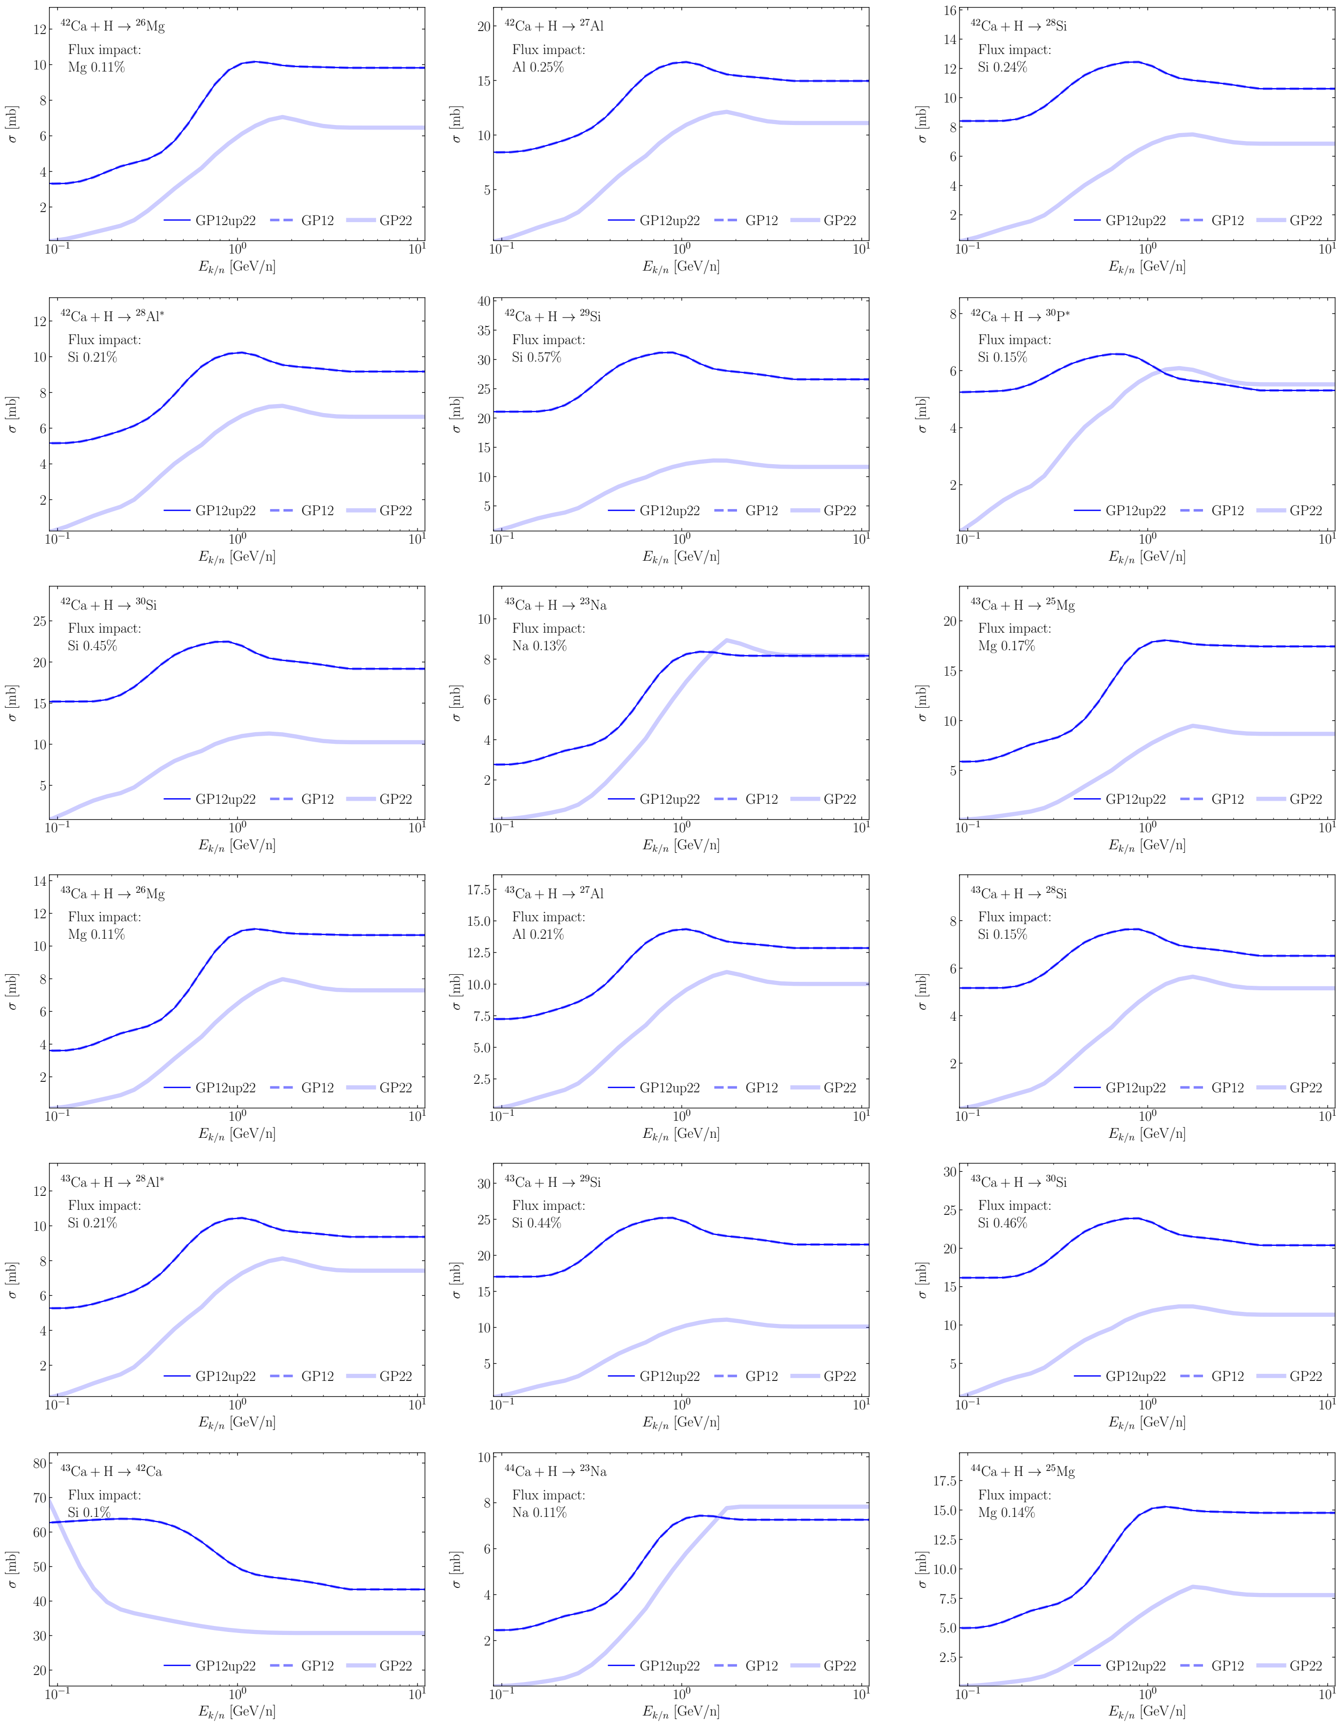

$^{42}$Ca + H → $^{26}$Mg
Flux impact: Mg 0.11%
$^{42}$Ca + H → $^{27}$Al
Flux impact: Al 0.25%
$^{42}$Ca + H → $^{28}$Si
Flux impact: Si 0.24%
$^{42}$Ca + H → $^{28}$Al*
Flux impact: Si 0.21%
$^{42}$Ca + H → $^{29}$Si
Flux impact: Si 0.57%
$^{42}$Ca + H → $^{30}$P*
Flux impact: Si 0.15%
$^{42}$Ca + H → $^{30}$Si
Flux impact: Si 0.45%
$^{43}$Ca + H → $^{23}$Na
Flux impact: Na 0.13%
$^{43}$Ca + H → $^{25}$Mg
Flux impact: Mg 0.17%
$^{43}$Ca + H → $^{26}$Mg
Flux impact: Mg 0.11%
$^{43}$Ca + H → $^{27}$Al
Flux impact: Al 0.21%
$^{43}$Ca + H → $^{28}$Si
Flux impact: Si 0.15%
$^{43}$Ca + H → $^{28}$Al*
Flux impact: Si 0.21%
$^{43}$Ca + H → $^{29}$Si
Flux impact: Si 0.44%
$^{43}$Ca + H → $^{30}$Si
Flux impact: Si 0.46%
$^{43}$Ca + H → $^{42}$Ca
Flux impact: Si 0.1%
$^{44}$Ca + H → $^{23}$Na
Flux impact: Na 0.11%
$^{44}$Ca + H → $^{25}$Mg
Flux impact: Mg 0.14%
GP12up22
GP12
GP22
$\sigma$ [mb]
$E_{k/n}$ [GeV/n]

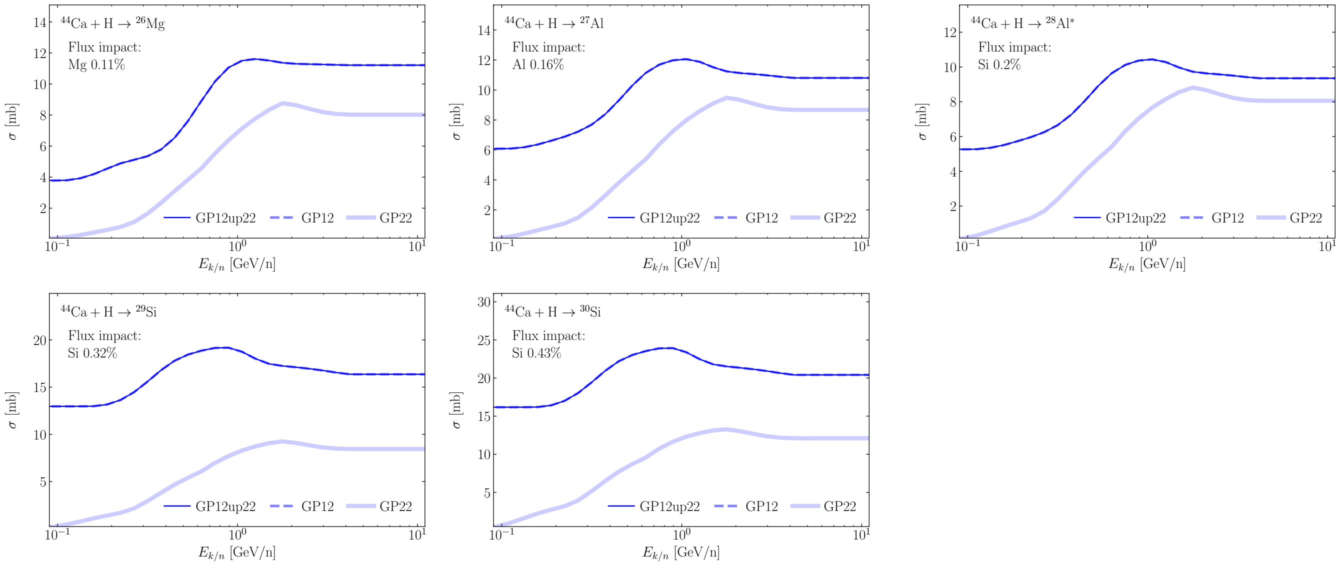


## Z=21 projectiles: $^{x}$Sc + H → $^{A}_{Z}X$

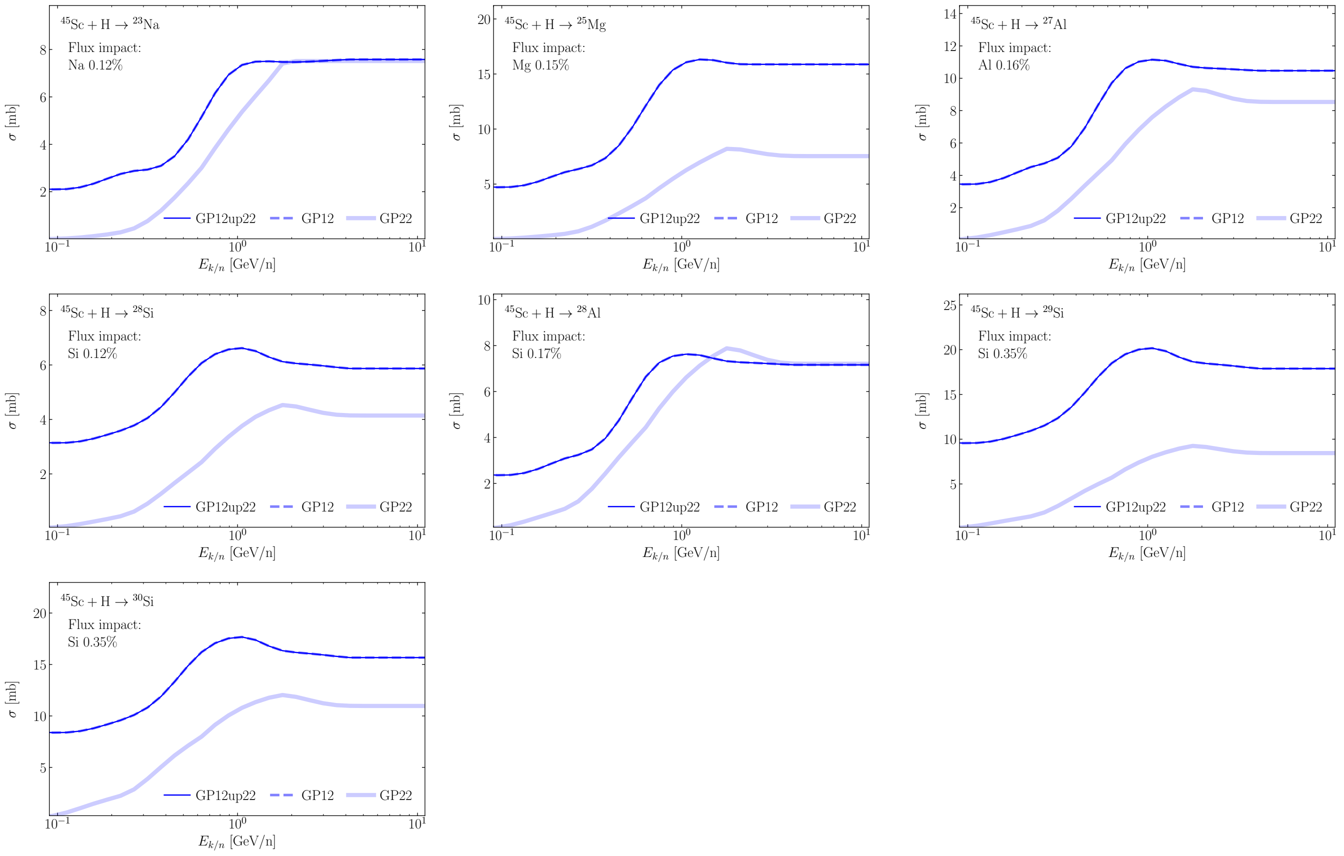


## Z=22 projectiles: $^{x}$Ti + H → $^{A}_{Z}X$

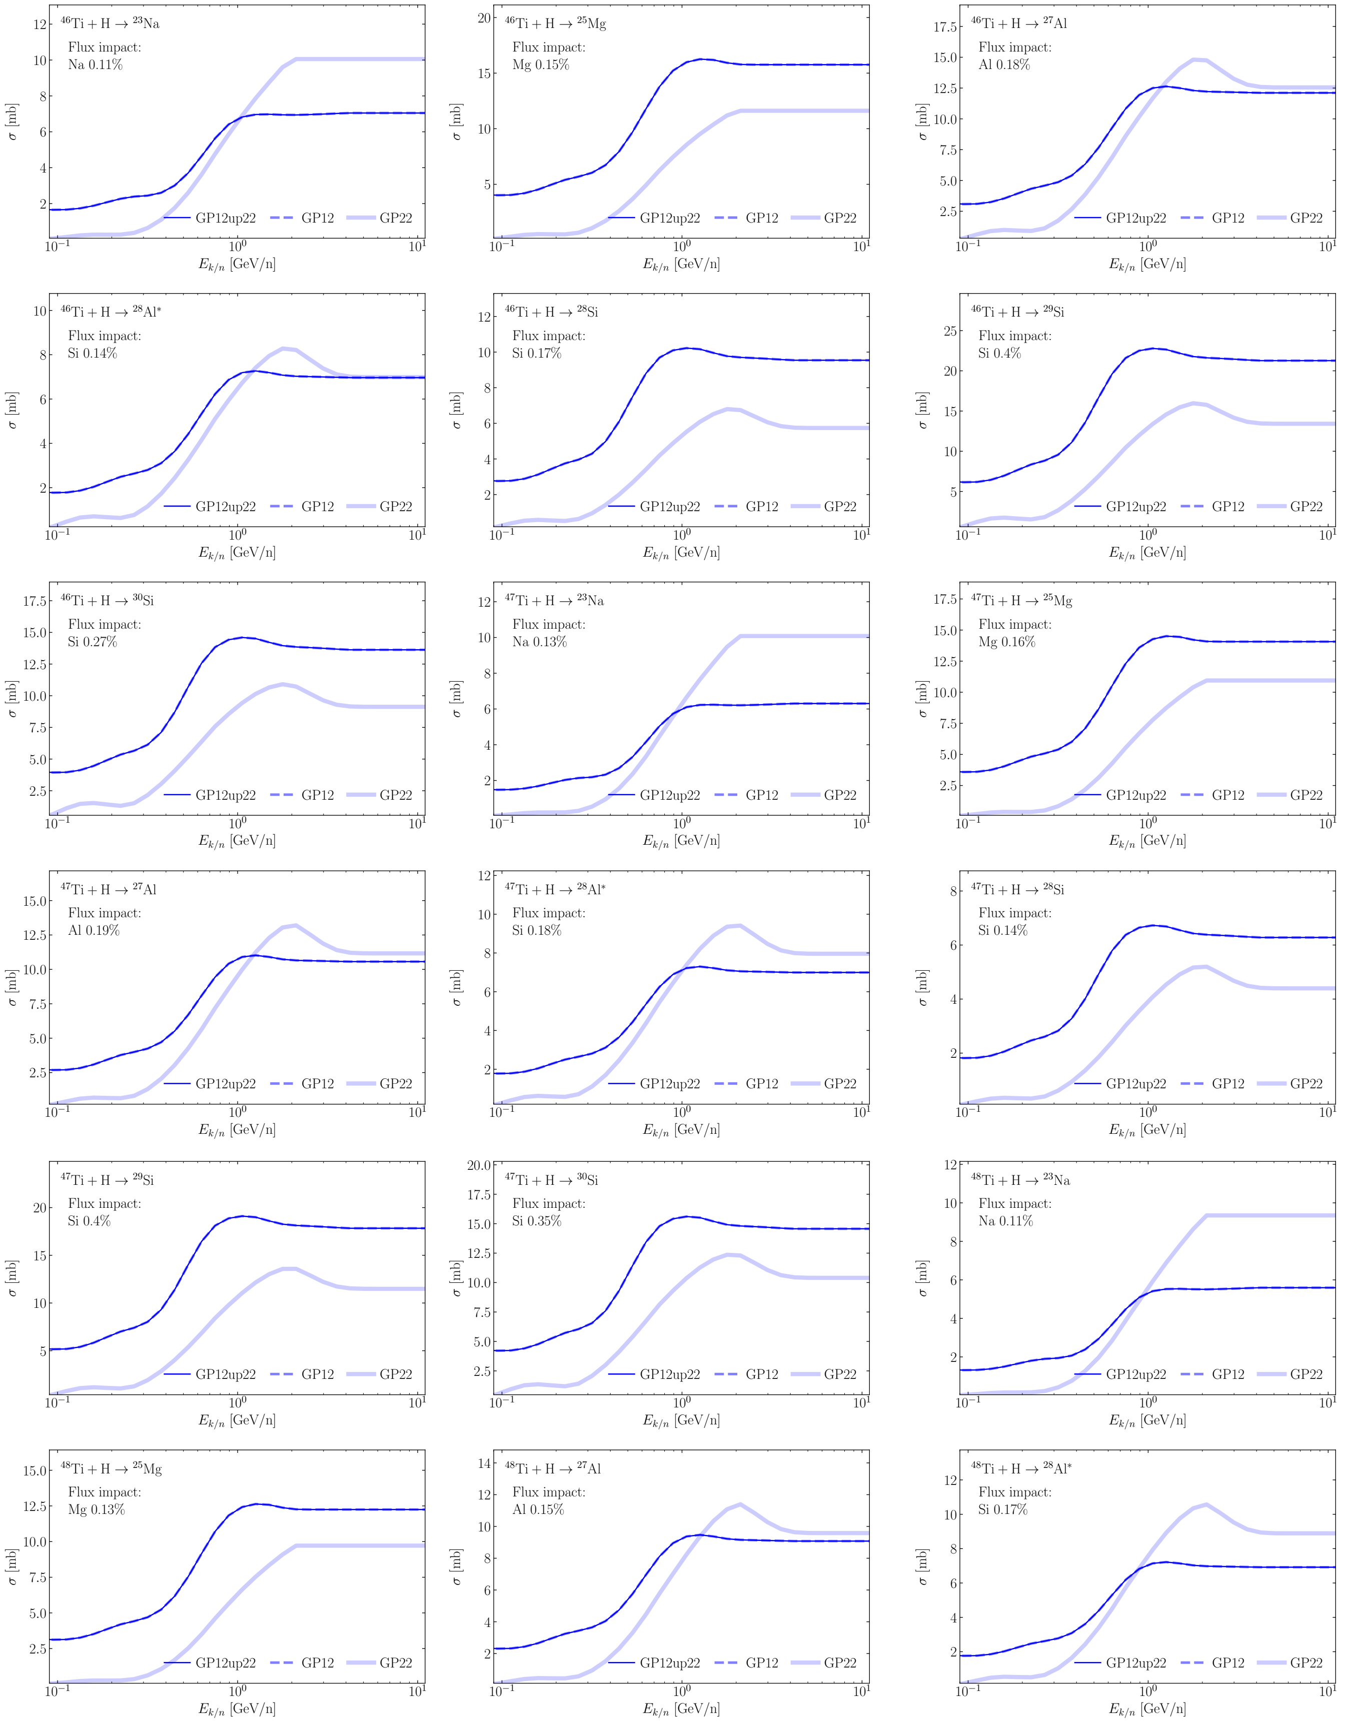

$^{46}Ti + H \rightarrow {}^{23}Na$
Flux impact: Na 0.11%
$^{46}Ti + H \rightarrow {}^{25}Mg$
Flux impact: Mg 0.15%
$^{46}Ti + H \rightarrow {}^{27}Al$
Flux impact: Al 0.18%
$^{46}Ti + H \rightarrow {}^{28}Al^{*}$
Flux impact: Si 0.14%
$^{46}Ti + H \rightarrow {}^{28}Si$
Flux impact: Si 0.17%
$^{46}Ti + H \rightarrow {}^{29}Si$
Flux impact: Si 0.4%
$^{46}Ti + H \rightarrow {}^{30}Si$
Flux impact: Si 0.27%
$^{47}Ti + H \rightarrow {}^{23}Na$
Flux impact: Na 0.13%
$^{47}Ti + H \rightarrow {}^{25}Mg$
Flux impact: Mg 0.16%
$^{47}Ti + H \rightarrow {}^{27}Al$
Flux impact: Al 0.19%
$^{47}Ti + H \rightarrow {}^{28}Al^{*}$
Flux impact: Si 0.18%
$^{47}Ti + H \rightarrow {}^{28}Si$
Flux impact: Si 0.14%
$^{47}Ti + H \rightarrow {}^{29}Si$
Flux impact: Si 0.4%
$^{47}Ti + H \rightarrow {}^{30}Si$
Flux impact: Si 0.35%
$^{48}Ti + H \rightarrow {}^{23}Na$
Flux impact: Na 0.11%
$^{48}Ti + H \rightarrow {}^{25}Mg$
Flux impact: Mg 0.13%
$^{48}Ti + H \rightarrow {}^{27}Al$
Flux impact: Al 0.15%
$^{48}Ti + H \rightarrow {}^{28}Al^{*}$
Flux impact: Si 0.17%
GP12up22
GP12
GP22
$\sigma$ [mb]
$E_{k/n}$ [GeV/n]

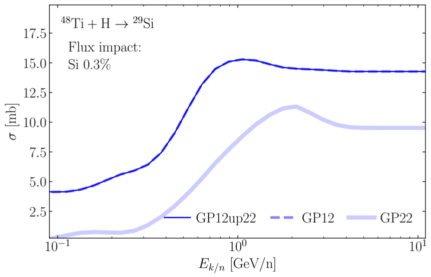


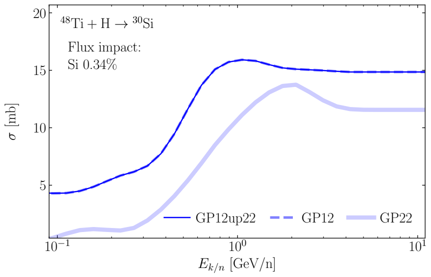


## Z=23 projectiles: $^{x}$V + H $\to {}^{A}_{Z}X$

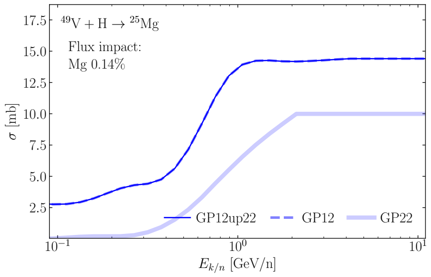


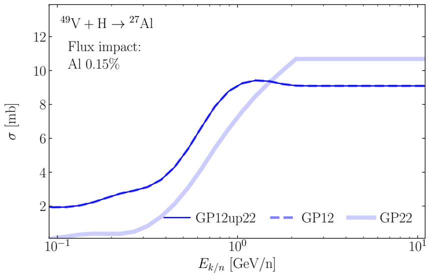


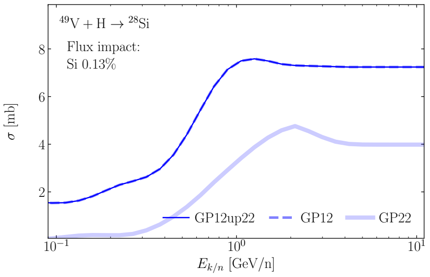


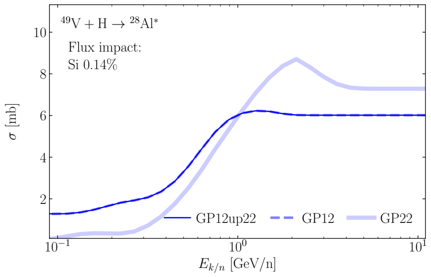


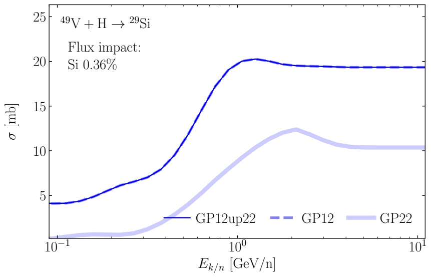


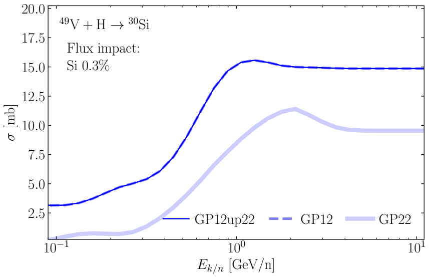


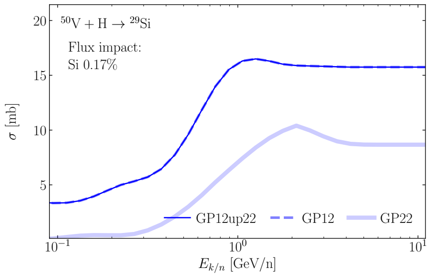


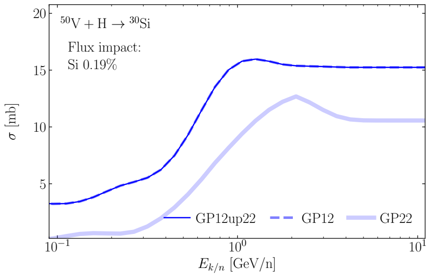


## Z=24 projectiles: $^{x}$Cr + H $\to {}^{A}_{Z}X$

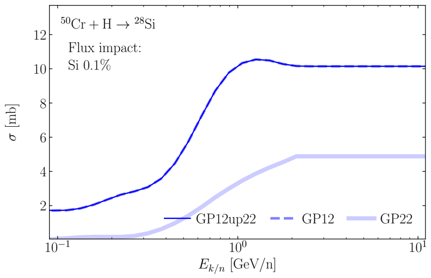


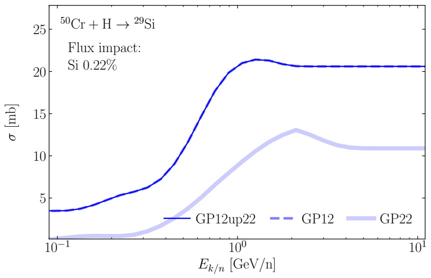


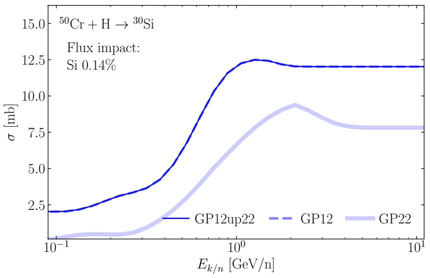

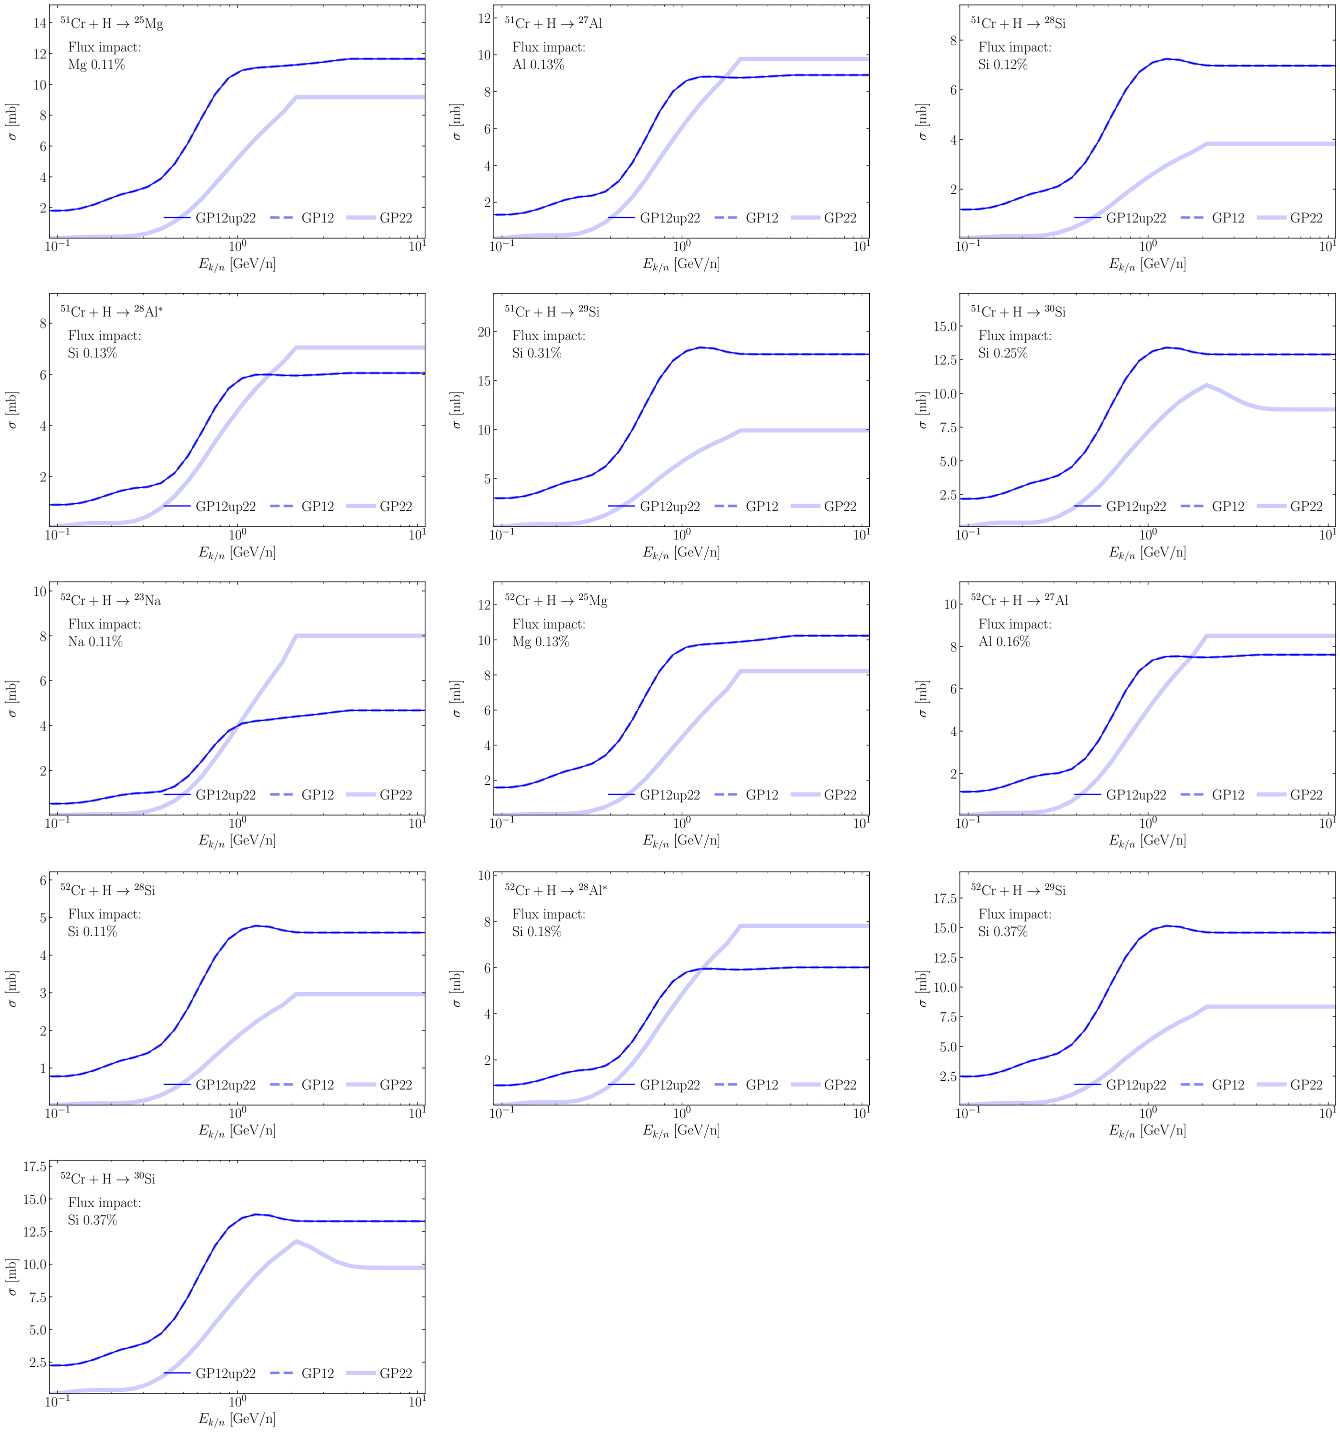


## Z=25 projectiles: $^{x}$Mn + H → $^{A}_{Z}X$

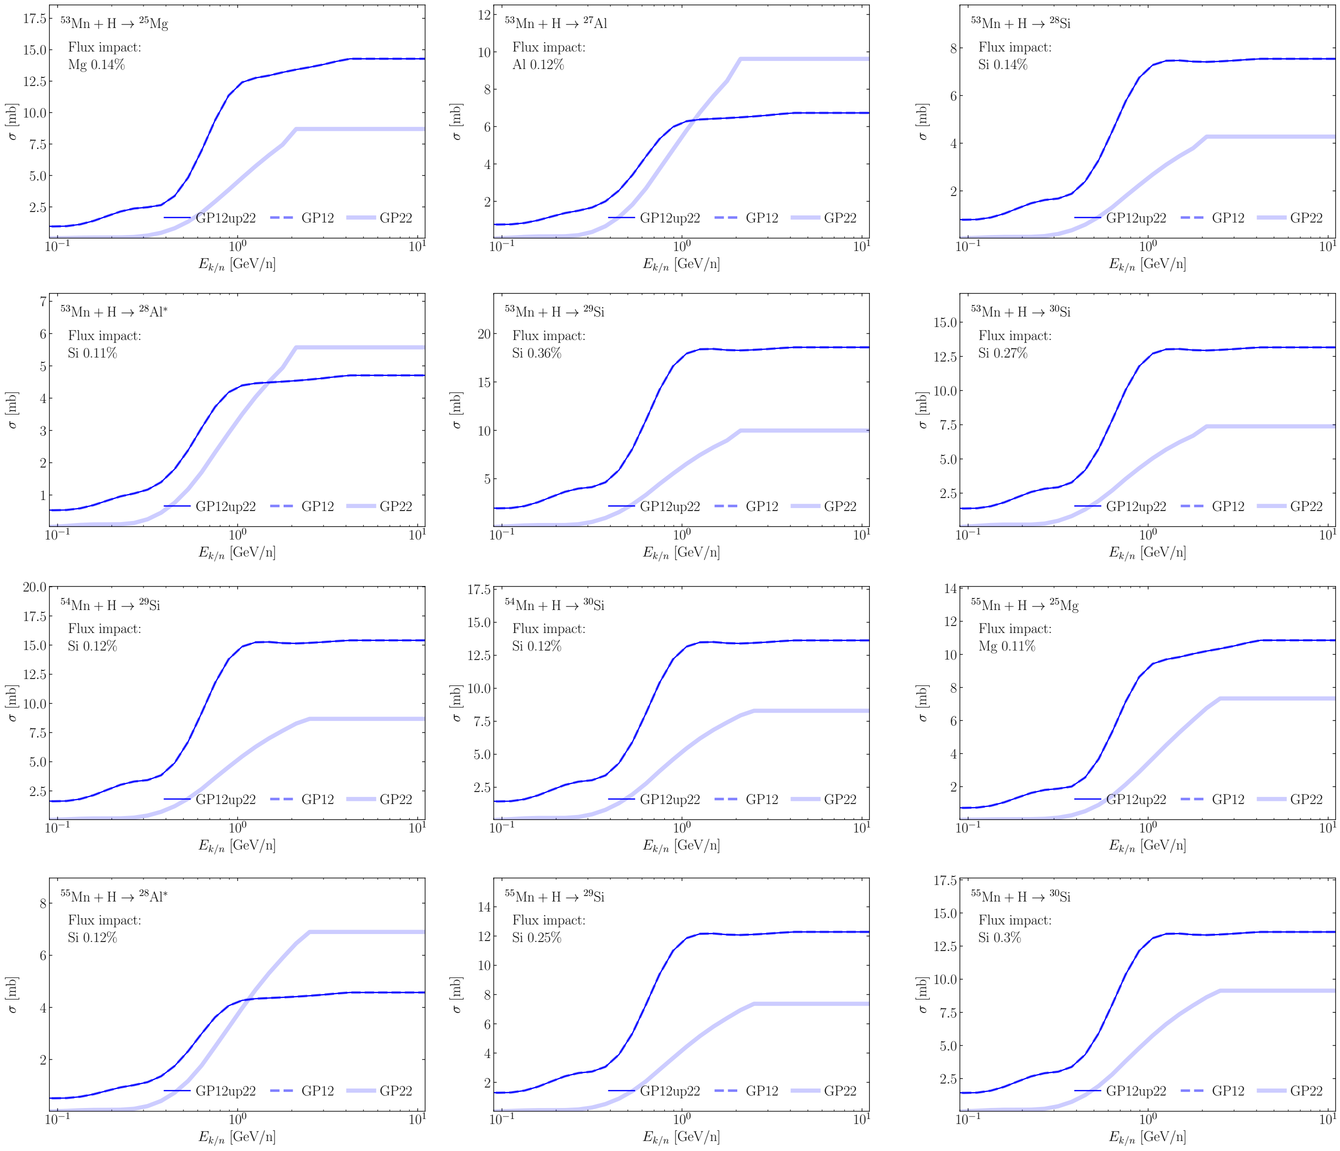


## Z=26 projectiles: $^{x}$Fe + H → $^{A}_{Z}X$

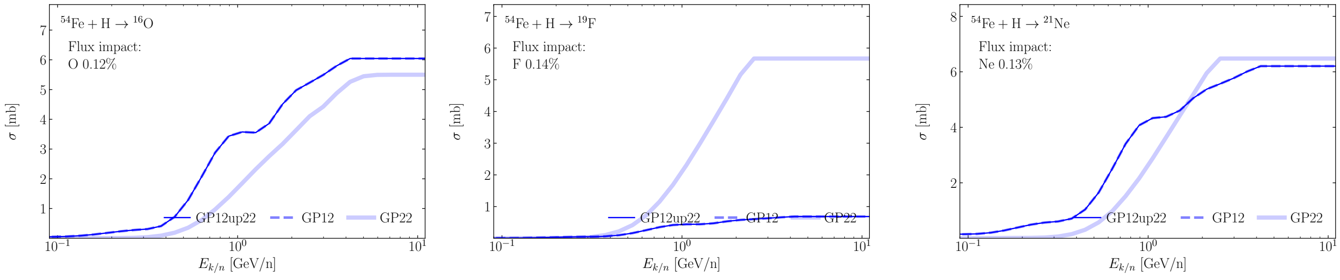

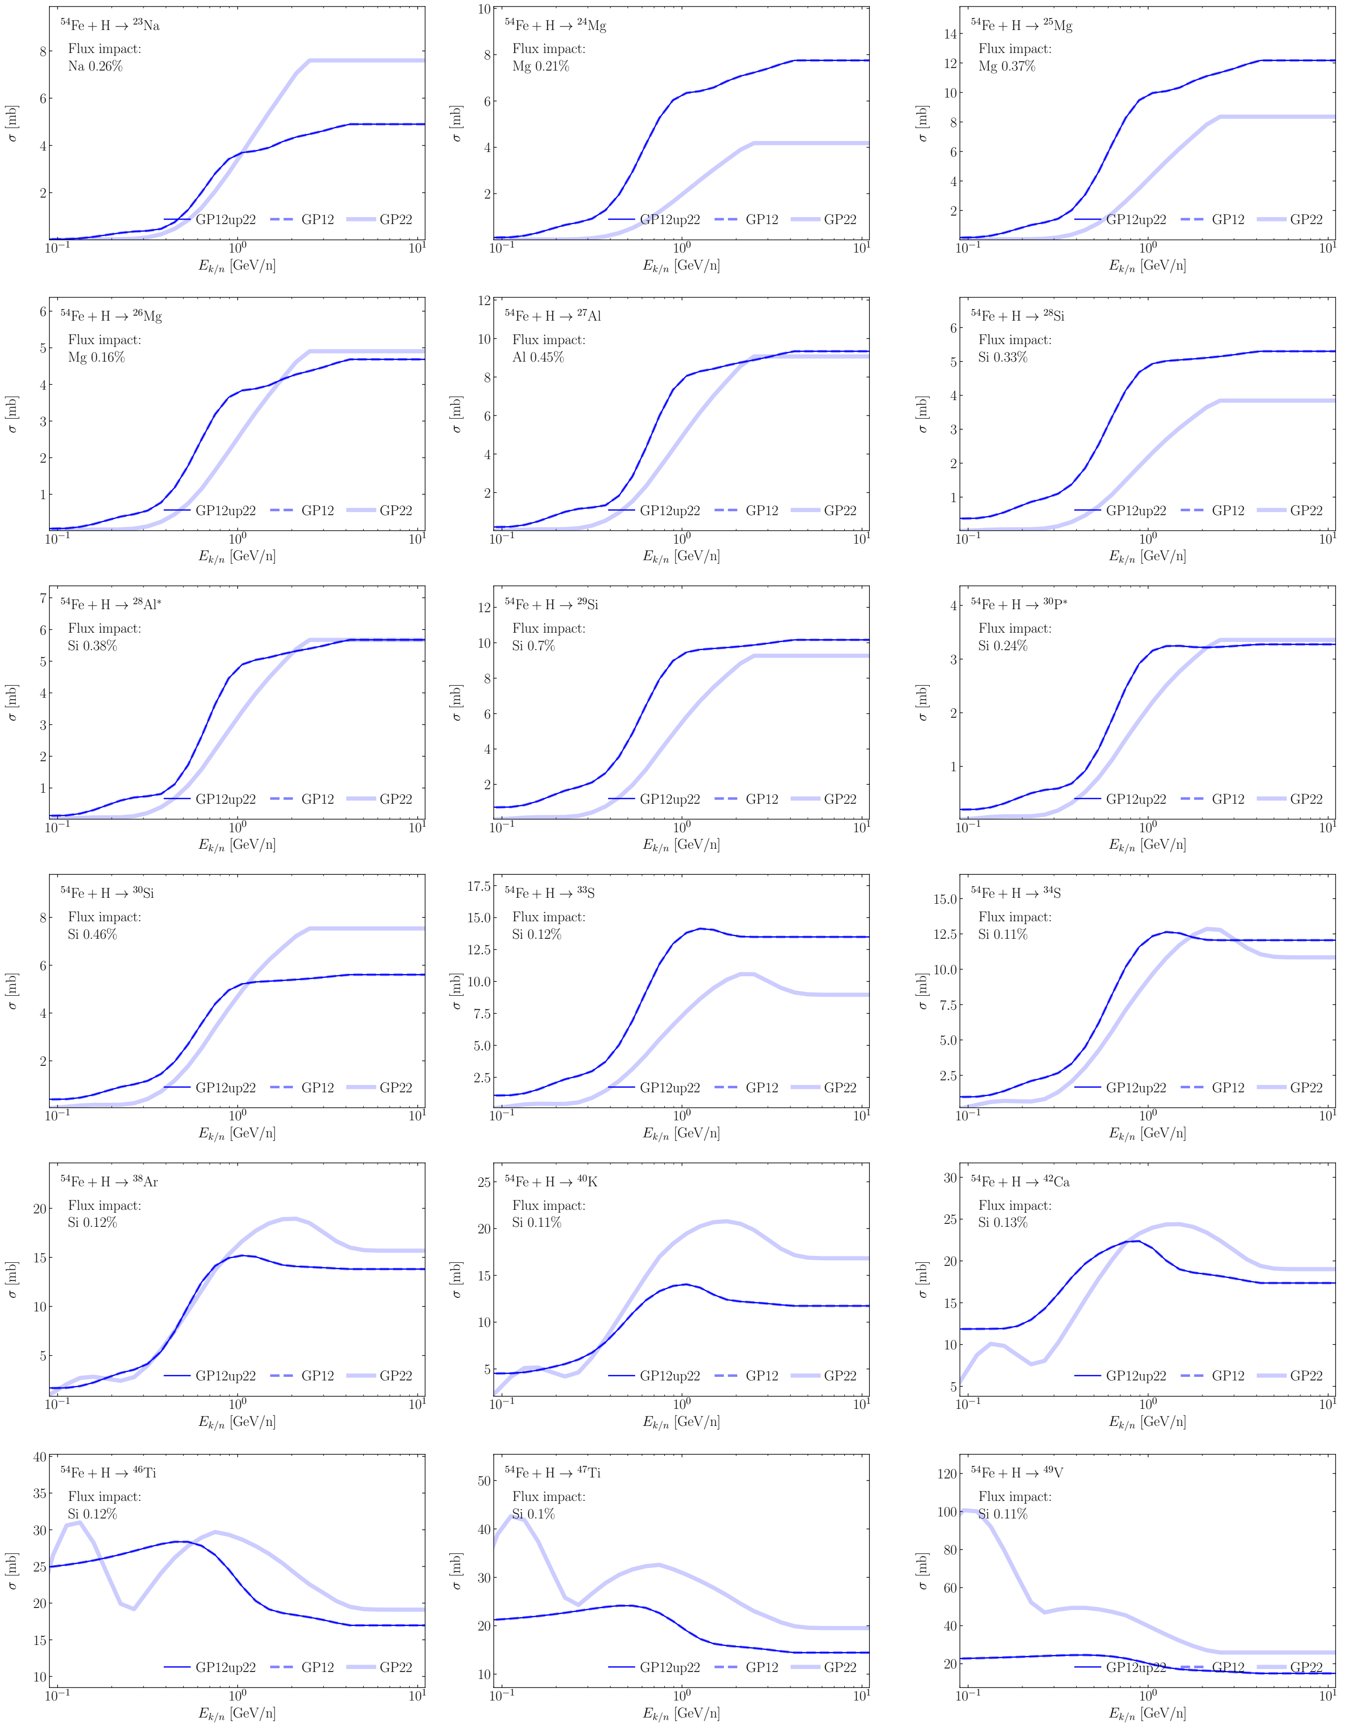

$^{54}$Fe + H → $^{23}$Na
Flux impact: Na 0.26%
$^{54}$Fe + H → $^{24}$Mg
Flux impact: Mg 0.21%
$^{54}$Fe + H → $^{25}$Mg
Flux impact: Mg 0.37%
$^{54}$Fe + H → $^{26}$Mg
Flux impact: Mg 0.16%
$^{54}$Fe + H → $^{27}$Al
Flux impact: Al 0.45%
$^{54}$Fe + H → $^{28}$Si
Flux impact: Si 0.33%
$^{54}$Fe + H → $^{28}$Al*
Flux impact: Si 0.38%
$^{54}$Fe + H → $^{29}$Si
Flux impact: Si 0.7%
$^{54}$Fe + H → $^{30}$P*
Flux impact: Si 0.24%
$^{54}$Fe + H → $^{30}$Si
Flux impact: Si 0.46%
$^{54}$Fe + H → $^{33}$S
Flux impact: Si 0.12%
$^{54}$Fe + H → $^{34}$S
Flux impact: Si 0.11%
$^{54}$Fe + H → $^{38}$Ar
Flux impact: Si 0.12%
$^{54}$Fe + H → $^{40}$K
Flux impact: Si 0.11%
$^{54}$Fe + H → $^{42}$Ca
Flux impact: Si 0.13%
$^{54}$Fe + H → $^{46}$Ti
Flux impact: Si 0.12%
$^{54}$Fe + H → $^{47}$Ti
Flux impact: Si 0.1%
$^{54}$Fe + H → $^{49}$V
Flux impact: Si 0.11%
GP12up22
GP12
GP22
$\sigma$ [mb]
$E_{k/n}$ [GeV/n]

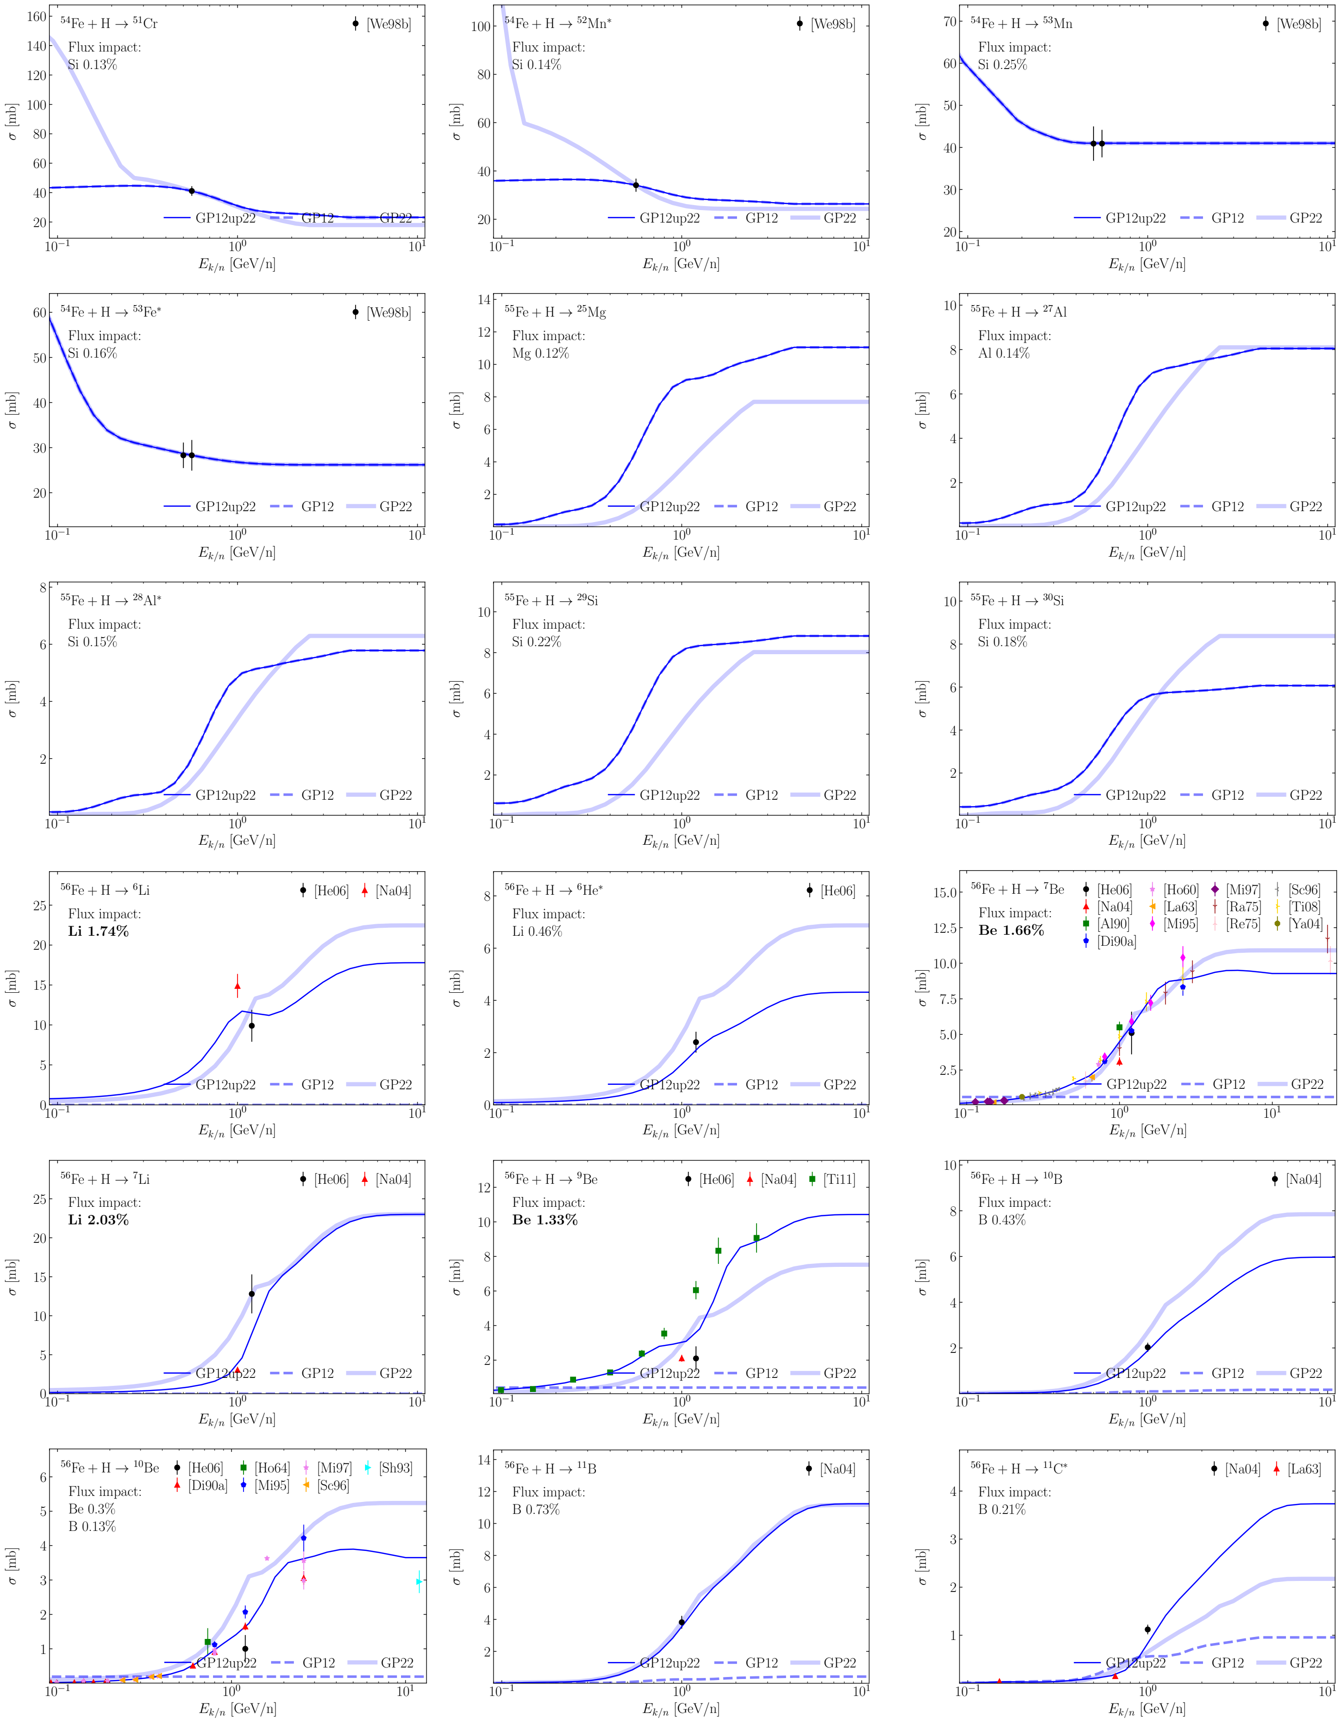

54Fe + H → 51Cr
Flux impact: Si 0.13%
[We98b]
54Fe + H → 52Mn*
Flux impact: Si 0.14%
[We98b]
54Fe + H → 53Mn
Flux impact: Si 0.25%
[We98b]
54Fe + H → 53Fe*
Flux impact: Si 0.16%
[We98b]
55Fe + H → 25Mg
Flux impact: Mg 0.12%
55Fe + H → 27Al
Flux impact: Al 0.14%
55Fe + H → 28Al*
Flux impact: Si 0.15%
55Fe + H → 29Si
Flux impact: Si 0.22%
55Fe + H → 30Si
Flux impact: Si 0.18%
56Fe + H → 6Li
Flux impact: Li 1.74%
[He06] [Na04]
56Fe + H → 6He*
Flux impact: Li 0.46%
[He06]
56Fe + H → 7Be
Flux impact: Be 1.66%
[He06] [Na04] [Al90] [Di90a] [Ho60] [La63] [Mi95] [Mi97] [Ra75] [Re75] [Sc96] [Ti08] [Ya04]
56Fe + H → 7Li
Flux impact: Li 2.03%
[He06] [Na04]
56Fe + H → 9Be
Flux impact: Be 1.33%
[He06] [Na04] [Ti11]
56Fe + H → 10B
Flux impact: B 0.43%
[Na04]
56Fe + H → 10Be
Flux impact: Be 0.3% B 0.13%
[He06] [Di90a] [Ho64] [Mi95] [Mi97] [Sc96] [Sh93]
56Fe + H → 11B
Flux impact: B 0.73%
[Na04]
56Fe + H → 11C*
Flux impact: B 0.21%
[Na04] [La63]
GP12up22
GP12
GP22
σ [mb]
Ek/n [GeV/n]

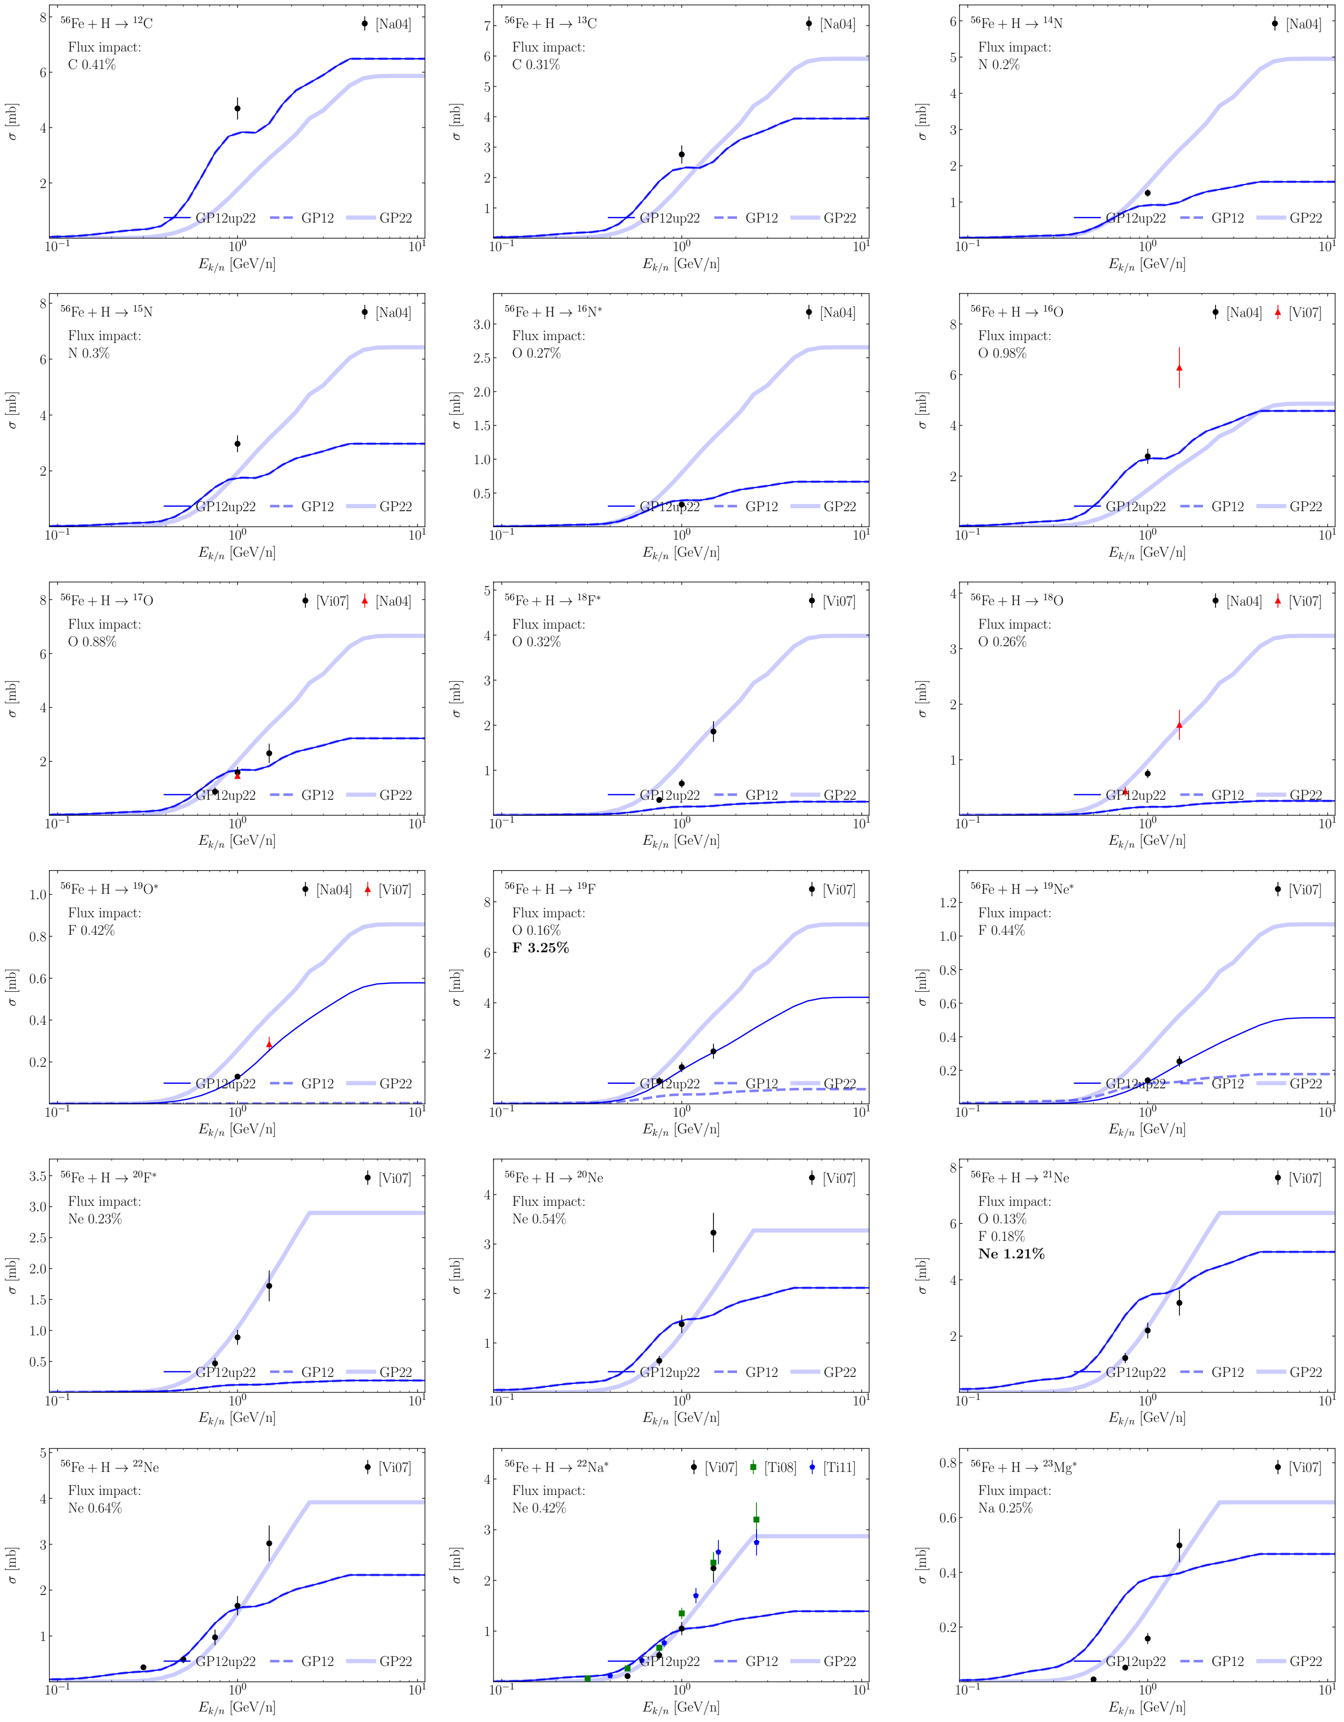

56Fe + H → 12C
[Na04]
Flux impact:
C 0.41%
56Fe + H → 13C
[Na04]
Flux impact:
C 0.31%
56Fe + H → 14N
[Na04]
Flux impact:
N 0.2%
56Fe + H → 15N
[Na04]
Flux impact:
N 0.3%
56Fe + H → 16N*
[Na04]
Flux impact:
O 0.27%
56Fe + H → 16O
[Na04] [Vi07]
Flux impact:
O 0.98%
56Fe + H → 17O
[Vi07] [Na04]
Flux impact:
O 0.88%
56Fe + H → 18F*
[Vi07]
Flux impact:
O 0.32%
56Fe + H → 18O
[Na04] [Vi07]
Flux impact:
O 0.26%
56Fe + H → 19O*
[Na04] [Vi07]
Flux impact:
F 0.42%
56Fe + H → 19F
[Vi07]
Flux impact:
O 0.16%
F 3.25%
56Fe + H → 19Ne*
[Vi07]
Flux impact:
F 0.44%
56Fe + H → 20F*
[Vi07]
Flux impact:
Ne 0.23%
56Fe + H → 20Ne
[Vi07]
Flux impact:
Ne 0.54%
56Fe + H → 21Ne
[Vi07]
Flux impact:
O 0.13%
F 0.18%
Ne 1.21%
56Fe + H → 22Ne
[Vi07]
Flux impact:
Ne 0.64%
56Fe + H → 22Na*
[Vi07] [Ti08] [Ti11]
Flux impact:
Ne 0.42%
56Fe + H → 23Mg*
[Vi07]
Flux impact:
Na 0.25%
GP12up22 GP12 GP22
σ [mb]
E_{k/n} [GeV/n]

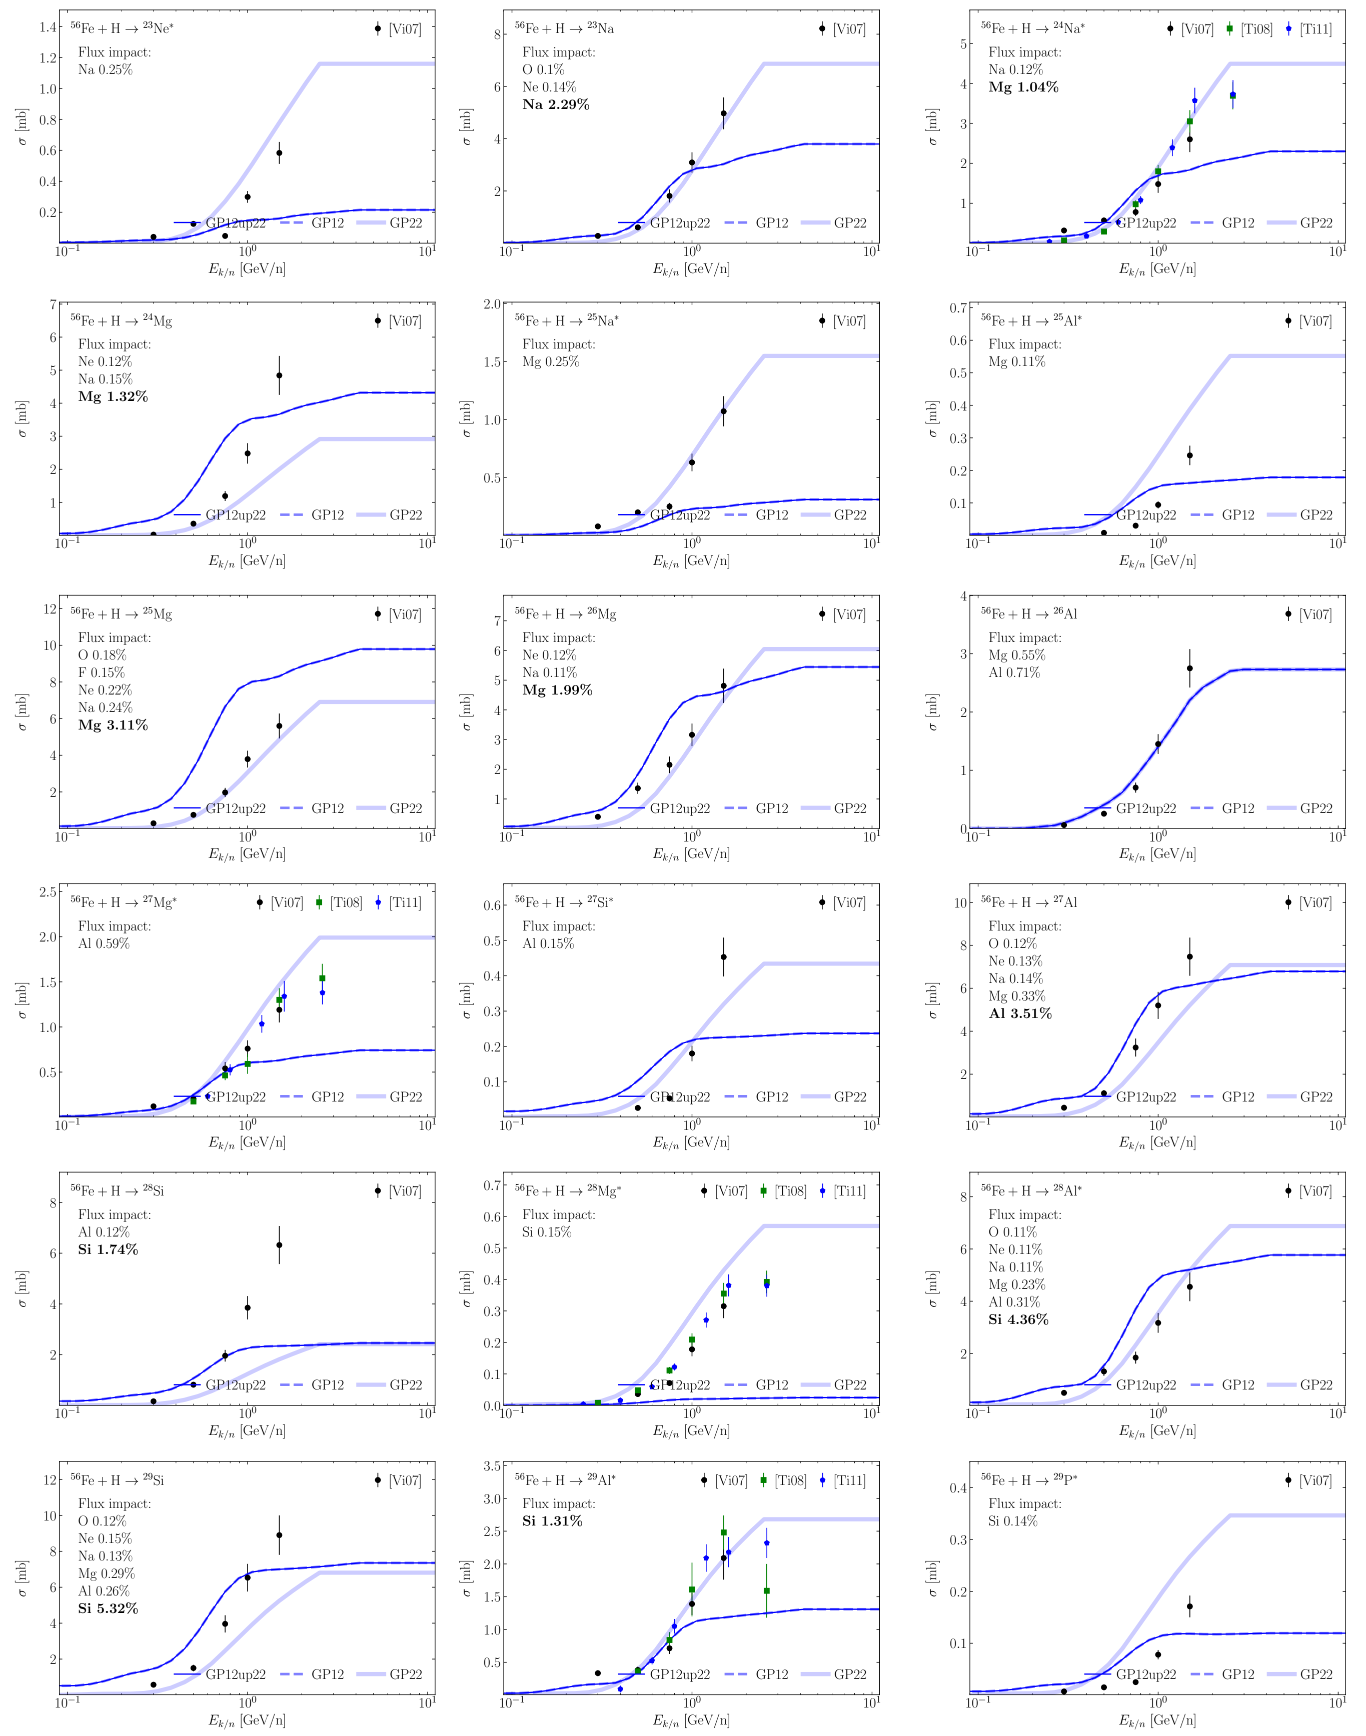

$^{56}$Fe + H → $^{23}$Ne*
[Vi07]
Flux impact:
Na 0.25%
$^{56}$Fe + H → $^{23}$Na
[Vi07]
Flux impact:
O 0.1%
Ne 0.14%
Na 2.29%
$^{56}$Fe + H → $^{24}$Na*
[Vi07] [Ti08] [Ti11]
Flux impact:
Na 0.12%
Mg 1.04%
$^{56}$Fe + H → $^{24}$Mg
[Vi07]
Flux impact:
Ne 0.12%
Na 0.15%
Mg 1.32%
$^{56}$Fe + H → $^{25}$Na*
[Vi07]
Flux impact:
Mg 0.25%
$^{56}$Fe + H → $^{25}$Al*
[Vi07]
Flux impact:
Mg 0.11%
$^{56}$Fe + H → $^{25}$Mg
[Vi07]
Flux impact:
O 0.18%
F 0.15%
Ne 0.22%
Na 0.24%
Mg 3.11%
$^{56}$Fe + H → $^{26}$Mg
[Vi07]
Flux impact:
Ne 0.12%
Na 0.11%
Mg 1.99%
$^{56}$Fe + H → $^{26}$Al
[Vi07]
Flux impact:
Mg 0.55%
Al 0.71%
$^{56}$Fe + H → $^{27}$Mg*
[Vi07] [Ti08] [Ti11]
Flux impact:
Al 0.59%
$^{56}$Fe + H → $^{27}$Si*
[Vi07]
Flux impact:
Al 0.15%
$^{56}$Fe + H → $^{27}$Al
[Vi07]
Flux impact:
O 0.12%
Ne 0.13%
Na 0.14%
Mg 0.33%
Al 3.51%
$^{56}$Fe + H → $^{28}$Si
[Vi07]
Flux impact:
Al 0.12%
Si 1.74%
$^{56}$Fe + H → $^{28}$Mg*
[Vi07] [Ti08] [Ti11]
Flux impact:
Si 0.15%
$^{56}$Fe + H → $^{28}$Al*
[Vi07]
Flux impact:
O 0.11%
Ne 0.11%
Na 0.11%
Mg 0.23%
Al 0.31%
Si 4.36%
$^{56}$Fe + H → $^{29}$Si
[Vi07]
Flux impact:
O 0.12%
Ne 0.15%
Na 0.13%
Mg 0.29%
Al 0.26%
Si 5.32%
$^{56}$Fe + H → $^{29}$Al*
[Vi07] [Ti08] [Ti11]
Flux impact:
Si 1.31%
$^{56}$Fe + H → $^{29}$P*
[Vi07]
Flux impact:
Si 0.14%
GP12up22
GP12
GP22
$\sigma$ [mb]
$E_{k/n}$ [GeV/n]

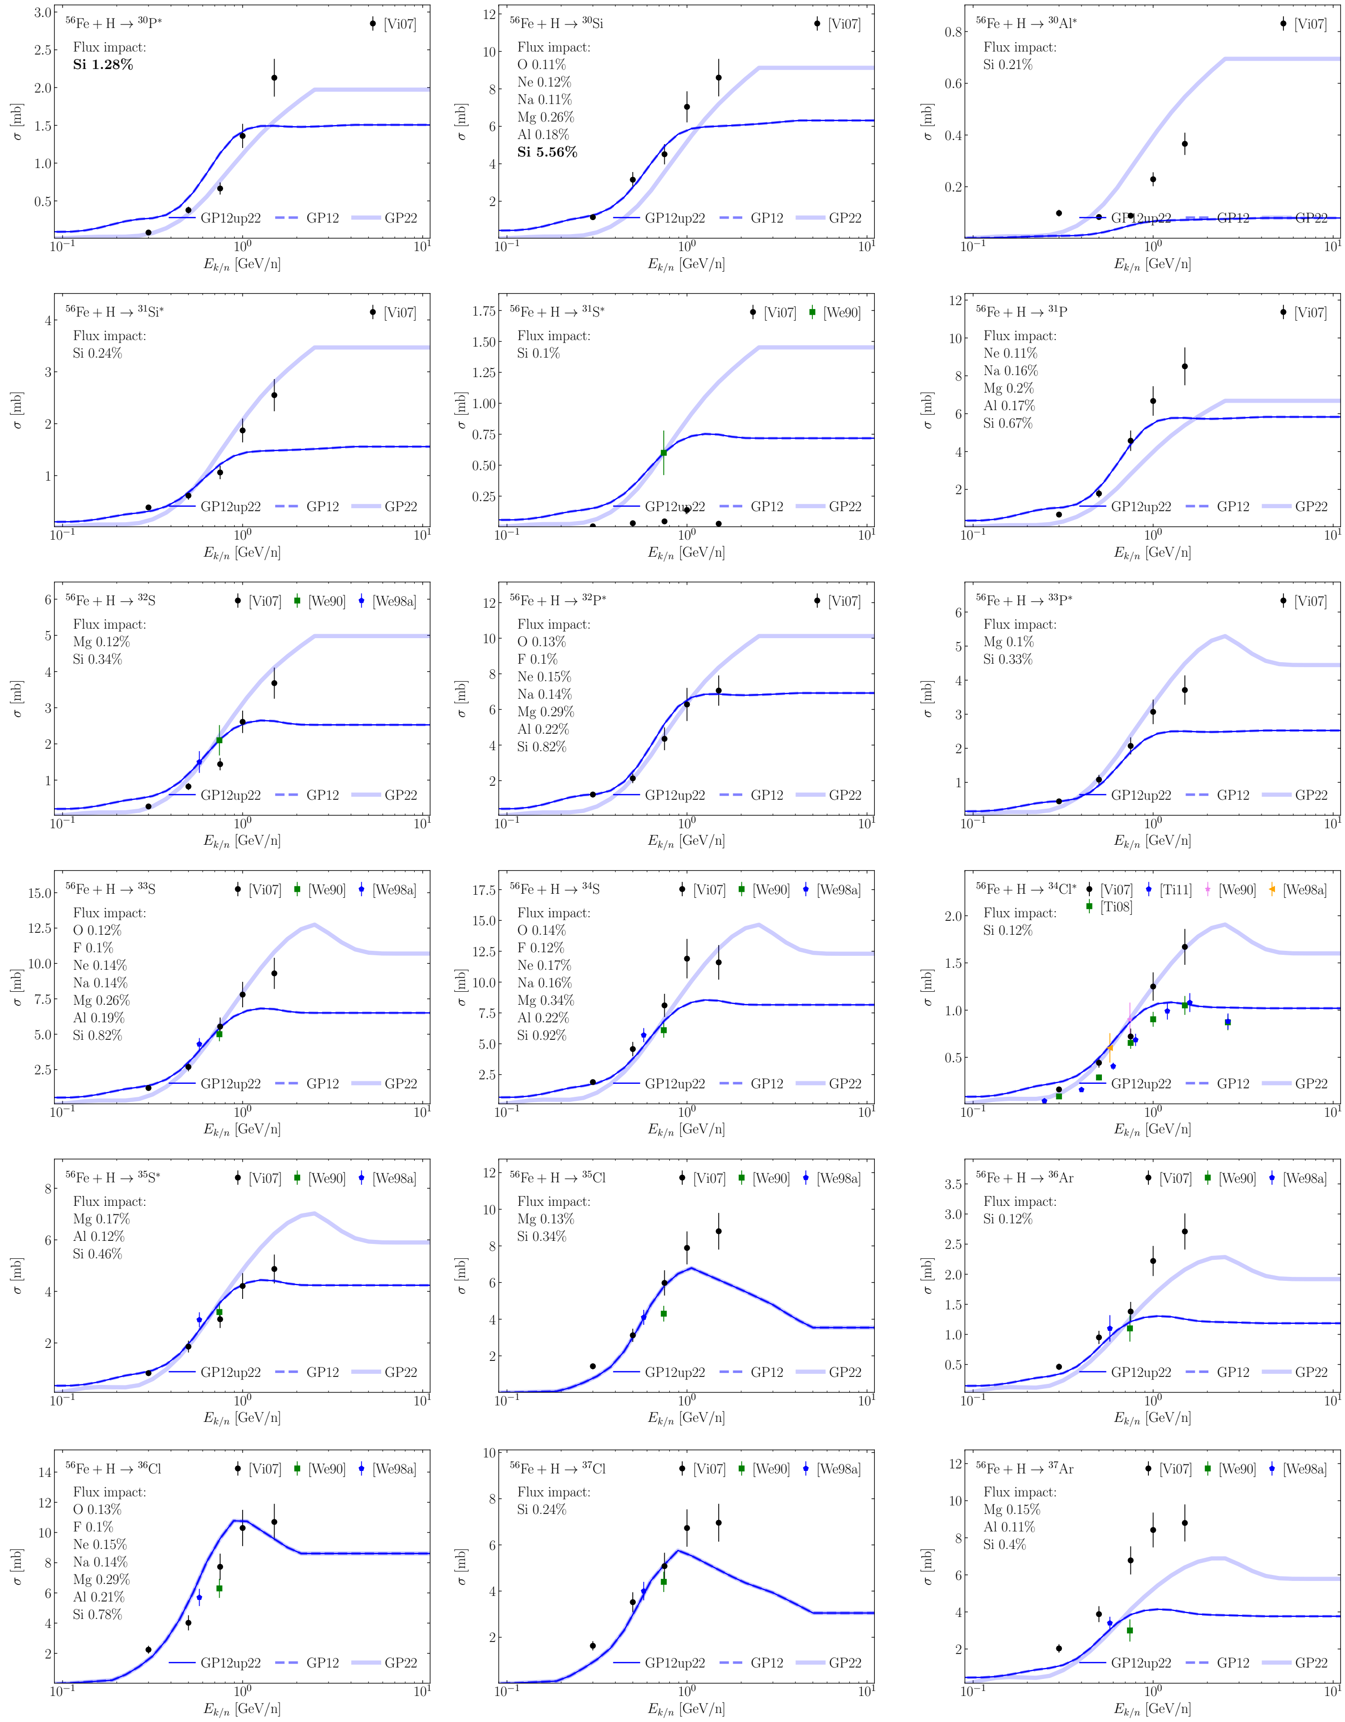
$^{56}$Fe + H → $^{30}$P*
[Vi07]
Flux impact:
**Si 1.28%**
$^{56}$Fe + H → $^{30}$Si
[Vi07]
Flux impact:
O 0.11%
Ne 0.12%
Na 0.11%
Mg 0.26%
Al 0.18%
**Si 5.56%**
$^{56}$Fe + H → $^{30}$Al*
[Vi07]
Flux impact:
Si 0.21%
$^{56}$Fe + H → $^{31}$Si*
[Vi07]
Flux impact:
Si 0.24%
$^{56}$Fe + H → $^{31}$S*
[Vi07] [We90]
Flux impact:
Si 0.1%
$^{56}$Fe + H → $^{31}$P
[Vi07]
Flux impact:
Ne 0.11%
Na 0.16%
Mg 0.2%
Al 0.17%
Si 0.67%
$^{56}$Fe + H → $^{32}$S
[Vi07] [We90] [We98a]
Flux impact:
Mg 0.12%
Si 0.34%
$^{56}$Fe + H → $^{32}$P*
[Vi07]
Flux impact:
O 0.13%
F 0.1%
Ne 0.15%
Na 0.14%
Mg 0.29%
Al 0.22%
Si 0.82%
$^{56}$Fe + H → $^{33}$P*
[Vi07]
Flux impact:
Mg 0.1%
Si 0.33%
$^{56}$Fe + H → $^{33}$S
[Vi07] [We90] [We98a]
Flux impact:
O 0.12%
F 0.1%
Ne 0.14%
Na 0.14%
Mg 0.26%
Al 0.19%
Si 0.82%
$^{56}$Fe + H → $^{34}$S
[Vi07] [We90] [We98a]
Flux impact:
O 0.14%
F 0.12%
Ne 0.17%
Na 0.16%
Mg 0.34%
Al 0.22%
Si 0.92%
$^{56}$Fe + H → $^{34}$Cl*
[Vi07] [Ti11] [We90] [We98a] [Ti08]
Flux impact:
Si 0.12%
$^{56}$Fe + H → $^{35}$S*
[Vi07] [We90] [We98a]
Flux impact:
Mg 0.17%
Al 0.12%
Si 0.46%
$^{56}$Fe + H → $^{35}$Cl
[Vi07] [We90] [We98a]
Flux impact:
Mg 0.13%
Si 0.34%
$^{56}$Fe + H → $^{36}$Ar
[Vi07] [We90] [We98a]
Flux impact:
Si 0.12%
$^{56}$Fe + H → $^{36}$Cl
[Vi07] [We90] [We98a]
Flux impact:
O 0.13%
F 0.1%
Ne 0.15%
Na 0.14%
Mg 0.29%
Al 0.21%
Si 0.78%
$^{56}$Fe + H → $^{37}$Cl
[Vi07] [We90] [We98a]
Flux impact:
Si 0.24%
$^{56}$Fe + H → $^{37}$Ar
[Vi07] [We90] [We98a]
Flux impact:
Mg 0.15%
Al 0.11%
Si 0.4%
GP12up22
GP12
GP22
$\sigma$ [mb]
$E_{k/n}$ [GeV/n]

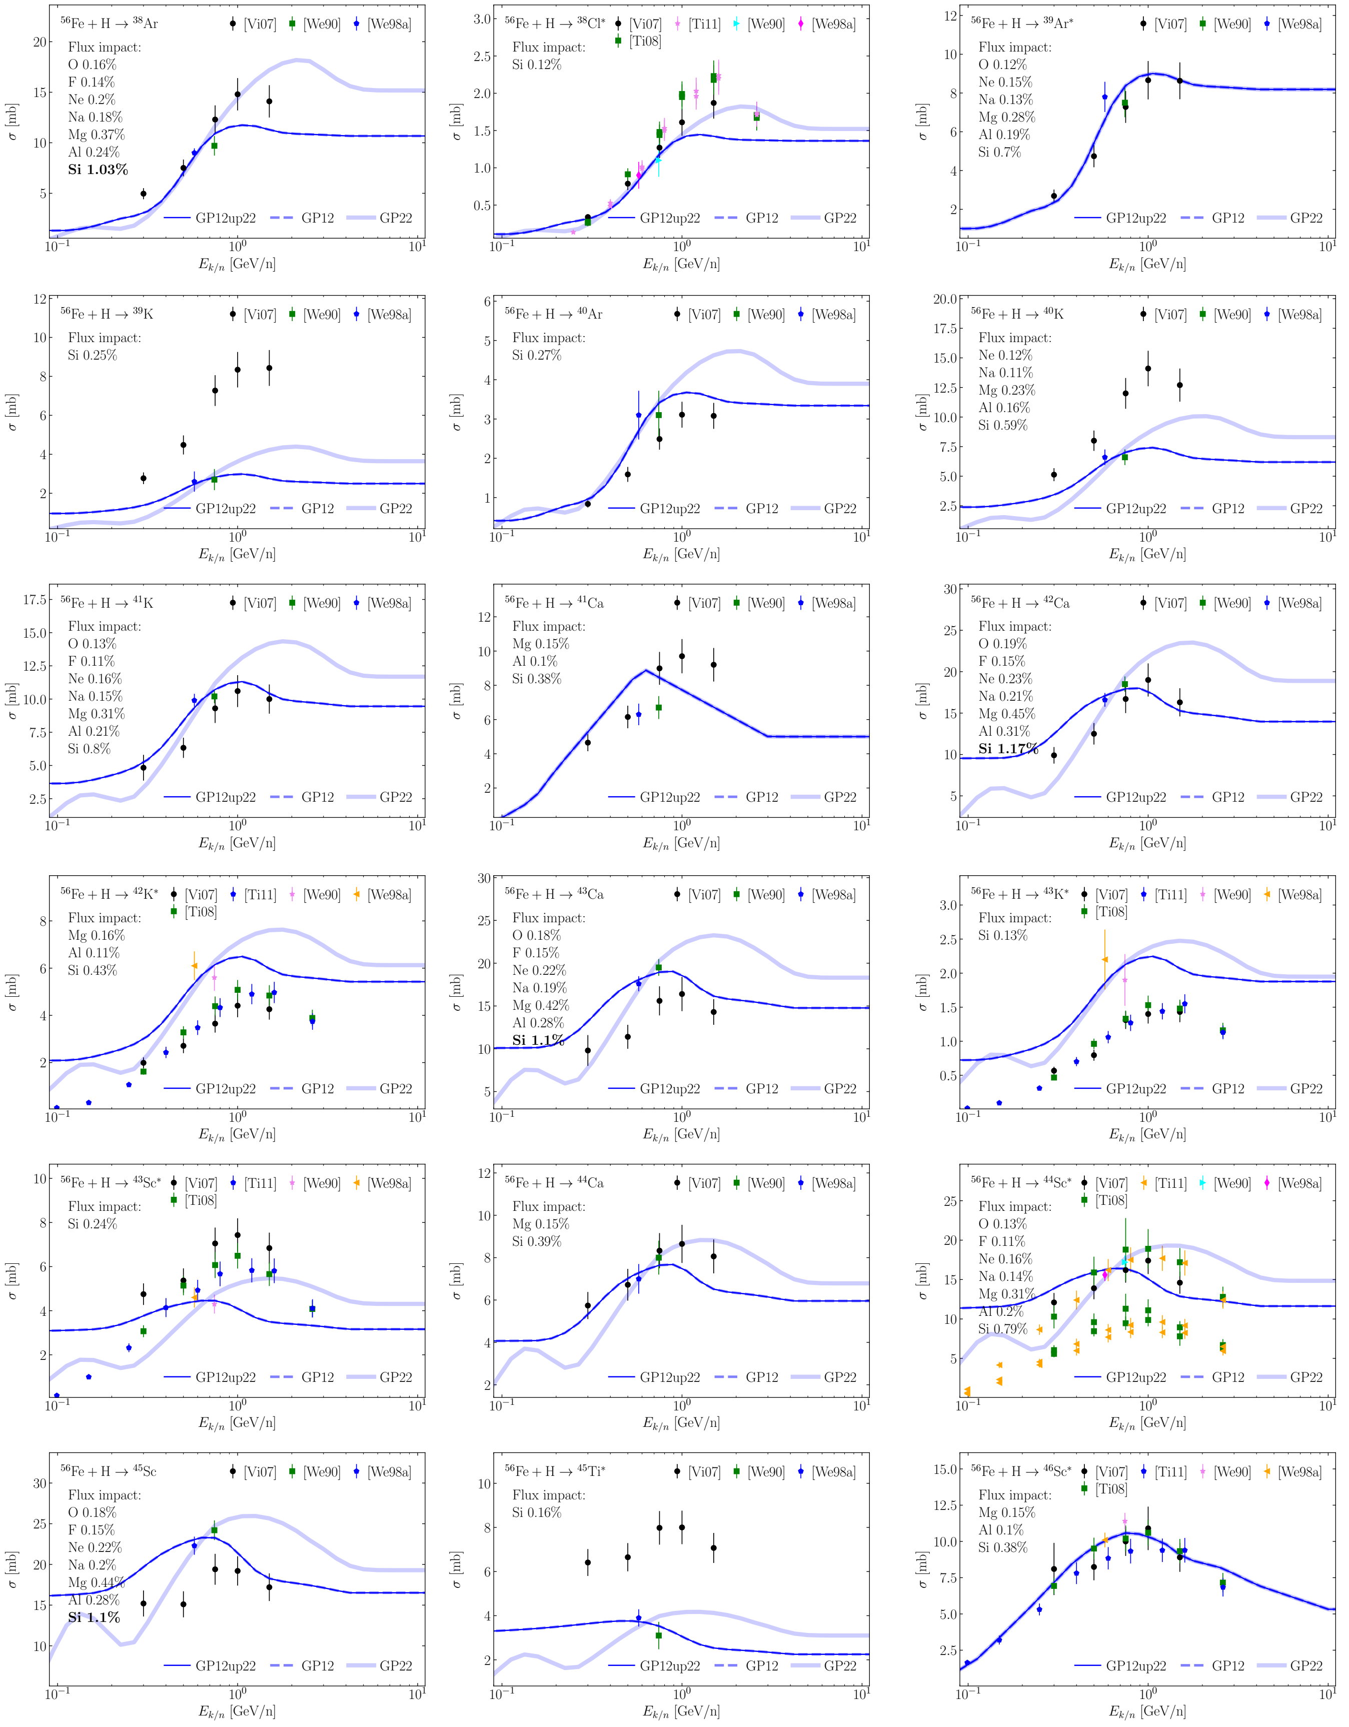
$^{56}$Fe + H → $^{38}$Ar
[Vi07] [We90] [We98a]
Flux impact:
O 0.16%
F 0.14%
Ne 0.2%
Na 0.18%
Mg 0.37%
Al 0.24%
Si 1.03%
$^{56}$Fe + H → $^{38}$Cl*
[Vi07] [Ti11] [We90] [We98a] [Ti08]
Flux impact:
Si 0.12%
$^{56}$Fe + H → $^{39}$Ar*
[Vi07] [We90] [We98a]
Flux impact:
O 0.12%
Ne 0.15%
Na 0.13%
Mg 0.28%
Al 0.19%
Si 0.7%
$^{56}$Fe + H → $^{39}$K
[Vi07] [We90] [We98a]
Flux impact:
Si 0.25%
$^{56}$Fe + H → $^{40}$Ar
[Vi07] [We90] [We98a]
Flux impact:
Si 0.27%
$^{56}$Fe + H → $^{40}$K
[Vi07] [We90] [We98a]
Flux impact:
Ne 0.12%
Na 0.11%
Mg 0.23%
Al 0.16%
Si 0.59%
$^{56}$Fe + H → $^{41}$K
[Vi07] [We90] [We98a]
Flux impact:
O 0.13%
F 0.11%
Ne 0.16%
Na 0.15%
Mg 0.31%
Al 0.21%
Si 0.8%
$^{56}$Fe + H → $^{41}$Ca
[Vi07] [We90] [We98a]
Flux impact:
Mg 0.15%
Al 0.1%
Si 0.38%
$^{56}$Fe + H → $^{42}$Ca
[Vi07] [We90] [We98a]
Flux impact:
O 0.19%
F 0.15%
Ne 0.23%
Na 0.21%
Mg 0.45%
Al 0.31%
Si 1.17%
$^{56}$Fe + H → $^{42}$K*
[Vi07] [Ti11] [We90] [We98a] [Ti08]
Flux impact:
Mg 0.16%
Al 0.11%
Si 0.43%
$^{56}$Fe + H → $^{43}$Ca
[Vi07] [We90] [We98a]
Flux impact:
O 0.18%
F 0.15%
Ne 0.22%
Na 0.19%
Mg 0.42%
Al 0.28%
Si 1.1%
$^{56}$Fe + H → $^{43}$K*
[Vi07] [Ti11] [We90] [We98a] [Ti08]
Flux impact:
Si 0.13%
$^{56}$Fe + H → $^{43}$Sc*
[Vi07] [Ti11] [We90] [We98a] [Ti08]
Flux impact:
Si 0.24%
$^{56}$Fe + H → $^{44}$Ca
[Vi07] [We90] [We98a]
Flux impact:
Mg 0.15%
Si 0.39%
$^{56}$Fe + H → $^{44}$Sc*
[Vi07] [Ti11] [We90] [We98a] [Ti08]
Flux impact:
O 0.13%
F 0.11%
Ne 0.16%
Na 0.14%
Mg 0.31%
Al 0.2%
Si 0.79%
$^{56}$Fe + H → $^{45}$Sc
[Vi07] [We90] [We98a]
Flux impact:
O 0.18%
F 0.15%
Ne 0.22%
Na 0.2%
Mg 0.44%
Al 0.28%
Si 1.1%
$^{56}$Fe + H → $^{45}$Ti*
[Vi07] [We90] [We98a]
Flux impact:
Si 0.16%
$^{56}$Fe + H → $^{46}$Sc*
[Vi07] [Ti11] [We90] [We98a] [Ti08]
Flux impact:
Mg 0.15%
Al 0.1%
Si 0.38%
GP12up22 GP12 GP22
σ [mb]
$E_{k/n}$ [GeV/n]

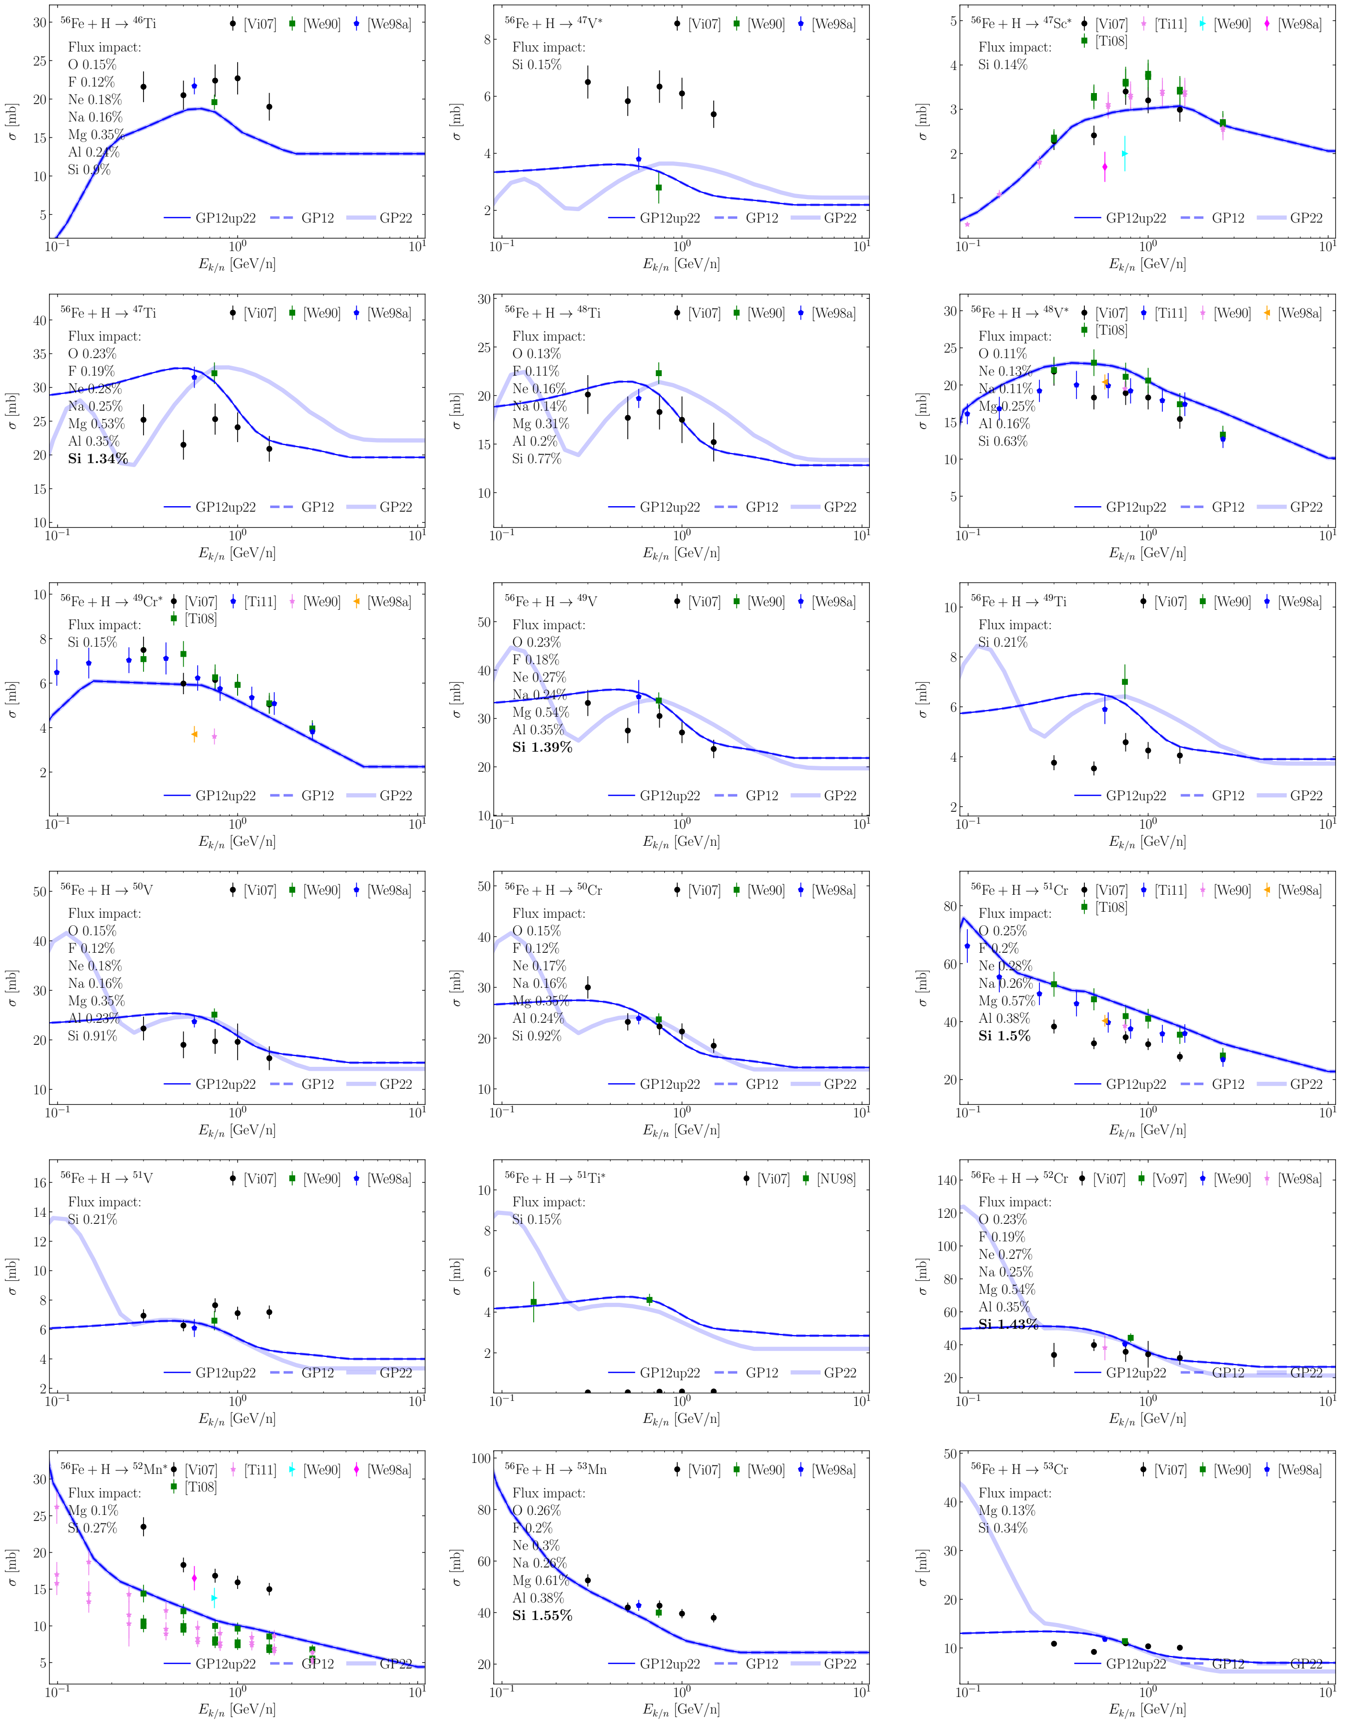
$^{56}$Fe + H → $^{46}$Ti
[Vi07] [We90] [We98a]
Flux impact:
O 0.15%
F 0.12%
Ne 0.18%
Na 0.16%
Mg 0.35%
Al 0.24%
Si 0.9%
GP12up22 GP12 GP22
$^{56}$Fe + H → $^{47}$V*
[Vi07] [We90] [We98a]
Flux impact:
Si 0.15%
GP12up22 GP12 GP22
$^{56}$Fe + H → $^{47}$Sc*
[Vi07] [Ti11] [We90] [We98a] [Ti08]
Flux impact:
Si 0.14%
GP12up22 GP12 GP22
$^{56}$Fe + H → $^{47}$Ti
[Vi07] [We90] [We98a]
Flux impact:
O 0.23%
F 0.19%
Ne 0.28%
Na 0.25%
Mg 0.53%
Al 0.35%
**Si 1.34%**
GP12up22 GP12 GP22
$^{56}$Fe + H → $^{48}$Ti
[Vi07] [We90] [We98a]
Flux impact:
O 0.13%
F 0.11%
Ne 0.16%
Na 0.14%
Mg 0.31%
Al 0.2%
Si 0.77%
GP12up22 GP12 GP22
$^{56}$Fe + H → $^{48}$V*
[Vi07] [Ti11] [We90] [We98a] [Ti08]
Flux impact:
O 0.11%
Ne 0.13%
Na 0.11%
Mg 0.25%
Al 0.16%
Si 0.63%
GP12up22 GP12 GP22
$^{56}$Fe + H → $^{49}$Cr*
[Vi07] [Ti11] [We90] [We98a] [Ti08]
Flux impact:
Si 0.15%
GP12up22 GP12 GP22
$^{56}$Fe + H → $^{49}$V
[Vi07] [We90] [We98a]
Flux impact:
O 0.23%
F 0.18%
Ne 0.27%
Na 0.24%
Mg 0.54%
Al 0.35%
**Si 1.39%**
GP12up22 GP12 GP22
$^{56}$Fe + H → $^{49}$Ti
[Vi07] [We90] [We98a]
Flux impact:
Si 0.21%
GP12up22 GP12 GP22
$^{56}$Fe + H → $^{50}$V
[Vi07] [We90] [We98a]
Flux impact:
O 0.15%
F 0.12%
Ne 0.18%
Na 0.16%
Mg 0.35%
Al 0.23%
Si 0.91%
GP12up22 GP12 GP22
$^{56}$Fe + H → $^{50}$Cr
[Vi07] [We90] [We98a]
Flux impact:
O 0.15%
F 0.12%
Ne 0.17%
Na 0.16%
Mg 0.35%
Al 0.24%
Si 0.92%
GP12up22 GP12 GP22
$^{56}$Fe + H → $^{51}$Cr
[Vi07] [Ti11] [We90] [We98a] [Ti08]
Flux impact:
O 0.25%
F 0.2%
Ne 0.28%
Na 0.26%
Mg 0.57%
Al 0.38%
**Si 1.5%**
GP12up22 GP12 GP22
$^{56}$Fe + H → $^{51}$V
[Vi07] [We90] [We98a]
Flux impact:
Si 0.21%
GP12up22 GP12 GP22
$^{56}$Fe + H → $^{51}$Ti*
[Vi07] [NU98]
Flux impact:
Si 0.15%
GP12up22 GP12 GP22
$^{56}$Fe + H → $^{52}$Cr
[Vi07] [Vo97] [We90] [We98a]
Flux impact:
O 0.23%
F 0.19%
Ne 0.27%
Na 0.25%
Mg 0.54%
Al 0.35%
**Si 1.43%**
GP12up22 GP12 GP22
$^{56}$Fe + H → $^{52}$Mn*
[Vi07] [Ti11] [We90] [We98a] [Ti08]
Flux impact:
Mg 0.1%
Si 0.27%
GP12up22 GP12 GP22
$^{56}$Fe + H → $^{53}$Mn
[Vi07] [We90] [We98a]
Flux impact:
O 0.26%
F 0.2%
Ne 0.3%
Na 0.26%
Mg 0.61%
Al 0.38%
**Si 1.55%**
GP12up22 GP12 GP22
$^{56}$Fe + H → $^{53}$Cr
[Vi07] [We90] [We98a]
Flux impact:
Mg 0.13%
Si 0.34%
GP12up22 GP12 GP22
σ [mb]
$E_{k/n}$ [GeV/n]

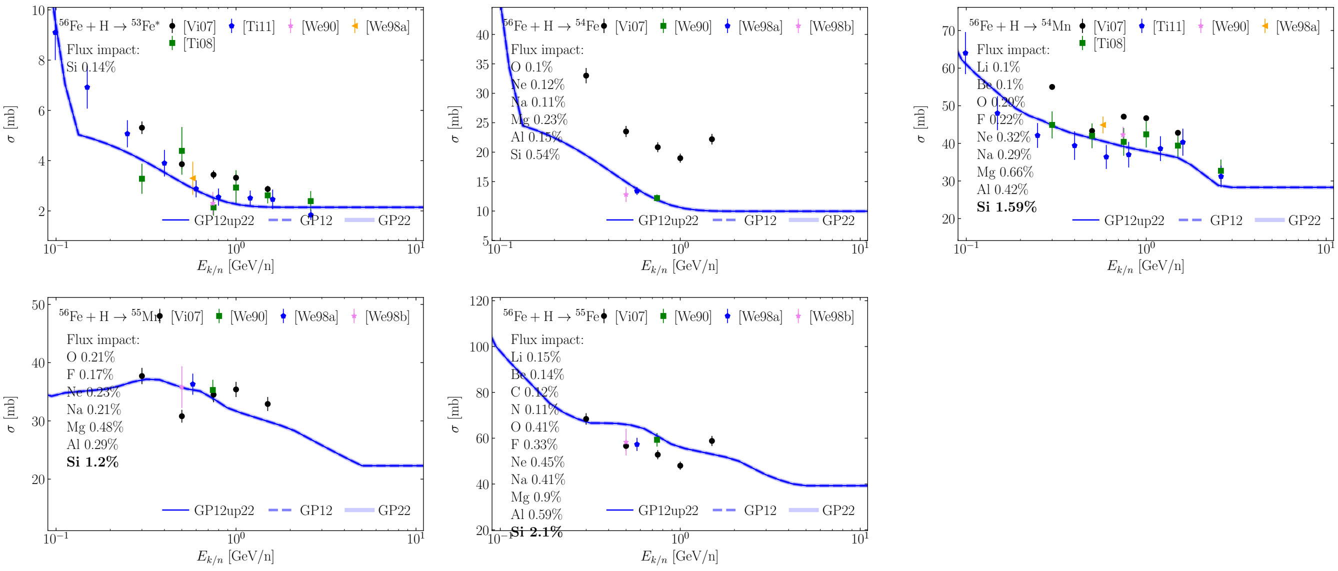

56Fe + H → 53Fe*
[Vi07] [Ti11] [We90] [We98a] [Ti08]
Flux impact:
Si 0.14%
GP12up22 GP12 GP22
σ [mb]
E k/n [GeV/n]
56Fe + H → 54Fe
[Vi07] [We90] [We98a] [We98b]
Flux impact:
O 0.1%
Ne 0.12%
Na 0.11%
Mg 0.23%
Al 0.15%
Si 0.54%
56Fe + H → 54Mn
[Vi07] [Ti11] [We90] [We98a] [Ti08]
Flux impact:
Li 0.1%
Be 0.1%
O 0.29%
F 0.22%
Ne 0.32%
Na 0.29%
Mg 0.66%
Al 0.42%
Si 1.59%
56Fe + H → 55Mn
[Vi07] [We90] [We98a] [We98b]
Flux impact:
O 0.21%
F 0.17%
Ne 0.23%
Na 0.21%
Mg 0.48%
Al 0.29%
Si 1.2%
56Fe + H → 55Fe
[Vi07] [We90] [We98a] [We98b]
Flux impact:
Li 0.15%
Be 0.14%
C 0.12%
N 0.11%
O 0.41%
F 0.33%
Ne 0.45%
Na 0.41%
Mg 0.9%
Al 0.59%
Si 2.1%

[1] A. Reinert and M. W. Winkler, J. Cosmology Astropart. Phys. **1**, 055 (2018), arXiv:1712.00002 [astro-ph.HE].
[2] D. Maurin, E. Ferronato Bueno, Y. Génolini, L. Derome, and M. Vecchi, A&A **668**, A7 (2022), arXiv:2203.00522 [astro-ph.HE].
[3] R. Ramaty, B. Kozlovsky, R. E. Lingenfelter, and H. Reeves, ApJ **488**, 730 (1997), astro-ph/9610255.
[4] M. Epherre, E. Gradsztajn, R. Klapisch, and H. Reeves, Nucl. Phys. A **139**, 545 (1969).
[5] P. Fontes, Phys. Rev. C **15**, 2159 (1977).
[6] J. R. Radin, E. Gradsztajn, and A. R. Smith, Phys. Rev. C **20**, 787 (1979).
[7] D. L. Olson, B. L. Berman, D. E. Greiner, H. H. Heckman, P. J. Lindstrom, and H. J. Crawford, Phys. Rev. C **28**, 1602 (1983).
[8] R. Silberberg, C. H. Tsao, and A. F. Barghouty, ApJ **501**, 911 (1998).
[9] A. Korejwo, ICRC **4**, 267 (1999).
[10] A. Korejwo, M. Giller, T. Dzikowski, V. Perelygin, and A. Zarubin, Journal of Physics G: Nuclear and Particle Physics **28**, 1199 (2002).
[11] S. M. Read and V. E. Viola, Jr., Atomic Data and Nuclear Data Tables **31**, 359 (1984).
[12] NUCLEX database: (i) A. S. Iljinov, V. G. Semenov, M. P. Semenova, N. M. Sobolevsky, and L. V. Udovenko, Springer Verlag, Landolt-Börnstein, New Series, subvolumes I/13a (1991), I/13b (1992), I/13c (1993), I/13d (1994), I/13e (1994), I/13f (1995), I/13h (1996), I/13h (1996); (ii) V. I. Ivanov, N. M. Sobolevsky, and V. G. Semenov, NUCLEX: an IBM PC Version of Handbook on Radionuclide Production Cross Section at Intermediate Energies, Proc. Specialists Mtg., Issy-les-Moulineaux, France, May 30–June 1, 1994, OECD, p. 387; (iii) Computer Version Of the Handbook on Radionuclide Production Cross-Sections at Intermediate Energies (the NUCLEX Code), Proc. 3d Specialists Meeting on Shielding Aspects of Accelerators, Targets and Irradiation Facilities (SATIF-3), Tohoku University, Sendai, Japan, May 12-13, 1997, NEA/OECD (1998) p. 277.; (iii) see also in https://cds.cern.ch/record/375269/files/9812071.pdf.
[13] R. Michel, M. Gloris, H.-J. Lange, I. Leya, M. Lüpke, U. Herpers, B. Dittrich-Hannen, R. Rösel, T. Schiekel, D. Filges, P. Dragovitsch, M. Suter, H.-J. Hofmann, W. Wölfli, P. W. Kubik, H. Baur, and R. Wieler, Nucl. Instr. Meth. Phys. Res. B **103**, 183 (1995).
[14] T. Schiekel, F. Sudbrock, U. Herpers, M. Gloris, H.-J. Lange, I. Leya, R. Michel, B. Dittrich-Hannen, H.-A. Synal, M. Suter, P. W. Kubik, M. Blann, and D. Filges, Nucl. Instr. Meth. Phys. Res. B **114**, 91 (1996).
[15] W. R. Webber, AIP Conference Proceedings **203**, 294 (1990), http://aip.scitation.org/doi/pdf/10.1063/1.39166.
[16] W. R. Webber, J. C. Kish, and D. A. Schrier, Phys. Rev. C **41**, 547 (1990).
[17] Transport Collaboration, C.-X. Chen, S. Albergo, *et al.*, ApJ **479**, 504 (1997).
[18] Transport Collaboration, C. N. Knott, S. Albergo, *et al.*, Phys. Rev. C **56**, 398 (1997).
[19] Transport Collaboration, C.-X. Chen, S. Albergo, *et al.*, Phys. Rev. C **56**, 1536 (1997).
[20] W. R. Webber, J. C. Kish, J. M. Rockstroh, Y. Cassagnou, R. Legrain, A. Soutoul, O. Testard, and C. Tull, ApJ **508**, 949 (1998).
[21] W. R. Webber, A. Soutoul, J. C. Kish, J. M. Rockstroh, Y. Cassagnou, R. Legrain, and O. Testard, Phys. Rev. C **58**, 3539 (1998).
[22] C. M. Bäcker, C. Bäumer, M. Gerhardt, K. Kröninger, C. Nitsch, H. M. Siregar, B. Timmermann, N. Verbeek, J. Weingarten, J. Wulff, and A. Yazgan, Nucl. Instrum. Methods Phys. Res. B **454**, 50 (2019).
[23] Y. E. Titarenko, V. F. Batyaev, A. Y. Titarenko, M. A. Butko, K. V. Pavlov, S. N. Florya, R. S. Tikhonov, V. M. Zhivun, A. V. Ignatyuk, S. G. Mashnik, S. Leray, A. Boudard, J. Cugnon, D. Mancusi, Y. Yariv, K. Nishihara, N. Matsuda, H. Kumawat, G. Mank, and W. Gudowski, Physics of Atomic Nuclei **74**, 523 (2011).
[24] Y. E. Titarenko, V. F. Batyaev, A. Y. Titarenko, M. A. Butko, K. V. Pavlov, S. N. Florya, R. S. Tikhonov, S. G. Mashnik, A. V. Ignatyuk, N. N. Titarenko, W. Gudowski, M. Těšínský, C.-M. L. Persson, H. A. Abderrahim, H. Kumawat, and H. Duarte, Phys. Rev. C **78**, 034615 (2008), arXiv:0804.1260 [nucl-ex].
[25] C.-M. Herbach, D. Hilscher, U. Jahnke, V. G. Tishchenko, J. Galin, A. Letourneau, A. Péghaire, D. Filges, F. Goldenbaum, L. Pienkowski, W. U. Schröder, and J. Tõke, Nucl. Instrum. Methods Phys. Res. A **562**, 729 (2006).
[26] É. K. Bazarov, V. V. Glagolev, V. V. Lugovoy, S. L. Lutpullaev, K. Olimov, V. I. Petrov, A. A. Yuldashev, and B. S. Yuldashev, Soviet Journal of Experimental and Theoretical Physics Letters **81**, 140 (2005).
[27] P. Napolitani, K. H. Schmidt, A. S. Botvina, F. Rejmund, L. Tassan-Got, and C. Villagrasa, Phys. Rev. C **70**, 054607 (2004).
[28] K. Kettern, Y. Shubin, G. Steyn, T. van der Walt, H. Coenen, and S. Qaim, Applied Radiation and Isotopes **60**, 939 (2004).
[29] H. Yashima, Y. Uwamino, H. Iwase, H. Sugita, T. Nakamura, S. Ito, and A. Fukumura, Nucl. Instrum. Methods Phys. Res. B **226**, 243 (2004).
[30] K. J. Kim, J. M. Sisterson, P. A. J. Englert, M. W. Caffee, R. C. Reedy, J. Vincent, and C. Castaneda, Nucl. Instr. Meth. Phys. Res. B **196**, 239 (2002).
[31] M. Faßbender, B. Schölten, and S. M. Qaim, Radiochimica Acta **81**, 1 (1998).
[32] J. M. Sisterson, K. Kim, A. Beverding, P. A. J. Englert, M. Caffee, A. J. T. Jull, D. J. Donahue, L. McHargue, C. Castaneda, J. Vincent, and R. C. Reedy, Nucl. Instr. Meth. Phys. Res. B **123**, 324 (1997).
[33] R. Michel, R. Bodemann, H. Busemann, R. Daunke, M. Gloris, H.-J. Lange, B. Klug, A. Krins, I. Leya, M. Lüpke, S. Neumann, H. Reinhardt, M. Schnatz-Büttgen, U. Herpers, T. Schiekel, F. Sudbrock, B. Holmqvist, H. Condé, P. Malmborg,

M. Suter, B. Dittrich-Hannen, P.-W. Kubik, H.-A. Synal, and D. Filges, Nucl. Instr. Meth. Phys. Res. B **129**, 153 (1997).
[34] I. Leya, H. J. Lange, and R. Michel, Meteoritics and Planetary Science Supplement **32**, A78 (1997).
[35] M. Faßbender, B. Scholten, Y. N. Shubin, and S. Qaim, in *Conference proceedings: Italian Physical Society*, Vol. 59 (Editrice Compositori, 1997) pp. 1646–1648.
[36] S. Shibata, M. Imamura, H. Nagai, K. Kobayashi, K. Sakamoto, M. Furukawa, and I. Fujiwara, Phys. Rev. C **48**, 2617 (1993).
[37] J. M. Sisterson, A. M. Koehler, A. J. T. Jull, D. J. Donahue, L. McHargue, R. C. Reedy, and P. A. J. Englert, in *Lunar and Planetary Science Conference*, Vol. 23 (1992).
[38] W. R. Webber, J. C. Kish, and D. A. Schrier, Phys. Rev. C **41**, 566 (1990).
[39] P. Kozma, K. D. Tolstov, and V. V. Yanovsky, Nucl. Instrum. Methods Phys. Res. A **291**, 662 (1990).
[40] B. Dittrich, U. Herpers, H. J. Hofmann, W. Wölfli, R. Bodemann, M. Lüpke, R. Michel, P. Dragovitsch, and D. Filges, Nucl. Instr. Meth. Phys. Res. B **52**, 588 (1990).
[41] B. Dittrich, U. Herpers, M. Lupke, R. Michel, H. J. Hofmann, and W. Wolfli, Radiochim.Acta **50**, 11 (1990).
[42] V. Aleksandrov, M. Semenova, and V. Semenov, Vopr. Atomn. Nauki i Tekhn., Ser. Yad. Fiz. Issledo **8**, 16 (1990).
[43] R. Michel, B. Dittrich, U. Herpers, F. Peiffer, T. Schiffmann, P. Cloth, P. Dragovitsch, and D. Filges, The Analyst **114**, 287 (1989).
[44] R. Michel, P. Dragovitsch, P. Englert, F. Peiffer, R. Stück, S. Theis, F. Begemann, H. Weber, P. Signer, R. Wieler, D. Filges, and P. Cloth, Nuclear Instruments and Methods in Physics Research B **16**, 61 (1986).
[45] J. L. Reyss, Y. Yokoyama, and F. Guichard, Earth and Planetary Science Letters **53**, 203 (1981).
[46] G. M. Raisbeck and F. Yiou, in *ICRC 15*, Vol. 2 (1977) p. 203.
[47] P. Fontes, Phys. Rev. C **15**, 2159 (1977).
[48] S. B. Kaufman, M. W. Weisfield, B. D. Wilkins, D. Henderson, and E. P. Steinberg, Phys. Rev. C **13**, 253 (1976).
[49] T. Inoue and S. Tanaka, Journal of Inorganic and Nuclear Chemistry **38**, 1425 (1976).
[50] K. R. Hogstrom, Phys. Rev. C **14**, 753 (1976).
[51] H. R. Heydegger, A. L. Turkevich, A. van Ginneken, and P. H. Walpole, Phys. Rev. C **14**, 1506 (1976).
[52] S. Regnier, P. Paillard, and G. Simonoff, Academie des Sciences Paris Comptes Rendus Serie B Sciences Physiques **280**, 513 (1975).
[53] G. M. Raisbeck and F. Yiou, Phys. Rev. C **12**, 915 (1975).
[54] G. M. Raisbeck, J. Lestringuez, and F. Yiou, Physics Letters B **57**, 186 (1975).
[55] G. M. Raisbeck and F. Yiou, Phys. Rev. C **9**, 1385 (1974).
[56] G. M. Raisbeck, J. Lestringuez, and F. Yiou, Phys. Rev. C **6**, 685 (1972).
[57] G. W. Butler, S. B. Kaufman, E. P. Steinberg, and B. D. Wilkins, Phys. Rev. C **6**, 1153 (1972).
[58] B. S. Amin, S. Biswas, D. Lal, and B. L. K. Somayajulu, Nucl. Phys. A **195**, 311 (1972).
[59] G. B. Stapleton and R. H. Thomas, Nucl. Phys. A **175**, 124 (1971).
[60] G. M. Raisbeck and F. Yiou, Phys. Rev. Lett. **27**, 875 (1971).
[61] P. Fontes, C. Perron, J. Lestringuez, F. Yiou, and R. Bernas, Nucl. Phys. A **165**, 405 (1971).
[62] R. Bimbot and H. Gauvin, Comptes rendus hebdomadaires des séances de l'académie des sciences, série B **273**, 1054 (1971).
[63] M. Barbier and S. Régnier, Journal of Inorganic and Nuclear Chemistry **33**, 2720 (1971).
[64] A. F. Stehney and E. P. Steinberg, Nuclear Physics B **5**, 188 (1968).
[65] G. V. Rayudu, Journal of Inorganic and Nuclear Chemistry **30**, 2311 (1968).
[66] I. Dostrovsky, H. Gauvin, and M. Lefort, Physical Review **169**, 836 (1968).
[67] P. Andrews, P. Butler, A. Christy, A. James, P. Kirkby, B. Lowe, and B. Renwick, Nuclear Physics A **109**, 689 (1968).
[68] I. R. Williams and C. B. Fulmer, Phys. Rev. **154**, 1005 (1967).
[69] D. F. Measday, Nuclear Physics **78**, 476 (1966).
[70] H. Gauvin, Compt.Rend. **263B**, 752 (1966).
[71] L. Valentin, Nuclear Physics **62**, 81 (1965).
[72] P. Reeder, Journal of Inorganic and Nuclear Chemistry **27**, 1879 (1965).
[73] I. Dostrovsky, R. Davis, A. M. Poskanzer, and P. L. Reeder, Physical Review **139**, 1513 (1965).
[74] R. Bernas, M. Epherre, E. Gradsztajn, R. Klapisch, and F. Yiou, Physics Letters **15**, 147 (1965).
[75] S. Warshaw, R. Swanson, and A. Rosenfeld, in *PHYSICAL REVIEW*, Vol. 95 (American Physical Society Physics Ellipse, College PK, MD 20740-3844 USA, 1954) pp. 649–649.
[76] G. V. S. Rayudu, Canadian Journal of Chemistry **42**, 1149 (1964).
[77] A. M. Poskanzer, L. P. Remsberg, S. Katcoff, and J. B. Cumming, Physical Review **133**, B1507 (1964).
[78] M. Honda and D. Lal, Nuclear Physics **51**, 363 (1964).
[79] L. Valentin, G. Albouy, J. P. Cohen, and M. Gusakow, Physics Letters **7**, 163 (1963).
[80] A. K. Lavrukhina, L. P. Moskaleva, V. V. Malyshev, and L. M. Satarova, Soviet Journal of Experimental and Theoretical Physics **16**, 1 (1963).
[81] H. Gauvin, M. Lefort, and X. Tarrago, Nuclear Physics **39**, 447 (1962).
[82] K. J. Foley, G. L. Salmon, and A. B. Clegg, Nuclear Physics **31**, 43 (1962).
[83] J. B. Cumming, G. Friedlander, J. Hudis, and A. M. Poskanzer, Physical Review **127**, 950 (1962).
[84] C. Brun, M. Lefort, and X. Tarrago, Journal de Physique et le Radium **23**, 371 (1962).
[85] M. Lefort, G. N. Simonoff, and X. Tarrago, Nuclear Physics **25**, 216 (1961).
[86] A. B. Clegg, K. J. Foley, G. L. Salmon, and R. E. Segel, Proceedings of the Physical Society **78**, 681 (1961).

[87] V. Parikh, Nuclear Physics **18**, 646 (1960).
[88] M. Honda and D. Lal, Physical Review **118**, 1618 (1960).
[89] P. A. Benioff, Physical Review **119**, 316 (1960).
[90] E. Baker, G. Friedlander, and J. Hudis, Phys. Rev. **112**, 1319 (1958).
[91] J. L. Symonds, J. Warren, and J. D. Young, Proceedings of the Physical Society. Section A **70**, 824 (1957).
[92] I. D. Prokoshkin and A. Tiapkin, SOVIET PHYSICS JETP-USSR **5**, 148 (1957).
[93] W. E. Burcham, J. L. Symonds, and J. D. Young, Proceedings of the Physical Society. Section A **68**, 1001 (1955).
[94] J. M. Dickson and T. C. Randle, Proceedings of the Physical Society. Section A **64**, 902 (1951).
[95] C. Villagrasa-Canton, A. Boudard, J.-E. Ducret, *et al.*, Phys. Rev. C **75**, 044603 (2007), nucl-ex/0612001.
[96] I. Leya, H. Busemann, H. Baur, R. Wieler, M. Gloris, S. Neumann, R. Michel, F. Sudbrock, and U. Herpers, Nucl. Instr. Meth. Phys. Res. B **145**, 449 (1998).
[97] L. C. Sah, (1960).
[98] R. R. Korteling and A. A. Caretto, Phys. Rev. C **1**, 193 (1970).
[99] J. W. Meadows and R. B. Holt, Physical Review **83**, 47 (1951).
[100] K. Goebel, D. Harting, J. C. Kluyver, A. Kusumegi, and H. Schultes, Nuclear Physics **24**, 28 (1961).
[101] N. M. Hintz and N. F. Ramsey, Physical Review **88**, 19 (1952).
[102] S. B. Kaufman, M. W. Weisfield, E. P. Steinberg, B. D. Wilkins, and D. J. Henderson, Phys. Rev. C **19**, 962 (1979).
[103] L. Marquez, Physical Review **86**, 405 (1952).
[104] L. Moskaleva, G. Fedoseev, and K. AN, SOVIET JOURNAL OF NUCLEAR PHYSICS-USSR **12**, 472 (1971).
[105] C. E. Tull, S. Albergo, Z. Caccia, C. X. Chen, S. Costa, H. J. Crawford, M. Cronqvist, J. Engelage, P. Ferrando, I. Flores, L. Greiner, T. G. Guzik, A. Insolia, F. C. Jones, C. N. Knott, S. Ko, C. Kuo, P. J. Lindstrom, J. Mazotta, J. W. Mitchell, R. Potenza, J. Romanski, G. V. Russo, A. Soutoul, T. J. M. Symons, O. Testard, C. Tuve, C. J. Waddington, W. R. Webber, J. P. Wefel, L. Wu, and X. Zhang, in *23rd International Cosmic Ray Conference (ICRC23), Volume 2*, International Cosmic Ray Conference, Vol. 2 (1993) p. 163.
[106] H. Vonach, A. Pavlik, A. Wallner, M. Drosg, R. C. Haight, D. M. Drake, and S. Chiba, Phys. Rev. C **55**, 2458 (1997).
